# Supplementary material for: Magnetic Distortion Resistant Orientation Estimation
Source: arXiv:2410.12304 source file (2024-10-16)
Supplement: Supplementary file 1 [file Appendix.tex]

\appendix

\vspace{100mm}
\section*{Revision Report}

We thank the reviewers for the constructive comments. 
We revised the paper according to the reviews and make corresponding changes.
As the major differences between this revision and the previous submission, we added more baselines for comparison experiments and more real experiments for evaluation.
Second, we paid a lot of attention on reorganizing the rewriting the paper for better understanding and reading experience.
Third, we thoroughly revised the related work section, in order to better distinguish our work's position relevant to other existing works.
We also added a new design component, the adaptive updating, in the design section, and many other detailed revisions.
In the following part, we present our corresponding revisions to the reviewers' comments. 
Again we thank all reviewers for their insightful reviews.

\section{Reviewer 1 (1AE)}

\subsection{}
\textbf{Original review:} \textit{'discuss a measurable application scenario that the proposed method improves, e.g. demonstrate real-use cases with appropriate applications (AR, VR, etc) to justify the improvement over the state-of-the-art. (R1)'}

\textbf{Corresponding revision:}

First, to demonstrate the direct benefit of orientation improvement, we included an extended case study in the evaluation section (Section~\ref{eval_star}).
We discuss a star sky view application which uses orientation results to render the stars and constellations on smart phones.
Such an application transforms the orientation result into star sky rendering accuracy.
\aliasSystem's overall accuracy of star sky rendering in such application is 86.69$\%$.
As comparison, MUSE has an accuracy of 70.92$\%$.
We also plot the performance of \aliasSystem and MUSE in Figure~\ref{star_2} and Figure~\ref{star_1} (also shown below).
This experiment should justify the improvement of \aliasSystem in a real-use application over the existing work.

\begin{figure} [H]
    % \vspace{-3mm}
    \begin{minipage}[t]{0.35\linewidth}
        % \hspace{-0.1cm}
        \centering
        % \vspace{-2cm}
        \includegraphics[width=1\linewidth]{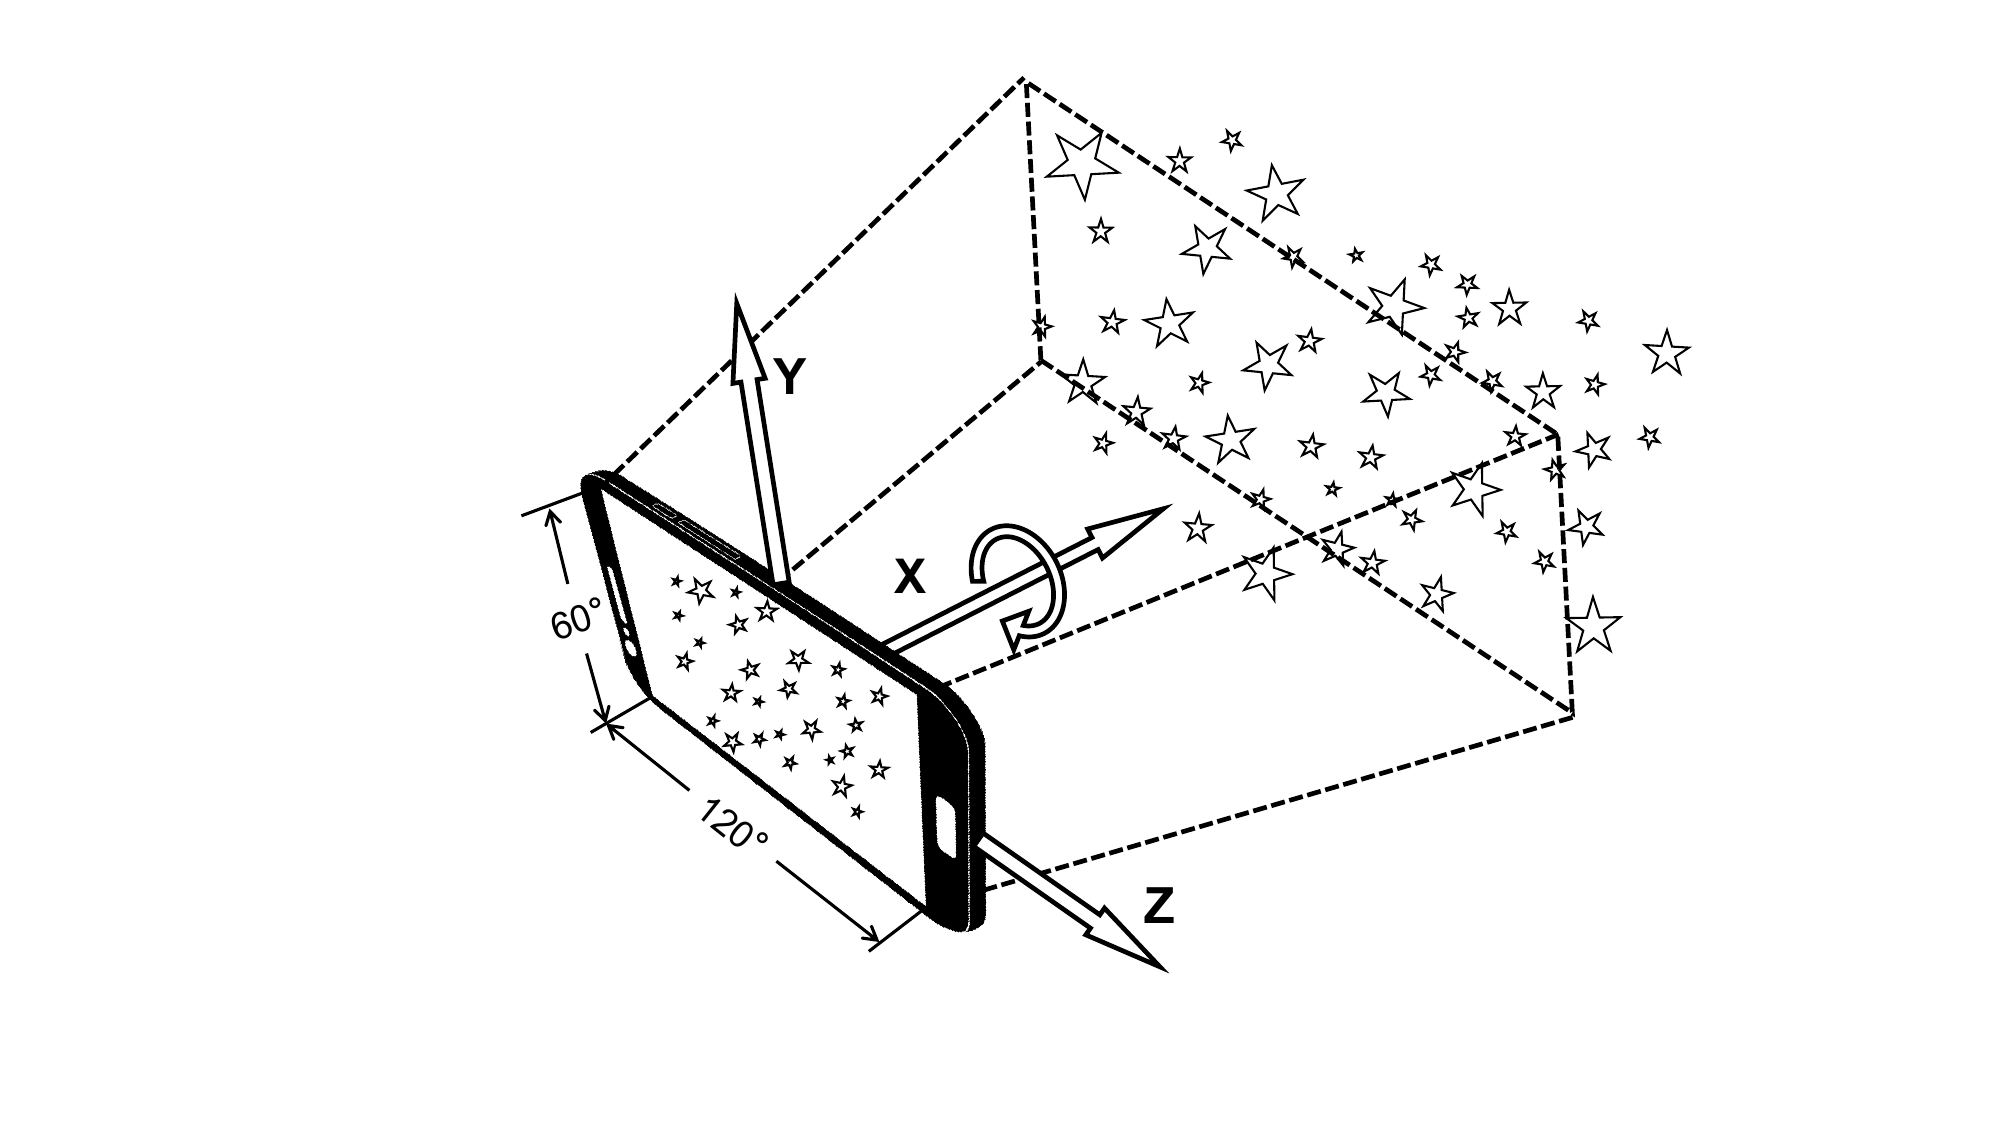}
        \captionsetup{labelformat=empty}
        % \captionsetup{labelformat=empty}
        % \vspace{-7mm}
       \caption{Star sky application.}
        % \label{ubi_star_sky}
    \end{minipage}
    \hfill
    \hfill
    \begin{minipage}[t]{0.27\linewidth}
        % \hspace{-0.1cm}
        \centering
        % % \vspace{-2cm}
        \includegraphics[width=1\linewidth]{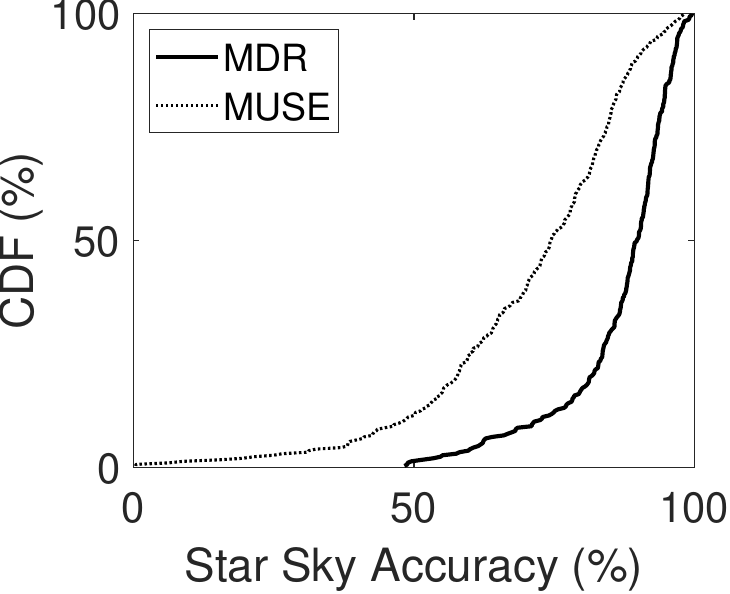}
        \captionsetup{labelformat=empty}
        % \vspace{-7mm}
       \caption{Star sky rendering accuracy CDF.}
        % \label{star_2}
    \end{minipage}
    \hfill
    \begin{minipage}[t]{0.27\linewidth}
        \centering
        % % \vspace{-0.1cm}
        \includegraphics[width=1\linewidth]{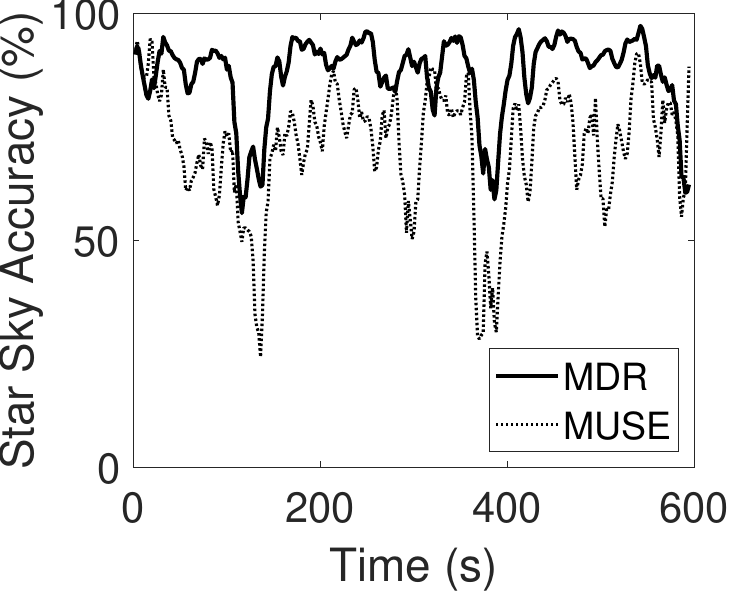}
        \captionsetup{labelformat=empty}
        % \vspace{-7mm}
        \caption{Rendering accuracy over time.}
        % % \vspace{-0.5cm}
        % \label{star_1}
    \end{minipage}
    \hfill
    % \vspace{-4mm}
\end{figure}

Additionally, orientation is commonly used to infer the location of devices, which can support many applications, such as in-air writing, and gesture recognition. 
Better orientation estimation leads to better location estimation.
As a result, \aliasSystem has an average location error of 0.1083m, while MUSE has  an average location error of 0.1364m.
\aliasSystem has 20.60\% lower error than MUSE.

\begin{figure}[H]
    \centering
    \includegraphics[width=0.6\linewidth]{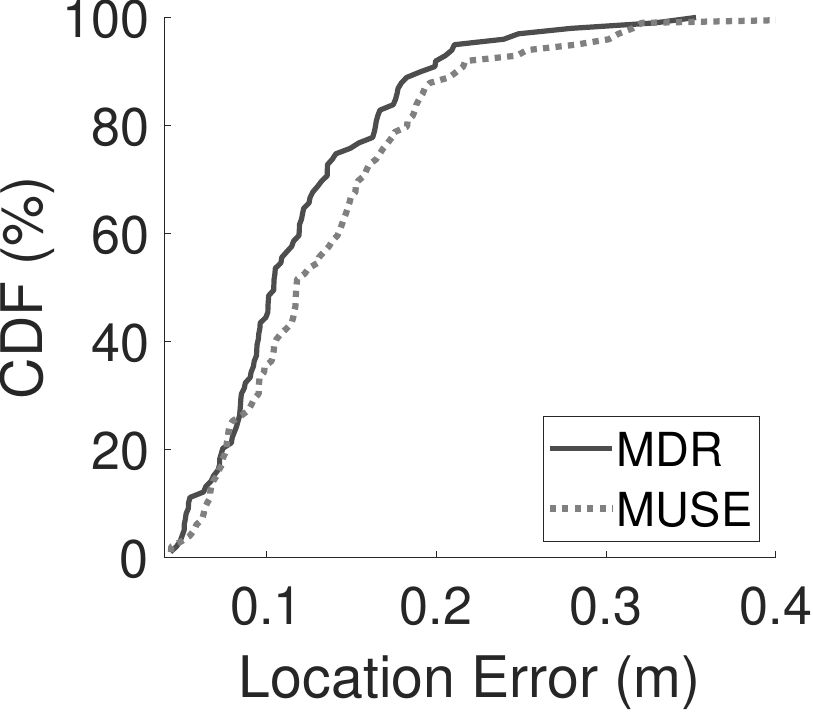}
    \captionsetup{labelformat=empty}
    \caption{Location estimation error}
    % \label{fig:enter-label}
\end{figure}

\subsection{}
\textbf{Original review:} \textit{'clarify analysis of the model (R2)'}

\textbf{Corresponding revision:} 
Reviewer 2 mentioned that \textit{'I suggest users include the correlation graph speed/arm length vs error for the clarity. Fig 23 shows the individual differences, but does not show this important factor. And more systematic analysis will demonstrate the break point of the proposed system that will provide very useful intuition on deployment scenario across varying users.'}.

In this revision, we analyze the performance of the baselines on different users' data in Section~\ref{users}, via look into the accelerometer error in their data, since accelerometer direction error is directly related to orientation estimation error.
High motion speed or intense acceleration maybe cause accelerometer direction error.
% but do not necessarily guarantee it.
Different users may have different error, depending on the user's motion pattern, which mainly affects the accelerometer accuracy.
We take two users as example.
User D's arm moves fast, having an average accelerometer direction error of 16.72°, while user H moves slowly and has an average accelerometer direction error of 7.79°.
As a result, the overall orientation error on user D is higher than user H.
The users evaluation Figure is attached below:

\begin{figure} [H]
    % \hspace{-0.1cm}
    \centering
    % % \vspace{-2cm}
    \includegraphics[width=0.59\linewidth]{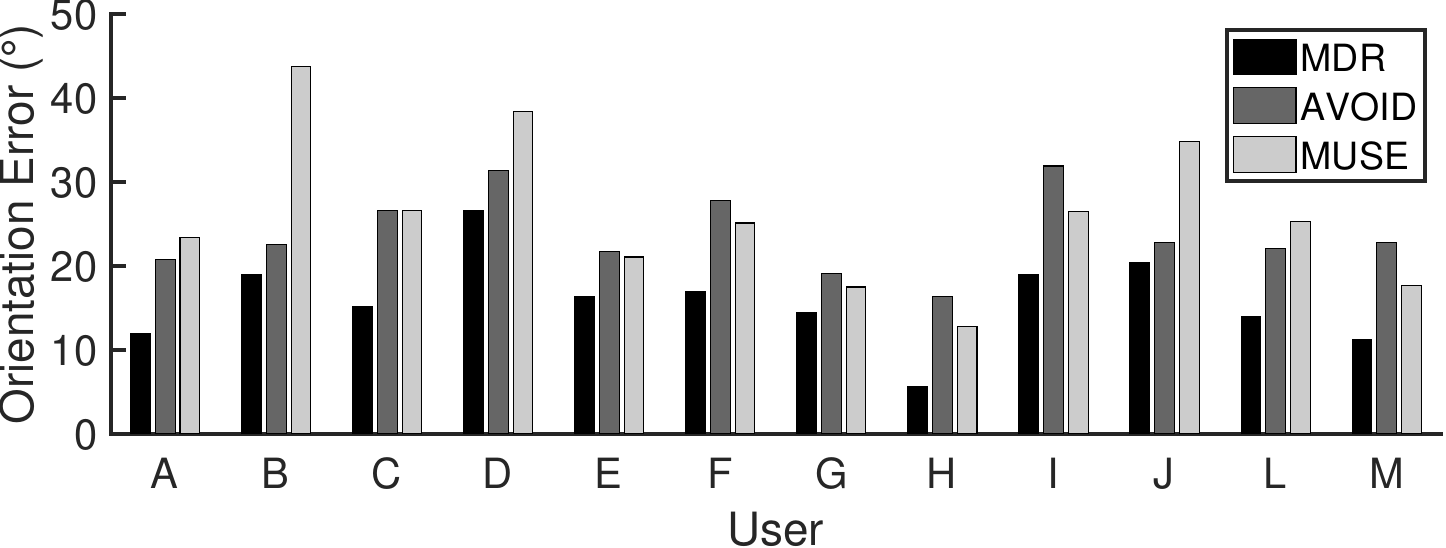}
    % % \vspace{-4mm}
    \captionsetup{labelformat=empty}
    \caption{Performance among different users.}
    % \label{users}
    % % \vspace{-3mm}
\end{figure}

We also plot an extra figure on the relationship between the accelerometer direction error (°) and the final orientation error (°) of \aliasSystem, as shown below:

\begin{figure}[H]
    \centering
    \includegraphics[width=0.3\linewidth] {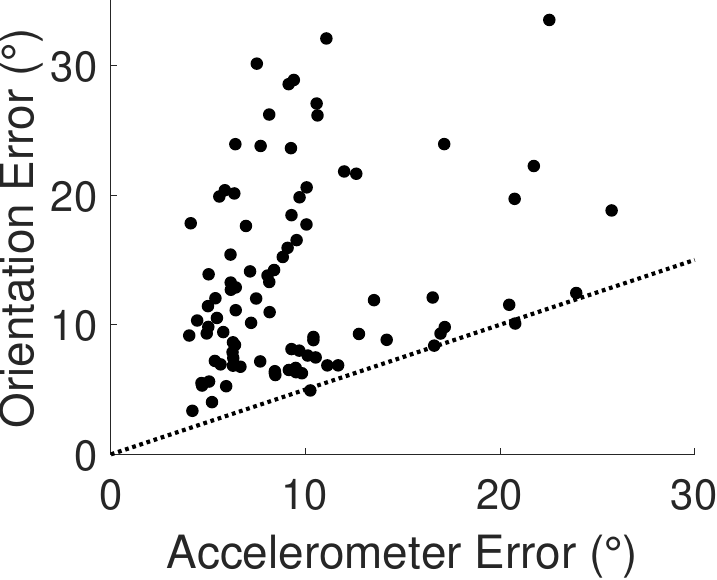}
    \captionsetup{labelformat=empty}
    \caption{Relationship between accelerometer error and orientation error}
    % \label{fig:enter-label}
\end{figure}

Every dot in the figure represents one data trace.
We can see as accelerometer direction increases, the lower bound of the overall error also increases, since the accelerometer direction serves as a direct input of sensor fusion.
However, it is hard to quantify the overall orientation error simply based on accelerometer error, mainly due to the existence of magnetometer error presence.

\subsection{}
\textbf{Original review:} \textit{'better acknowledge prior work, particularly on magnetic distortions (R3)'}

\textbf{Corresponding revision:} 
In this new version, we thoroughly revised Section~\ref{related}: Related Work, and put it earlier in the paper.
Specifically, Section~\ref{related} include three major parts: Magnetic Fingerprint, IMU-based Orientation Estimation, and Magnetic Distortion in Orientation Estimation.

We first discuss the magnetic fingerprinting technique used in localization, as it is closely related with \aliasSystem's magnetic anchor database design.
We justify that the way \aliasSystem uses magnetic anchor database is different from magnetic fingerprint.
Moreover, we discuss that the spatial resolution requirement for magnetic anchor database for orientation estimation is higher than magnetic fingerprint for localization, and based on which, we argue that the database preparation overhead is greater.
That is where the Automatic Updating (Section~\ref{selfDB}) design of \aliasSystem comes in to reduce the overhead of database preparation.

Next, we briefly introduce the related works in IMU-based orientation estimation. 
We identify MUSE~\cite{muse} as the state-of-the-art orientation estimation method, inspired by which, we also adopt a complementary filter for orientation estimation.
We then discuss the current researches that deal with magnetic distortion in orientation estimation (\cite{fan2017adaptive,ahrs}).
We argue that, although they reduce the negative impact of magnetic distortion to a certain extent, they do not fundamentally model the distorted magnetic field. 
Therefore they fail to resist distortion when it is high (verified in Section~\ref{eval_distortion}, with Figure~\ref{result} shown below).
As comparison, \aliasSystem uses a magnetic anchor database to model the magnetic field to resist distortion, and thus has better resistance performance.

\begin{figure}[H]
    % % \vspace{-0.2cm}
    \begin{minipage}[t]{0.5\linewidth}
        \centering
        % % \vspace{-0.1cm}
        \includegraphics[width=1\linewidth]{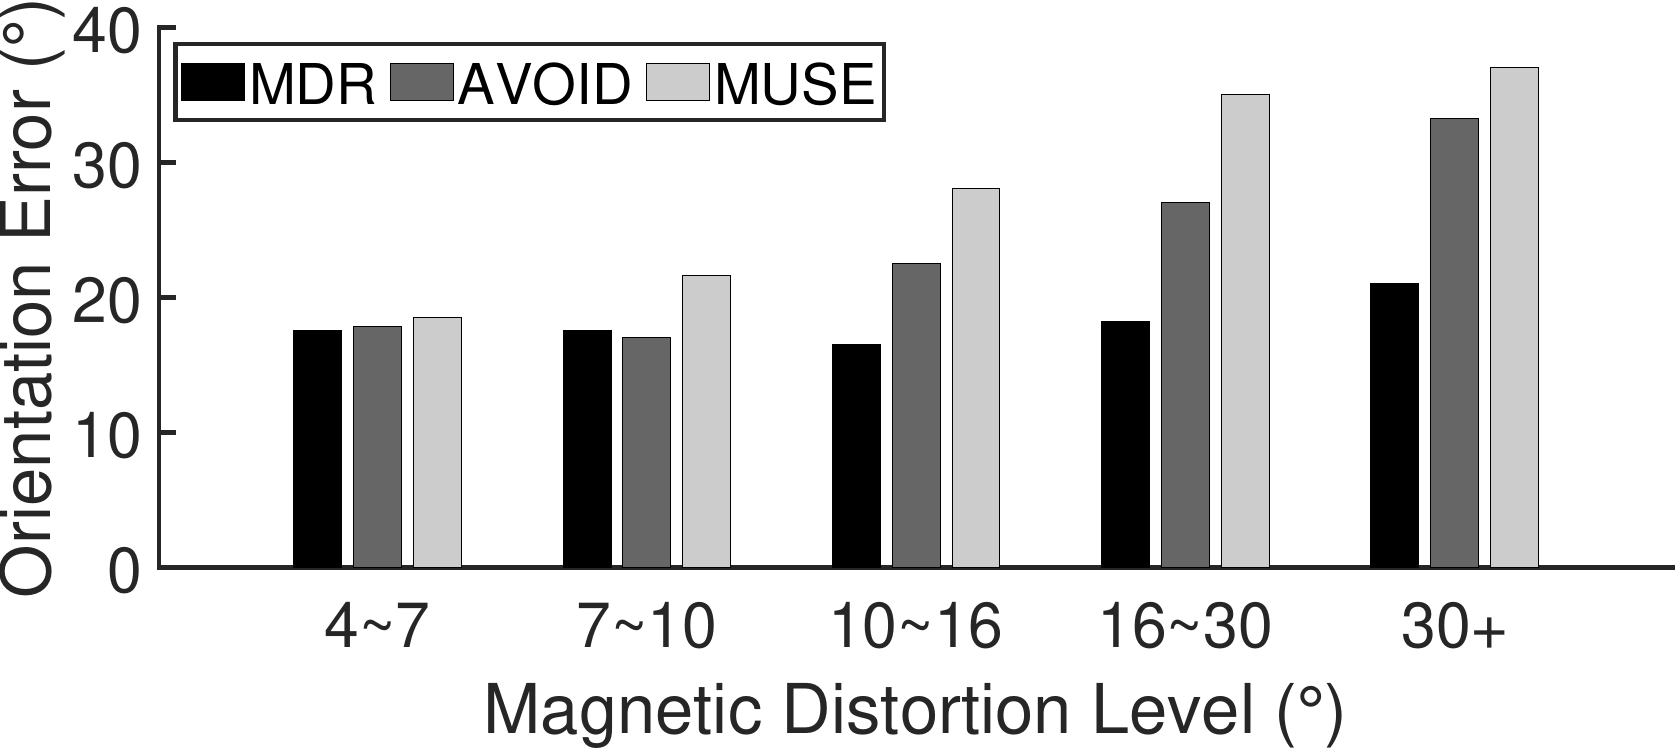}
        \captionsetup{labelformat=empty}
        % \vspace{-7mm}
        \caption{Orientation error of the baselines at different magnetic distortion levels.}
        % \label{result}
    \end{minipage}
\end{figure}

Reviewer 3 mentioned two other works on solving magnetic distortion: “An Adaptive Orientation Estimation Method for Magnetic and Inertial Sensors in the Presence of Magnetic Disturbances” \cite{fan2017adaptive}.
“Accurate Orientation Estimation Using AHRS under Conditions of Magnetic Distortion” \cite{ahrs}.
We have looked into the two works and implemented them into experiment for comparison.

Specifically, we included a custom baseline named \textit{AVOID}, via taking the idea from \cite{fan2017adaptive,ahrs}, i.e. to reduce magnetometer usage when magnetic distortion is severe, therefore avoiding its negative impact.
We mainly refer to the strategy from the later work~\cite{fan2017adaptive}, and incorporate it into a complementary filter, with all modifications used in \aliasSystem, except the database design of \aliasSystem, so that the only difference between \textit{AVOID} and \aliasSystem is the way they resist magnetic distortion.
Later in evaluation (Section~\ref{eval_distortion}) we compare \aliasSystem and AVOID, which proves that fundamentally modelling the distorted magnetic field via a database provides stronger resistance to the distortion (Section~\ref{eval_distortion}).
\aliasSystem is not the first that tries to resist magnetic distortion in orientation estimation.
However, in this work we study the solution of 'fundamentally model magnetic field distortion in orientation estimation', and the experiment in Section~\ref{eval_distortion} verifies the distortion resistant capability of \aliasSystem.
Figures of the experiments are attached below:

\begin{figure} [H]
    % % \vspace{-0.2cm}
    \hfill
    \begin{minipage}[t]{0.50\linewidth}
        % \hspace{-1mm}
        \centering
        % % \vspace{-2cm}
        \includegraphics[width=1\linewidth]{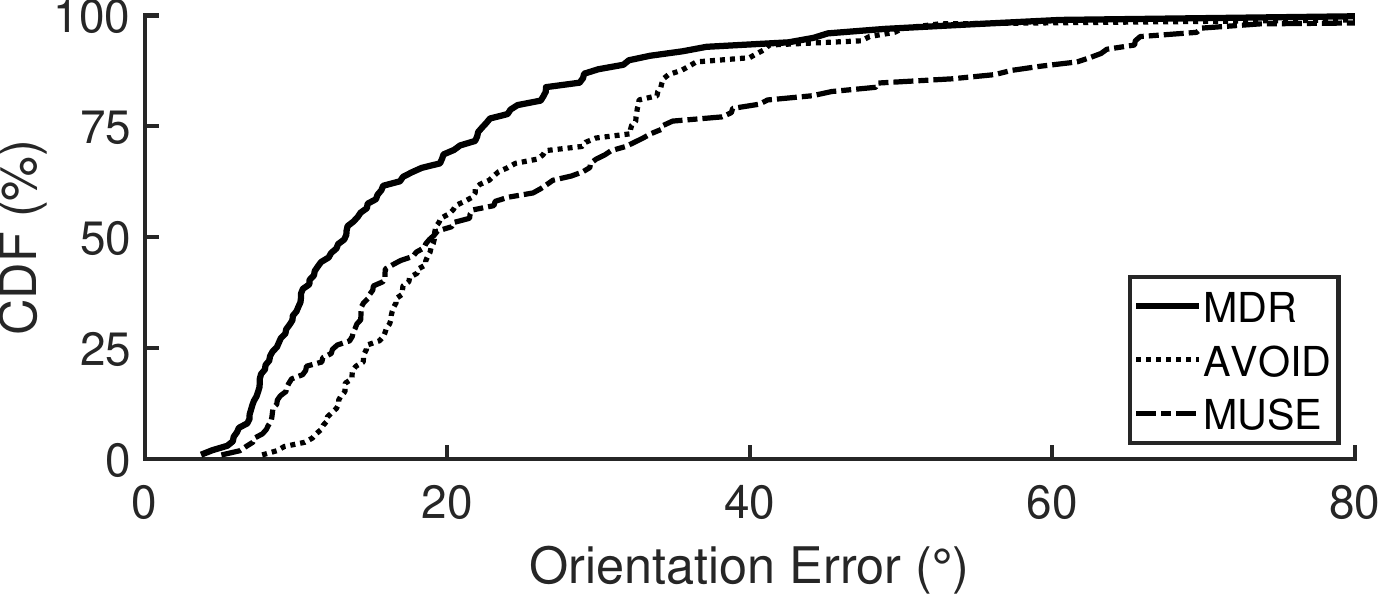}
        \captionsetup{labelformat=empty}
        % % \vspace{-4mm}
       \caption{Overall orientation error comparison between baselines.}
        % \label{overall}
        % % \vspace{-4mm}
    \end{minipage}
    \hfill
    \begin{minipage}[t]{0.40\linewidth}
        \centering
        % % \vspace{-0.1cm}
        \includegraphics[width=1\linewidth]{fig/sensys_eval_dev.pdf}
        \captionsetup{labelformat=empty}
        % % \vspace{-7mm}
        \caption{Orientation error of the baselines at different magnetic distortion levels.}
        % \label{result}
    \end{minipage}
    \hfill
    % % \vspace{-4mm}
\end{figure}

\subsection{}
\textbf{Original review:} \textit{'incorporate a quantitative comparison with SOTA methods from other papers or existing IMU manufacturers (R4)'}

\textbf{Corresponding revision:}
In previous submission, we only compared \aliasSystem with a classical complementary filter (CF), while in this revision, we included MUSE~\cite{muse}, the state-of-the-art orientation estimation method, which also uses a complementary filter as basis.
Additionally, we included another custom baseline named \textit{AVOID} (introduced in Section~\ref{baselines}).
\textit{AVOID} stands for the methods that avoid the negative effect of magnetic distortion, without modelling it~\cite{fan2017adaptive,ahrs}.
We take the key idea from \cite{fan2017adaptive} (explained in Section~\ref{baselines}), and incorporate it into a complementary filter, along with all modifications used in \aliasSystem.
The only difference between \textit{AVOID} and \aliasSystem is the way they deal with magnetic distortion.
Therefore via comparing \aliasSystem and AVOID, we prove that fundamentally modelling the distorted magnetic field provides better resistance to magnetic distortion in orientation estimation.

\begin{figure} [H]
    % % \vspace{-0.2cm}
    \hfill
    \begin{minipage}[t]{0.50\linewidth}
        \hspace{-1mm}
        \centering
        % % \vspace{-2cm}
        \includegraphics[width=1\linewidth]{fig/sensys_eval_overall.pdf}
        \captionsetup{labelformat=empty}
        % \vspace{-4mm}
       \caption{Overall orientation error comparison between baselines.}
        % \label{overall}
        % \vspace{-4mm}
    \end{minipage}
    \hfill
    \begin{minipage}[t]{0.40\linewidth}
        \centering
        % % \vspace{-0.1cm}
        \includegraphics[width=1\linewidth]{fig/sensys_eval_dev.pdf}
        \captionsetup{labelformat=empty}
        % \vspace{-7mm}
        \caption{Orientation error of the baselines at different magnetic distortion levels.}
        % \label{result}
    \end{minipage}
    \hfill
    % \vspace{-4mm}
\end{figure}

\subsection{}
\textbf{Original review:} \textit{'explain the ground truth of orientation (R4)'}

\textbf{Corresponding revision:}
In previous submission we only briefly introduced our ground truth data collection.
In this revision, we assigned a separate subsection (Section~\ref{ground truth}) to introduce our data collection method.
We bind a smart watch (with IMU sensors in it) to a VR controller, and use the technique from~\cite{miao} to convert the controller's orientation and location to the smart watch, so that we can acquire the smart watch's orientation and location.
The VR device adopts computer vision based tracking technique to
locate the controller, and thus can provide accurate ground truth.
Its orientation error is below 0.85° and location error is below 0.7 cm (\cite{miao}).

\subsection{}
\textbf{Original review:} \textit{'both R1 and R4 raise the issue of differences between devices. This can be addressed by evaluating a variety of different devices (chipsets/phones)'}

\textbf{Corresponding revision:}
We use Fossil Gen 5 smartwatch for experiments. 
It is equipped with AK0991X magnetometer and LSM6DSO 6-axis accelerometer with gyroscope.
There are also other mobile devices that use the same sensors, such as Sony Xperia 1 III, Oneplus 7, Motorola moto g fast, MiWatch, Xiaomi Mi 10T Pro, and TicWatch Pro 3. 

Additionally, to prove the scalability of \aliasSystem, we added a IMU hardware comparison experiment in Section~\ref{hardware}, which compares the IMU raw readings between our smart watch, a Samsung Galaxy S21 5G, and an iPhone XS max.
Figure~\ref{compare} shows the visualized results, and statistics shows that  the sensors’ relative similarities between the smartwatch and the Samsung
Galaxy S21 are 91.91$\%$, 95.18$\%$, and 97.76$\%$, for accelerometer, gyroscope, and magnetometer respectively. 
Similarities between the smartwatch and the iPhone are 97.25$\%$ 97.34$\%$, and 98.16$\%$.
This should prove \aliasSystem's scalability to other smart platforms.

\begin{figure} [H] 
    \subfigure[Watch Acc.]{\includegraphics[width=0.3\linewidth]{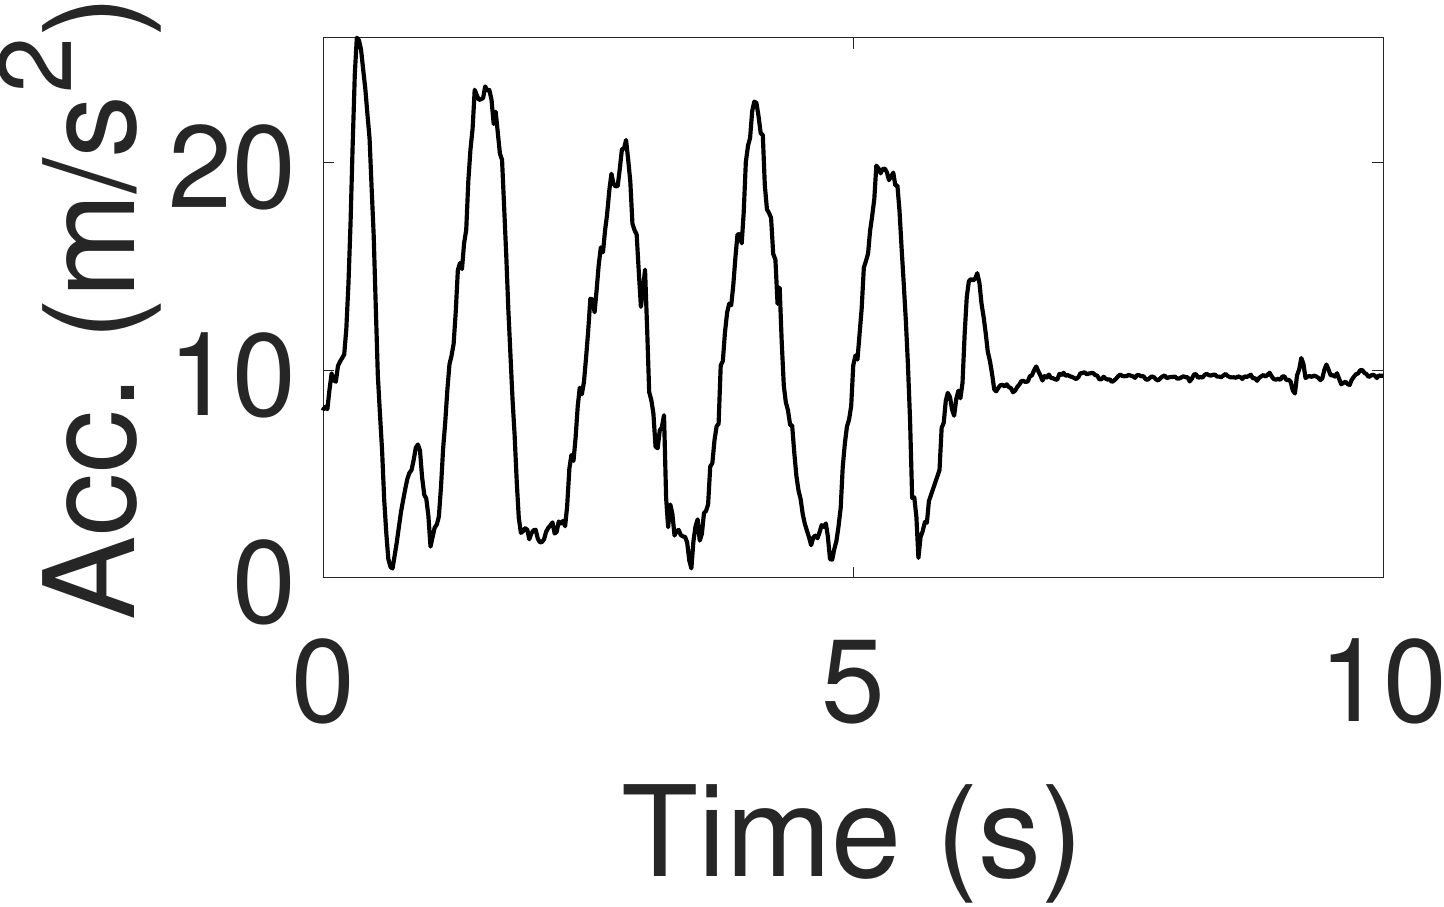}}
    \subfigure[Samsung Acc.]{\includegraphics[width=0.3\linewidth]{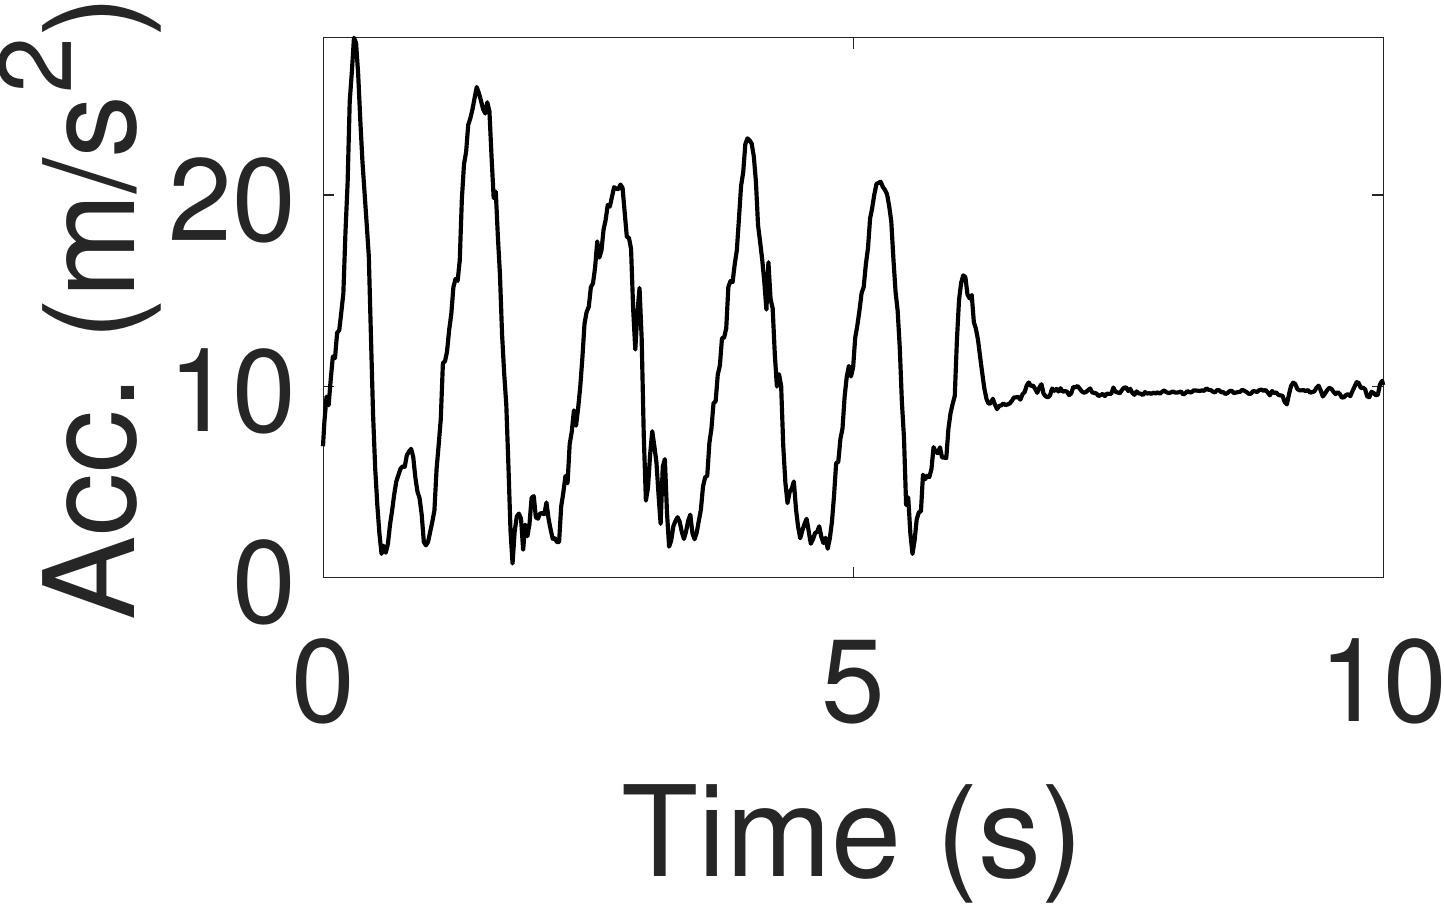}}
    \subfigure[iPhone Acc.]{\includegraphics[width=0.3\linewidth]{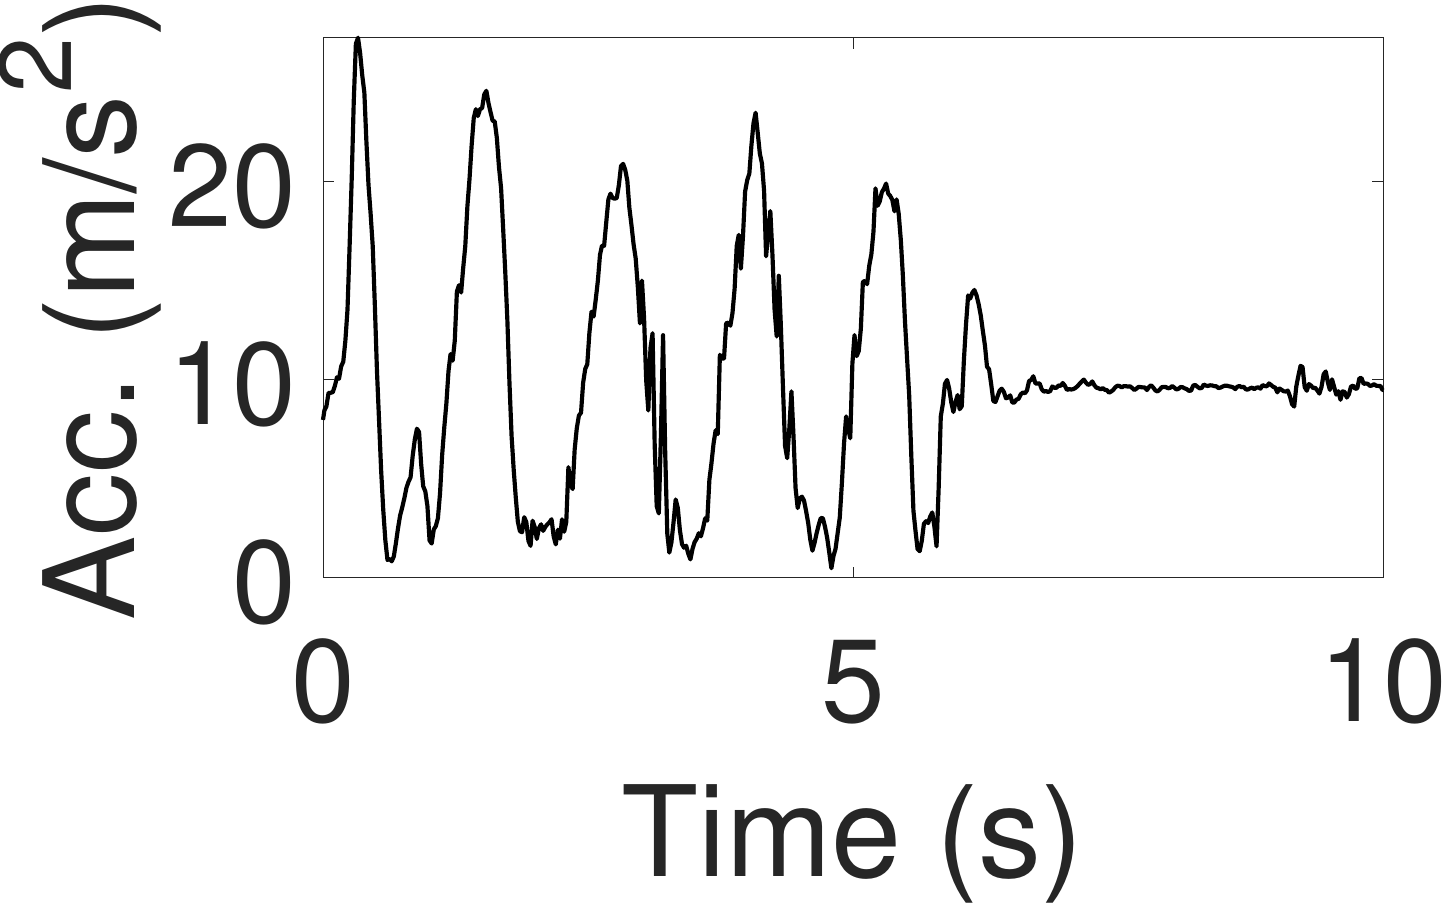}}
    
    \subfigure[Watch Gyro.]{\includegraphics[width=0.3\linewidth]{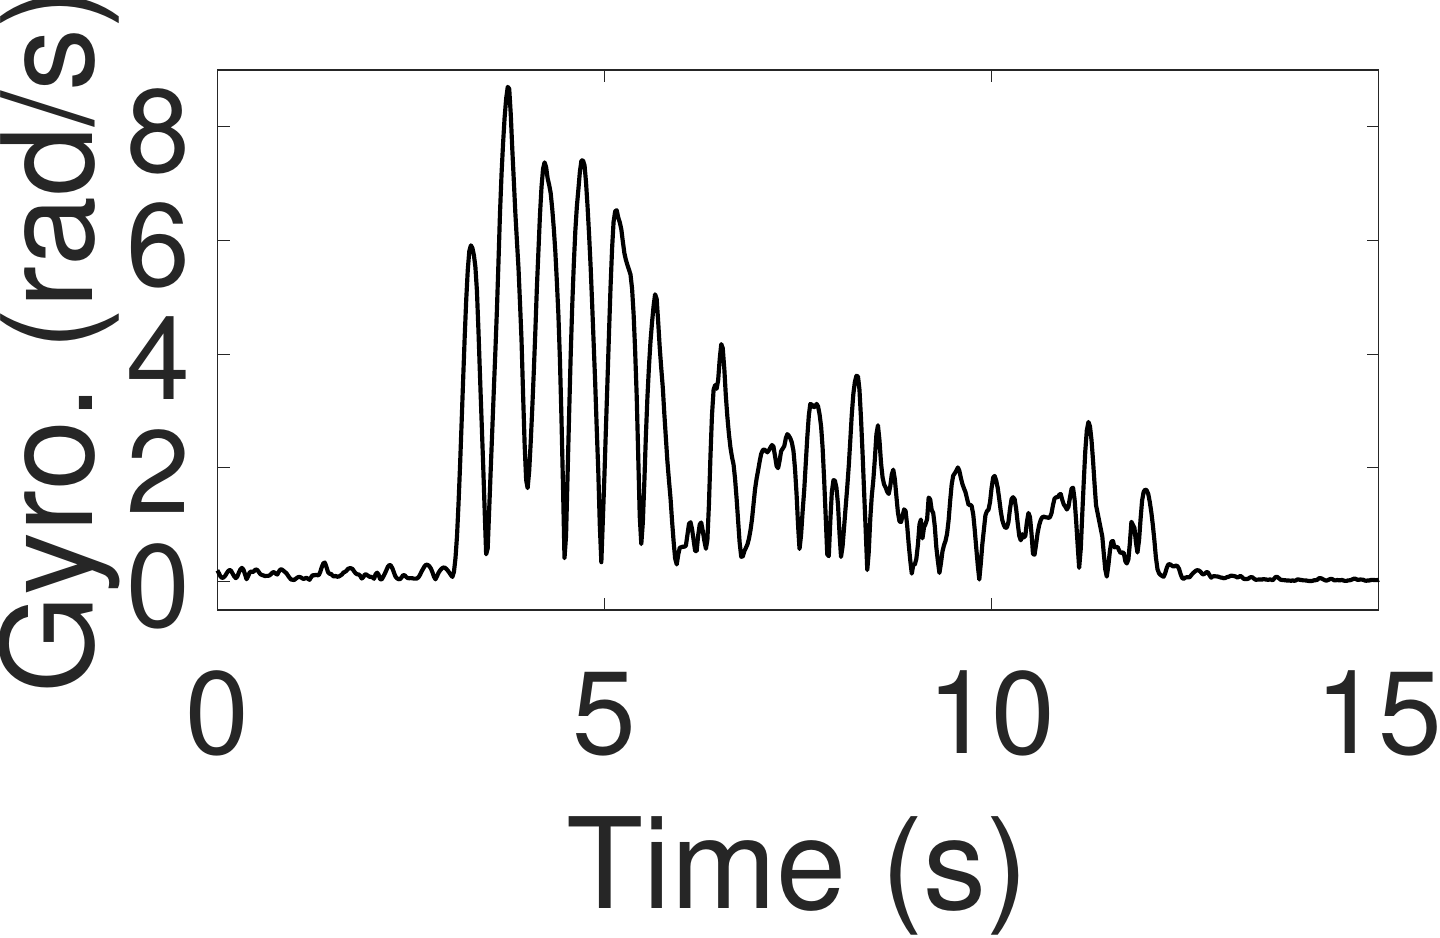}}
    \subfigure[Samsung Gyro.]{\includegraphics[width=0.3\linewidth]{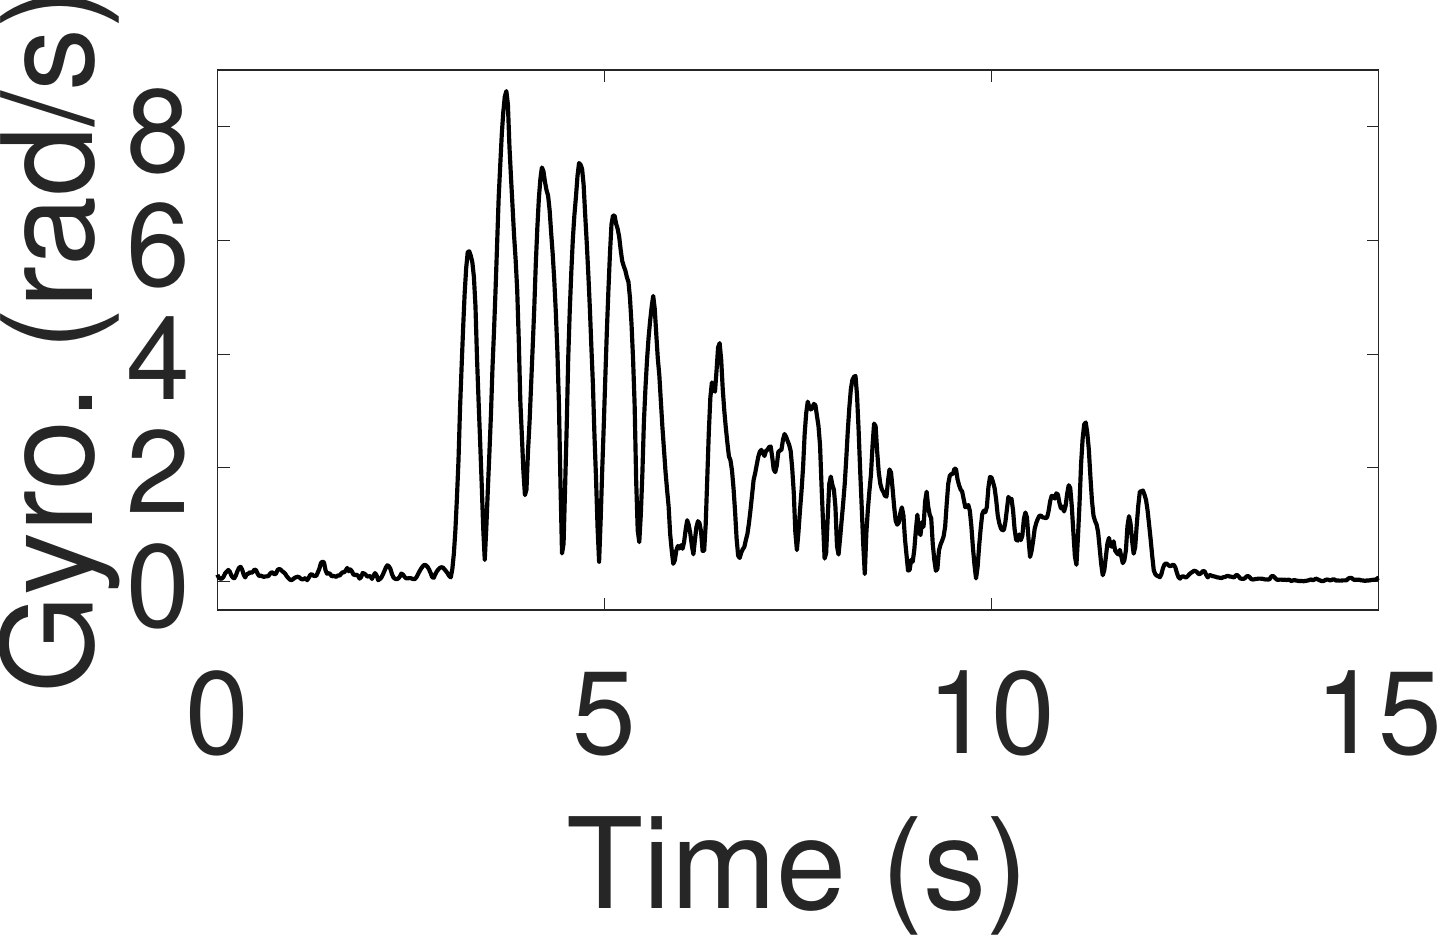}}
    \subfigure[iPhone Gyro.]{\includegraphics[width=0.3\linewidth]{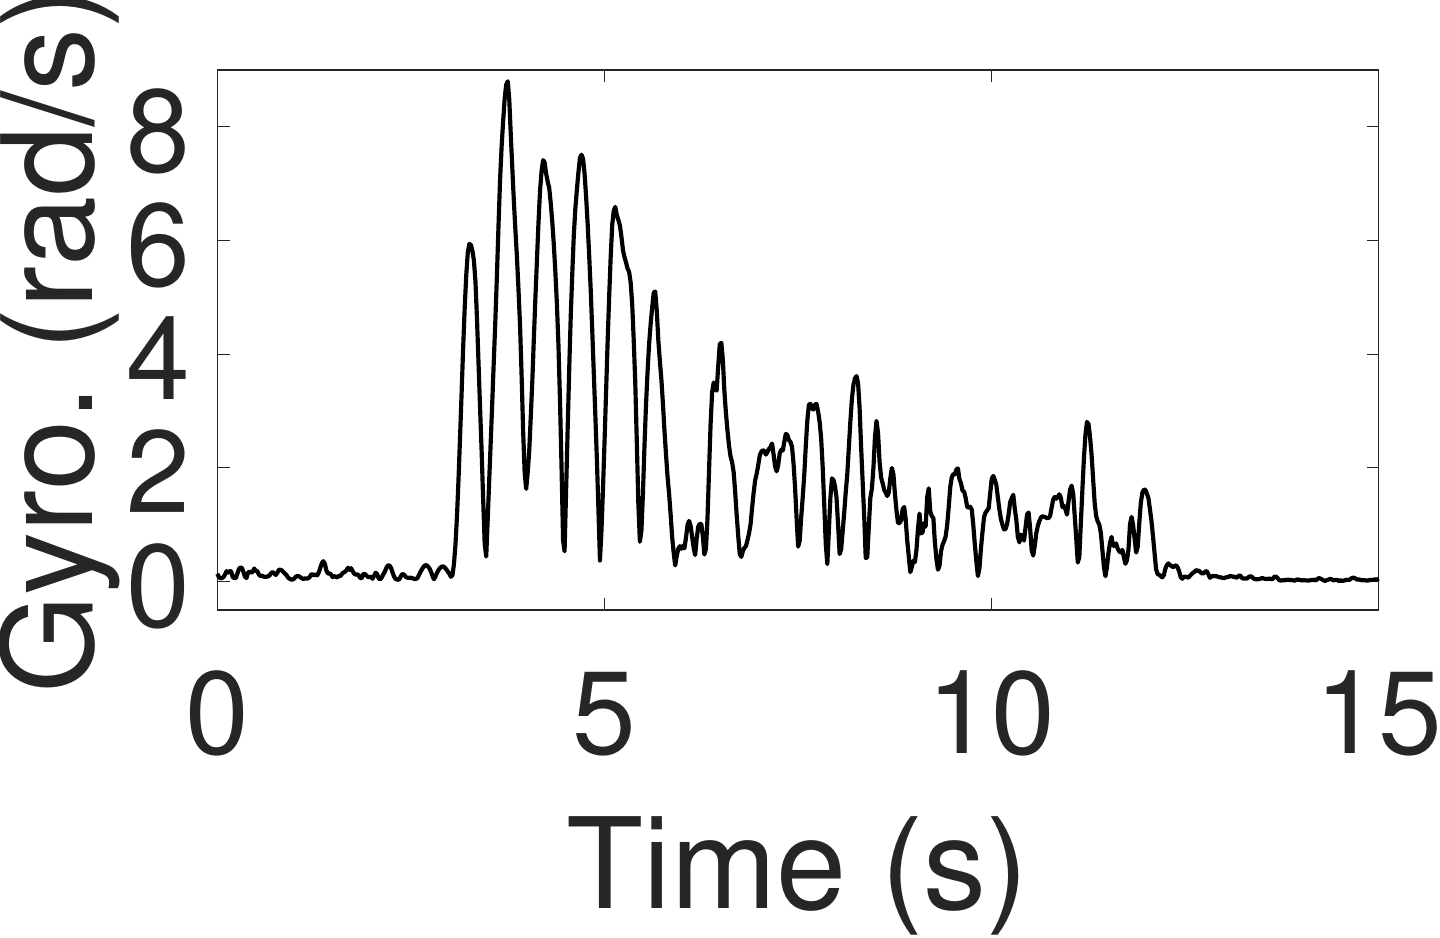}}
    
    \subfigure[Watch Mag.]{\includegraphics[width=0.3\linewidth]{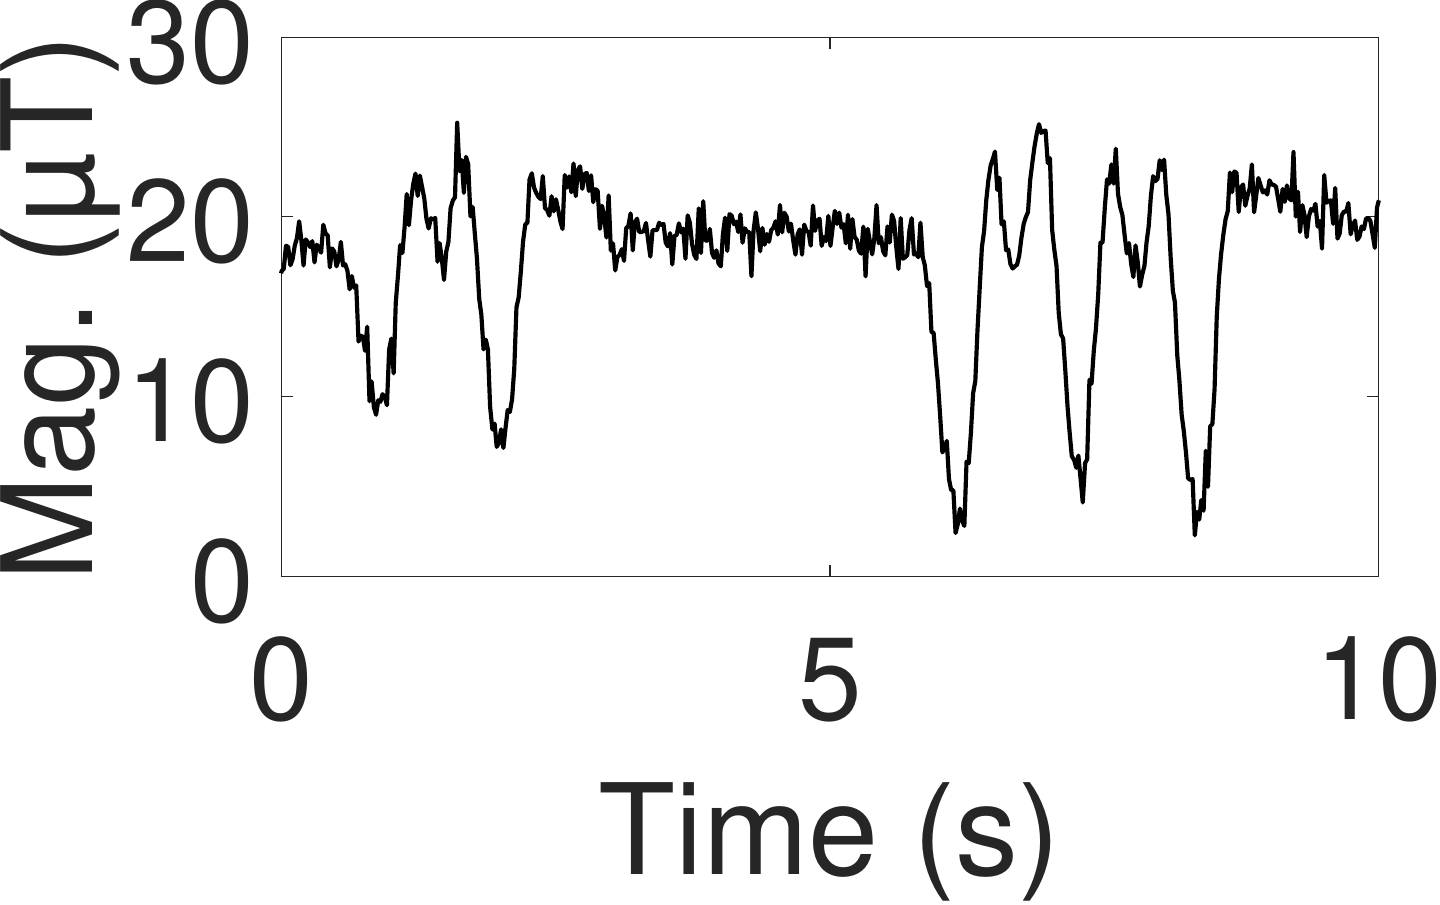}}
    \subfigure[Samsung Mag.]{\includegraphics[width=0.3\linewidth]{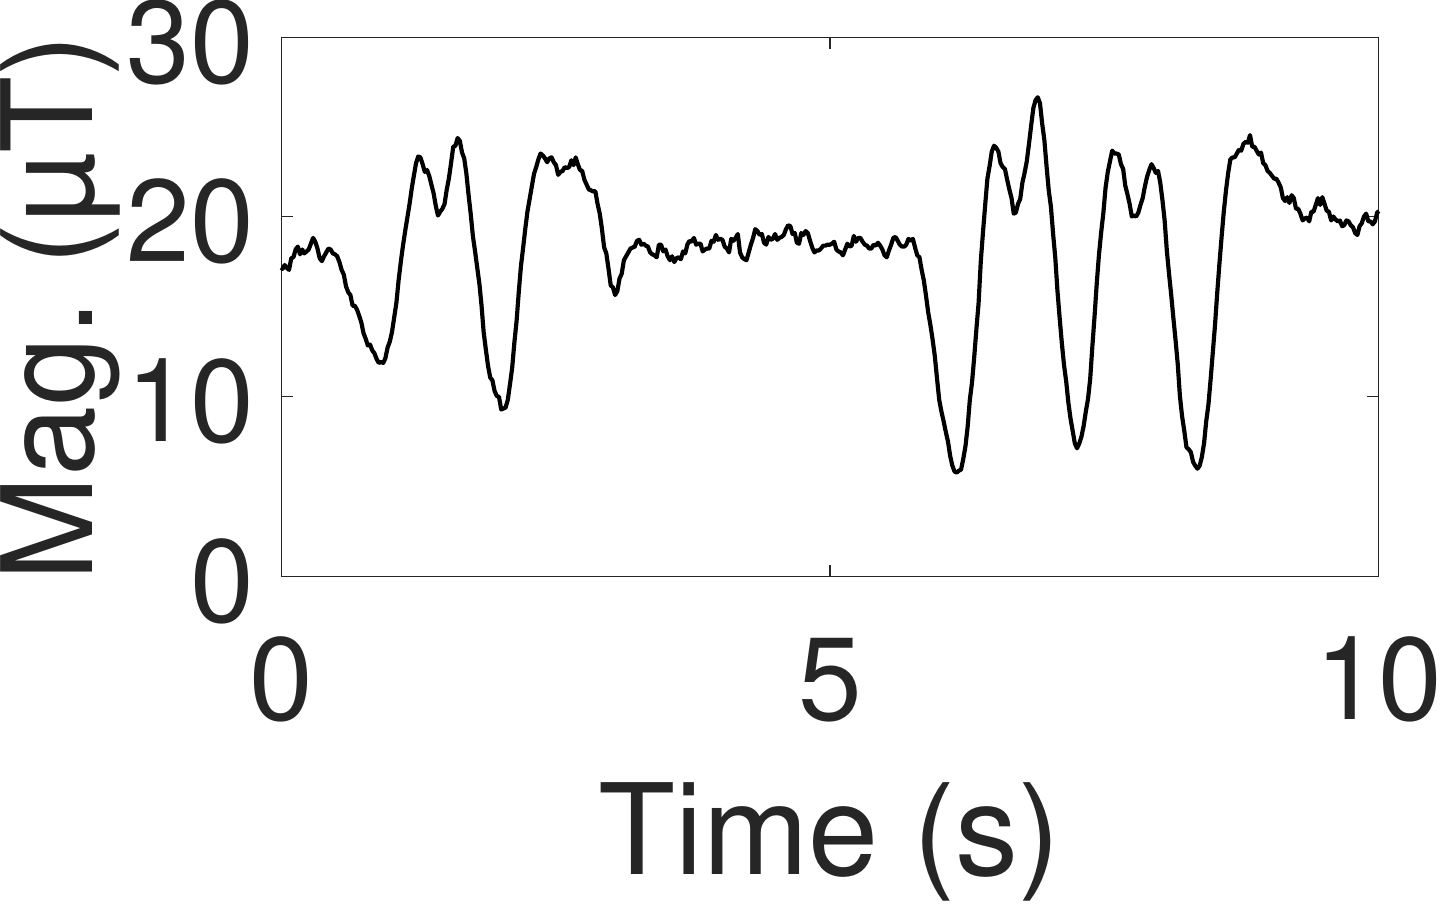}}
    \subfigure[iPhone Mag.]{\includegraphics[width=0.3\linewidth]{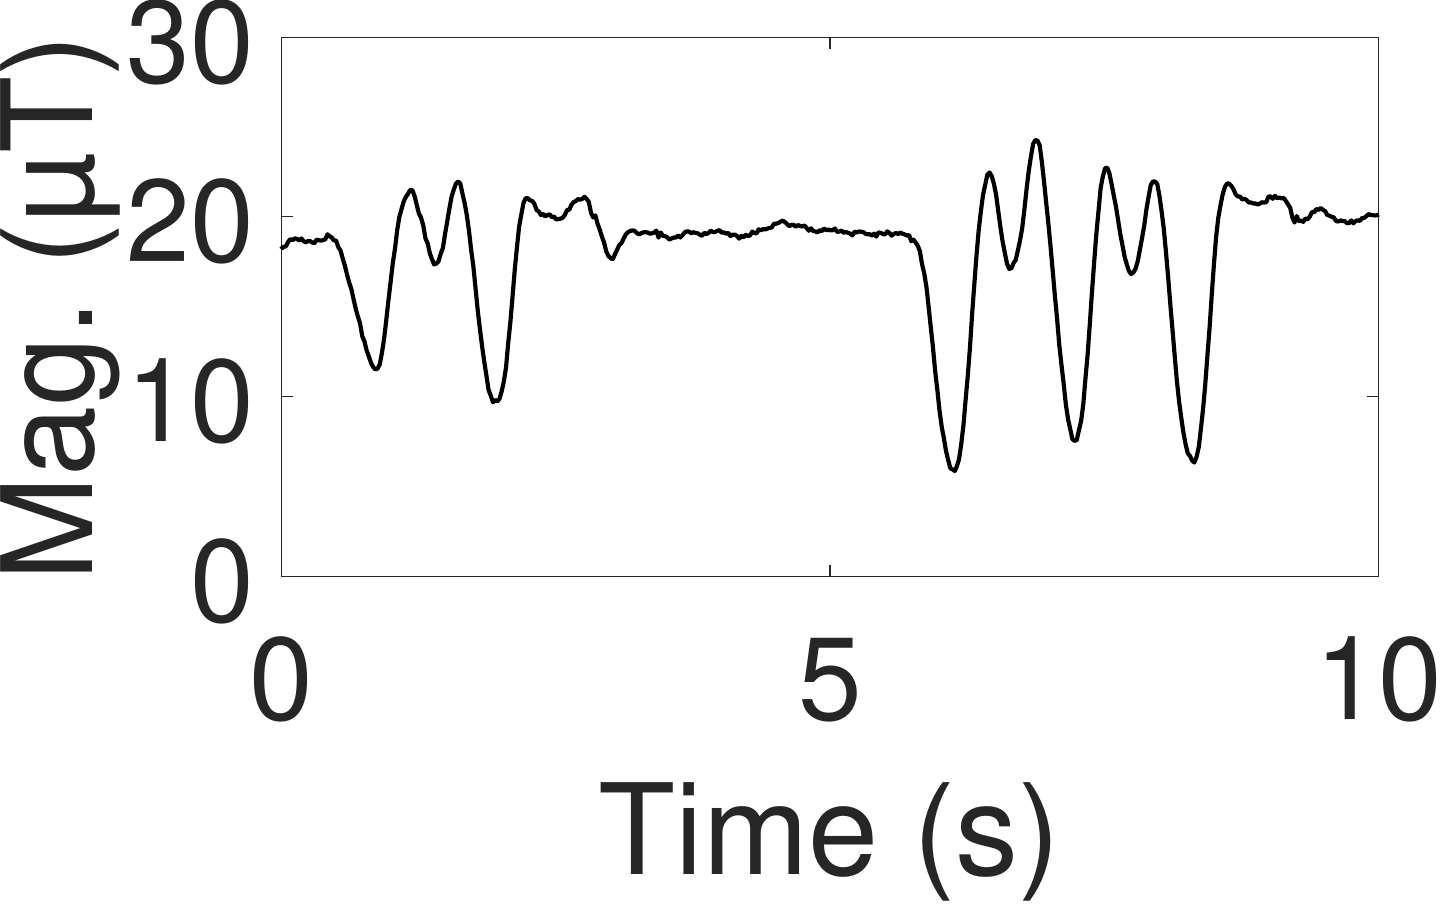}}
    
    % \vspace{-5mm}
    
    \captionsetup{labelformat=empty}
    \caption{Sensor comparison between smart devices}
    % \vspace{-5mm}
\end{figure}

\subsection{}

\textbf{Original review:} \textit{'All reviewers raised the issue of the paper being too long and difficult to read. The writing needs to be significantly improved. I would strongly suggest considering all of reviewer suggestions for making the paper both more legible and concise.'}

\textbf{Corresponding revision:}
% We are terribly sorry about the writing in the previous submission.
We have taken the suggestions and re-written the paper thoroughly.

We rewrote the introduction and made sure that each paragraph corresponds to a major section of the paper.
We also listed the potential contributions of this paper at the end of the introduction, for better understanding.

We thoroughly revised the Related Work (Section~\ref{related}), and migrated it to the top, in order to provide an early understanding on our work's difference between existing methodologies (e.g. magnetic fingerprint).

% of the paper, since we wish to clearly identify our difference from magnetic fingerprint 
We reduced the length of the Background (Section~\ref{secBackground}), but kept the necessary contents related to the topic.

We thoroughly re-organized the Design section.
In the previous submission, we introduce \aliasSystem in different versions (e.g. $MDR_L+D$, $MDR_D$, $MDR$, $MDR+$), which were hard to understand.
In this revision, for better understanding, we name the full system design as \aliasSystem, and cancelled all other version names in the design section.
We introduce the key design of \aliasSystem and its database in Section~\ref{selfDB} (corresponding to $MDR_{L+D} \rightarrow MDR_D \rightarrow MDR$ in the previous submission)
Specifically in Section~\ref{selfDB}, we proposed a new design named Adaptive Updating, introduced in Section~\ref{adaptive_updating}, which was not included in the previous submission.
In Section~\ref{pro}, we introduce the design of reducing errors in database operations (corresponding to $MDR \rightarrow MDR+$ and subsection 'Improving Database Usage' in the previous submission)

We expanded the Evaluation section with more baselines for comparison and more real experiments.
Specifically, in the previous submission, we only compared \aliasSystem with classical complementary filter (CF), while in this revision, we mainly compare with a more meaningful baseline: the current state-of-the-art orientation estimation method MUSE~\cite{muse}, which also uses complementary filter as basis.
Additionally we included a custom baseline named \textit{AVOID}, via taking the idea from \cite{fan2017adaptive,ahrs}, i.e. to reduce magnetometer usage when magnetic distortion is severe, therefore avoiding its negative impact.
We mainly refer to the strategy from the later work~\cite{fan2017adaptive}, and incorporate it into a complementary filter, with all modifications used in \aliasSystem, except the database design of \aliasSystem, so that the only difference between \textit{AVOID} and \aliasSystem is the way they resist magnetic distortion.
Later in evaluation (Section~\ref{eval_distortion}) we compare \aliasSystem and AVOID, which proves that fundamentally modelling the distorted magnetic field via a database provides stronger resistance to the distortion (Section~\ref{eval_distortion}).

% For other expanded real experiments, we first add a IMU hardware comparison in Section~\ref{hardware}, which compares the IMU raw reading between our smart watch, a Samsung Galaxy S21 5G, and an iPhone XS max.
% Figure~\ref{compare} shows the visualized results, and statistics shows that  the sensors’ relative similarities between the smartwatch and the Samsung
% Galaxy S21 are 91.91$\%$, 95.18$\%$, and 97.76$\%$, for accelerometer, gyroscope, and magnetometer respectively. 
% Similarities between the smartwatch and the iPhone are 97.25$\%$ 97.34$\%$, and 98.16$\%$.
% This verifies \aliasSystem's scalability to other smart platforms.

We kept all experiments from previous submission evaluation, including experiments on overall performance~\ref{eval_overall}, different users~\ref{eval_users}, different places~\ref{pla}, different distortion levels~\ref{eval_distortion}, performance decomposition~\ref{decompose}, impact of database resolution~\ref{secDatabaseResolution}, and memory cost~\ref{eval_memory}.
In this revision, we added performance decomposition on adaptive updating~\ref{eval_adaptive_updating}, in order to evaluate our new design component: adaptive database updating (Section \ref{adaptive_updating}).
We also examined location estimation accuracy in Section~\ref{eval_loc}, as it is one important factor in arm tracking and activity recognition.

We also revised the evaluation on analysis on database construction efficiency (Section~\ref{DBeval}).
In Figure~\ref{build up}, beside the old curve 'Database Size', we added another curve 'Database Error', which demonstrates that the database refines its accuracy over time, indicating \aliasSystem's reliability in self-exploring new scenarios.
Additionally in the latency section (Section~\ref{computation latency}), we conducted new real experiment, in which we migrated \aliasSystem onto the Iphone XS Max and tested \aliasSystem's computation latency. 
Result shows, for every 1 second, \aliasSystem can process data of 3.37 seconds, demonstrating its real-time capability on mobile platform.

All experiments are re-conducted with new designs and an extra portion of newly collected data.

\section{Reviewer 5 (2AE)}

\subsection{}

\textbf{Original review:} 
\textit{Lack of meaningful evaluative application}

\textit{While the authors do state in the introduction that increased accuracy of device orientation estimation would improve gesture recognition, Augmented Reality, Virtual Reality, and indoor navigation, they do not provide any meaningful target application to evaluate the effectiveness of their proposed solution.}

\textit{Stated another way... Why is this increase in accuracy of device orientation for indoor environments important? The authors claim an improvement of 4.66 degrees (page 20, paragraph 3) and their database only improves orientation accuracy by 0.61 degrees (page 20, paragraph 3) but it is unclear if this improvement is important in the scope of IMWUT or HCI in general. What type of user interfaces or experiences does 4.66 degrees improvement in orientation estimation enable that was not possible before? or is this work just improvement for the sake of improvement?}

\textit{It will greatly improve the manuscript if the authors provide a measurable application usage scenario that their proposed method improves/enables. For example, if the authors demonstrated a VR application that required good orientation estimation, lost item retrieval, or even an in-air writing application and then showed a quantitative and qualitative improvement in performance and usability with and without the proposed solution, that would go a long way to demonstrating the importance of their work.}

\textit{As it stands now, it is hard to understand what the proposed method will enable that is not already possible.}

\textbf{Corresponding revision:} 
In the previous submission, in Section 5.6 Performance Decomposition, 4.66° (21.98°-17.32° = 4.66°) stands for the improvement via database design (page 20).
The 0.61° (4.66°-4.01° = 0.65°) stand for the difference between the database improvement with and without the Error-Reduction design.
However, we have removed the 0.61° in this revision, in order to avoid misunderstanding.
In this revision, we compared \aliasSystem with MUSE, and \aliasSystem's overall performance is 16.42°, which is  44.47$\%$ better than MUSE.

\begin{figure} [H]
    \hspace{-1mm}
    \centering
    % % \vspace{-2cm}
    \includegraphics[width=0.6\linewidth]{fig/sensys_eval_overall.pdf}
    \captionsetup{labelformat=empty}
    % \vspace{-4mm}
   \caption{Overall orientation estimation error.}
    % \label{overall}
    % \vspace{-4mm}
\end{figure}

As for the impact of orientation accuracy in real use cases, first, improvement in orientation estimation accuracy can support many applications, e.g. VR graphic rendering, human activity recognition and motion tracking.
Orientation also serves as a basis for odometry-based location estimation, in co-operation with accelerometer, since the raw acceleration measurement requires to be transformed via orientation into global reference in order to be integrated into movement traces.

To provide an concrete example, in this revision, we included an extended case study in the evaluation section (Section~\ref{eval_star}).
An demonstration of the application is shown below:

\begin{figure}[H]
    \centering
    \includegraphics[width=0.5\linewidth]{fig/ubi_star_sky.pdf}
    \captionsetup{labelformat=empty}
    \caption{Star sky application}
    % \label{fig:enter-label}
\end{figure}

We discuss a star sky view application which uses orientation results to render the stars and constellations on smart phones.
Such an application transforms the orientation result into star sky rendering accuracy.
\aliasSystem's overall accuracy of star sky rendering in such application is 86.69$\%$.
As comparison, MUSE has an accuracy of 70.92$\%$.
We also plot the performance of \aliasSystem and MUSE in Figure~\ref{star_2} and Figure~\ref{star_1} (also shown below).
This experiment should justify the improvement of \aliasSystem in a real-use application over the existing work.

\begin{figure} [H]
    % % \vspace{-0.2cm}
    \hfill
    \begin{minipage}[t]{0.30\linewidth}
        \hspace{-0.1cm}
        \centering
        % % \vspace{-2cm}
        \includegraphics[width=1\linewidth]{fig/ubicomp_star_2.pdf}
        \captionsetup{labelformat=empty}
        % \vspace{-7mm}
       \caption{Star sky rendering accuracy CDF.}
        % \label{star_2}
    \end{minipage}
    \hfill
    \begin{minipage}[t]{0.30\linewidth}
        \centering
        % % \vspace{-0.1cm}
        \includegraphics[width=1\linewidth]{fig/ubicomp_star_1.pdf}
        \captionsetup{labelformat=empty}
        % \vspace{-7mm}
        \caption{Star sky rendering accuracy over time.}
        % % \vspace{-0.5cm}
        % \label{star_1}
    \end{minipage}
    \hfill
    \hfill
    % \vspace{-4mm}
\end{figure}

\subsection{}

\textbf{Original review:} \textit{Why is fingerprinting the best solution?}

\textbf{Corresponding revision:}
First, we would like to distinguish \aliasSystem from fingerprinting.
Fingerprinting is a technique used in location estimation, as it records the pattern of local magnetic field and perform matching to locate devices.
However, in our work, although \aliasSystem also tries to record the magnetic field via a database, it uses the database to correct magnetic calibration.
Additionally there are other factors that make \aliasSystem's database different from fingerprinting for localization.
Details can be found in Section~\ref{related}.

We then answer the question of 'Why modelling magnetic distortion with a database is the best solution? (in the context of orientation estimation)'
To that end, we compare our solution with existing magnetic distortion handling methods.
To be specific, in this revision, we included an custom baseline named \textit{AVOID} (introduced in Section~\ref{baselines}).
\textit{AVOID} stands for the methods that avoid the negative effect of magnetic distortion, without modelling it~\cite{fan2017adaptive,ahrs}.
We take the key idea from \cite{fan2017adaptive} (introduced with Equation~\ref{baseline1}-\ref{lambda} and explanations in Section~\ref{baselines}), and incorporated it into a complementary filter, along with all modifications used in \aliasSystem.
The only difference between \textit{AVOID} and \aliasSystem is the way they deal with magnetic distortion.
Therefore via comparing \aliasSystem and AVOID, we prove that fundamentally modelling the distorted magnetic field provides better resistance to magnetic distortion in orientation estimation.
Experimental results in Section \ref{eval_distortion} shows that \aliasSystem has stronger distortion resistant capability than \textit{AVOID}, indicating that modelling magnetic distortion with a database is the better solution to magnetic distortion.

\begin{figure}[H]
    % % \vspace{-0.2cm}
    \begin{minipage}[t]{0.42\linewidth}
        \centering
        % % \vspace{-0.1cm}
        \includegraphics[width=1\linewidth]{fig/sensys_eval_dev.pdf}
        \captionsetup{labelformat=empty}
        % \vspace{-7mm}
        \caption{Orientation error of the baselines at different magnetic distortion levels.}
        % \label{result}
    \end{minipage}
\end{figure}

\subsection{}

\textbf{Original review:} \textit{While fingerprinting has been shown to work for both localization and orientation estimation for well-controlled environments. It is generally not considered to be a viable solution since the environments are not static, and thus the database must be continually updated. For instance, every time the furniture in a room is moved, an appliance is changed, or a new magnet is brought into the space, there is the potential that the baseline magnetic field distribution will change. One key question is how stable the magnetic field distortion is over time.}
\textit{The authors claim that "the pattern of magnetic field distortion is chronologically stable" (page 2, paragraph 3). Is this true? What if the user moves their laptop (or other soft iron or hard iron object) to a new location (not captured in the database), will this not change the earth's field distribution? Will this change in the earth's field effect the orientation estimation accuracy? will it effect the system performance?}

\textbf{Corresponding revision:}
We identify the question of 'how stable the magnetic field distortion is over time.' as Temporal Stability (Section \ref{stability}, corresponding to Section 3.5.1: Chronological stability in the previous submission, and also shown below).
In Section \ref{stability}, we recorded a static magnetometer’s readings in an indoor environment for 12 hours, and plotted its 3-axis readings in Figure~\ref{temporal} (corresponding to Figure 11 in the previous submission).
Result shows that, despite a constant measurement noise, the magnetic field is relatively stable over time.

\begin{figure}[H]
    % \vspace{-0.3cm}
    % \begin{minipage}[t]{0.45\linewidth}
    %     \centering
    %     \includegraphics[width=\textwidth]{fig/sensys_muse_devM.pdf}
    %      % \vspace{-7.5mm}
    %     % \caption{Impact of different magnetic distortion levels.}
    %     \caption{Impact of magnetic distortion.}
    %     % % \vspace{0cm}
    %     \label{muse_devM}
    % \end{minipage}
    \hspace{0.1cm}
    \begin{minipage}[t]{0.3\linewidth}
        \centering
        \includegraphics[width=\textwidth]{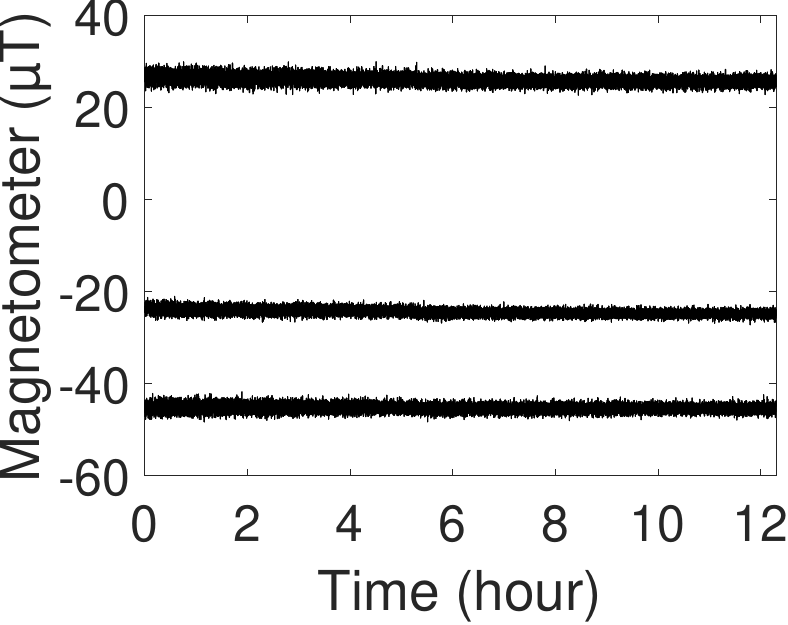}
         % \vspace{-7.5mm}
         \captionsetup{labelformat=empty}
        \caption{Temporal stability of magnetic field.}
        % % \vspace{0cm}
        % \label{temporal}
    \end{minipage}
    % \vspace{-4mm}
\end{figure}

As for the situation where a new magnet is brought into the space, the magnetic field will definitely change.
However, our system \aliasSystem has the capability of automatic database updating, as introduced in Section \ref{selfDB}.
\aliasSystem requires no prior knowledge to distorted magnetic field.
Instead, it fully relies on the self-exploration via automatic updating to build its own database for the local magnetic field.
Figure \ref{build up} in Section \ref{DBeval} shows that the database would constantly build and refine itself (since \aliasSystem visits the same places multiple times, and averaging multiple visits will increase accuracy).
According to Figure \ref{build up} (also shown below), it would reach a relatively good accuracy and reliability after 300 seconds.

\begin{figure}[H]
    % \hfill
    \begin{minipage}[t]{0.38\linewidth}
        \centering
        % % \vspace{-0.1cm}
        \includegraphics[width=1\linewidth]{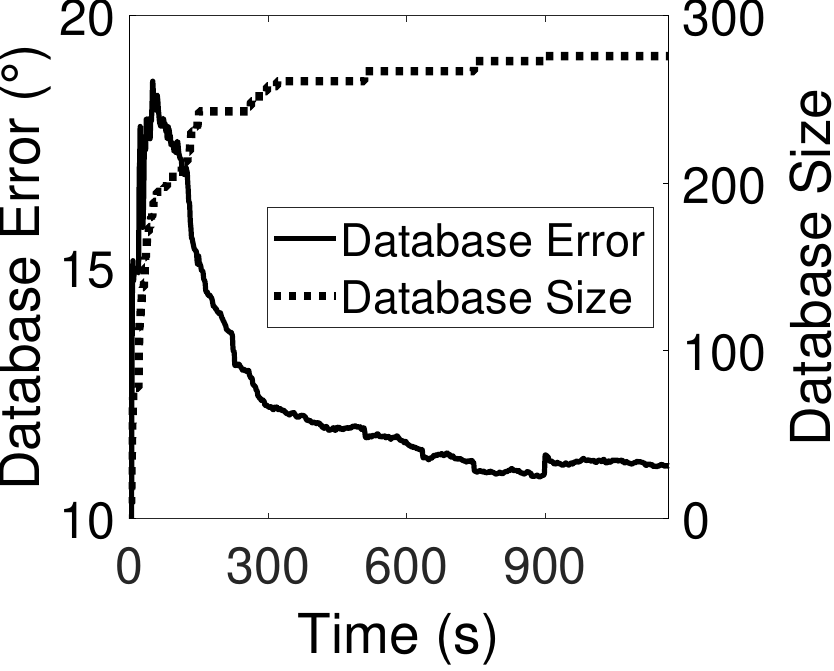}
        % \vspace{-7mm}
        \captionsetup{labelformat=empty}
        \caption{Database accuracy and size during construction.}
        % % \vspace{-0.5cm}
        % \label{build up}
    \end{minipage}
\end{figure}

As long as the new magnet is put in place before \aliasSystem starts running, \aliasSystem can fit itself into the environment and model the distortion pattern. 
Therefore, for the question: \textit{'What if the user moves their laptop (or other soft iron or hard iron object) to a new location (not captured in the database).'}, since \aliasSystem requires no prior knowledge to the new location and its magnetic field, this situation will not hurt \aliasSystem's performance, as all our experiments were conducted with an empty database at the beginning.

As for the situation where the new magnet is brought into space after \aliasSystem starts running, i.e. the ground truth of distortion pattern changes during database updating, we had such situation during our experiment at the place 'Stairwell' (introduced in Section \ref{places}).
At the ’Stairwell’, the nearby 2-meter-tall metal doors at the floor entrance frequently open and close due to the commuting crowd, making the magnetic distortion pattern occasionally changing.
Therefore at the ’Stairwell’, \aliasSystem is slightly worse than \textit{AVOID} (Section \ref{pla}), who simply reduces magnetometer usage when distortion is detected.
This is shown in Figure~\ref{place}, and also shown below:

\begin{figure} [H]
    \hspace{-0.1cm}
    \centering
    % % \vspace{-2cm}
    \includegraphics[width=.58\linewidth]{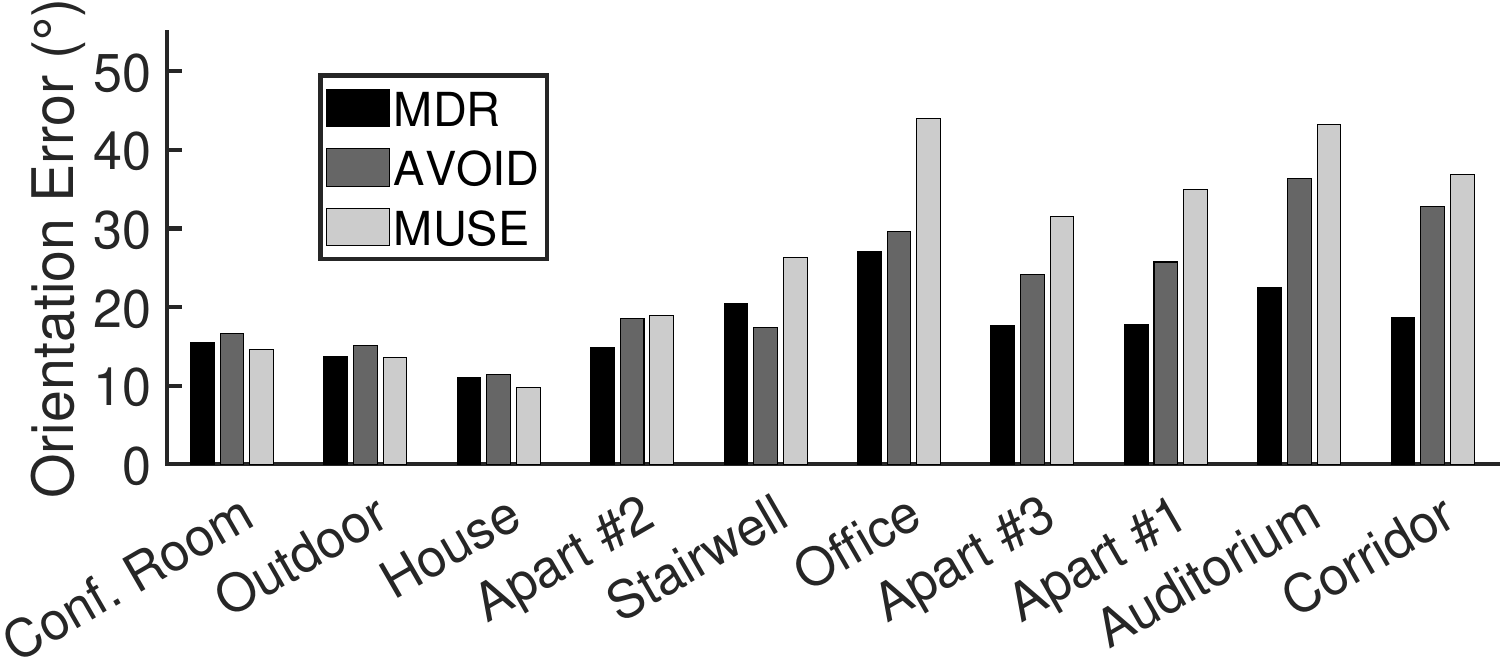}
    % \vspace{-4mm}
    \captionsetup{labelformat=empty}
    \caption{Performance at different places.}
    % \label{place}
    % \vspace{-5mm}
\end{figure}

In conclusion, as long as there is no artificial change to the magnetic environment, the magnetic field would be stable, and \aliasSystem would work well.
If there is limited artificial change to the magnetic environment (e.g. 2-meter-tall metal doors open and close), \aliasSystem will perform worse, but sightly.
In the theoretical worst case, where the local magnetic field changes both constantly and dramatically (e.g. maybe nearby a nuclear fusion reactor), we argue that the magnetometer should not be used at all, and all IMU-based orientation estimation methods will degrade to 'gyroscope + accelerometer' solution.

\subsection{}

\textbf{Original review:} \textit{If the goal is simply to improve orientation estimation, why not just calibrate the 3D magnetometer each time? IOS and Android devices both provide mechanisms that calibrate the magnetometer by rotating the phone or smartwatch to different orientations to measure the local distortion of the magnetic field. Why is this not enough? What applications are the authors proposing that this standard method of calibration is not suitable for?}

\textbf{Corresponding revision:}
We would like to point out that \textit{'calibrate the 3D magnetometer each time'} does not calibrate the magnetic distortion at each location.
Magnetic distortion makes the magnetometer’s reading deviate from true north and point to different directions at different locations (Introduction, 4th paragraph).
As an intuitive example is given in figure below (Figure 1 in the previous submission), a distorted magnetic field will have different direction at different location.

\begin{figure}[H] %通栏
    \begin{minipage}[t]{0.45\linewidth}
        \centering
        % % \vspace{-3cm}
        \includegraphics[width=0.7\textwidth]{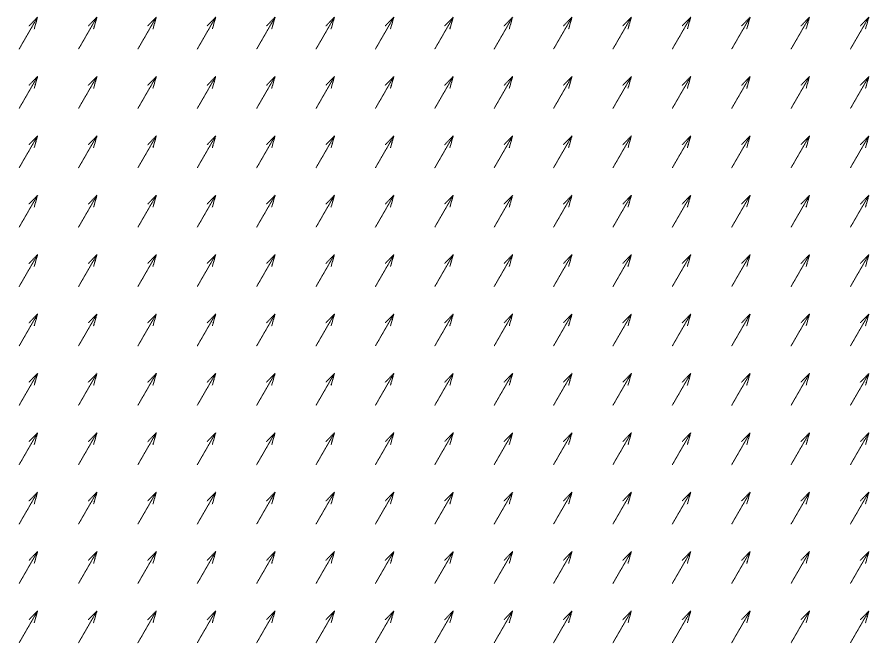}
        \captionsetup{labelformat = empty}
        % % \vspace{-3cm}
        \caption{Example of distortion-free magnetic field}
         % \vspace{-1cm}
        % \label{nodistortion}
    \end{minipage}
    \hspace{0.5cm}
    \begin{minipage}[t]{0.45\linewidth}
        \centering
        % % \vspace{-3cm}
        % \hspace{-1cm}
        \includegraphics[width=0.7\textwidth]{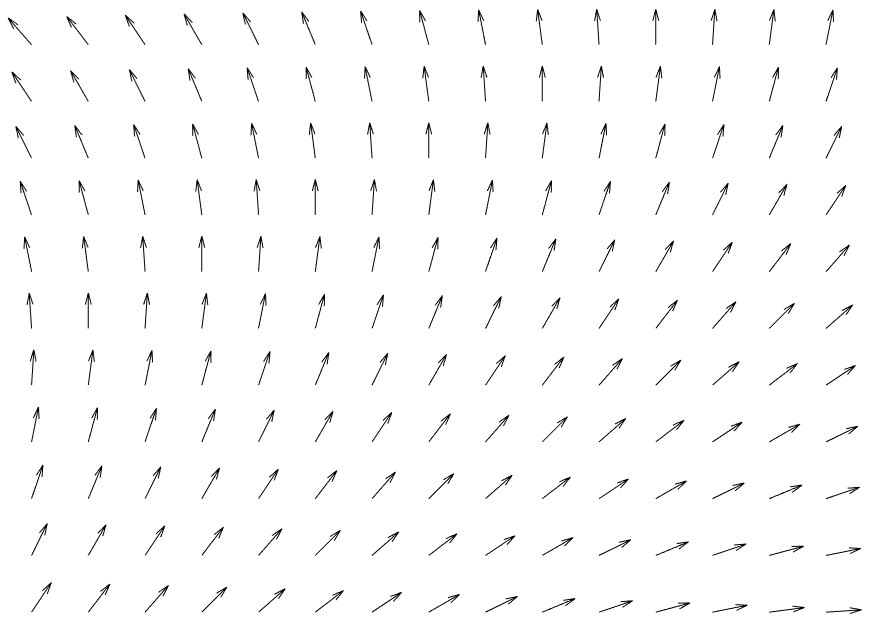}
        \captionsetup{labelformat = empty}
        % % \vspace{-3cm}
        \caption{Example of distorted magnetic field}
        % \label{distortionyes}
    \end{minipage}
       % \vspace{-0.1in}
\end{figure}

Therefore \textit{'calibrate the magnetometer by rotating the phone or smartwatch to different orientations to measure the local distortion of the magnetic field'} is not viable, as the \textit{'local distortion'} is a spatial concept that cannot be fully calibrated at a single location.
\textit{'rotating the phone or smartwatch to different orientations'} maybe be able to calibrate the bias in magnetometer sensor, but no matter how we rotate the phone or smartwatch at one single location, we would not have any knowledge on other locations' magnetic field direction, until we actually visit other locations.

If we want to actually fully calibrate the distortion each time before the system starts, we would have to pre-visit every location that could be visited later, which would induce large preparation overhead.
Different from that, \aliasSystem performs automatic updating (very similar to the \textit{'calibrate'}) to measure the magnetic field at every visited location and built its own database, therefore cancelling the preparation overhead.

% \begin{figure} [H]
%     \centering
%     \hspace{-7mm}
%     \includegraphics[width=0.7\linewidth]{fig/workflow_v10.pdf}
%     % % \vspace{-3.5mm}
%     \captionsetup{labelformat=empty}
%     \caption{MDR System Workflow.}
%     % \label{flow}
%     % \vspace{-5mm}
% \end{figure}

\subsection{}

\textbf{Original review:} \textit{Unclear comparison to state of the art}

\textit{As presented the performance metrics reported in the manuscript are hard to interpret. What is the base line that the work is comparing too CF? MUSE? MDR? MDR+ without database? all of them? Is MDR+ without database part of the contribution or is it just MDR+ database? Given that one of the stated claims of the paper is the inclusion of a database it appears that MDR+ database, only provides a 0.61 degree improvement in accuracy compared to MDR+ without database. Is this significant and important?}

\textit{Furthermore almost all the reported values are given in terms of percent improvement over an ever shifting baseline (CF, MUSE, MDR, MDR+ without database) but it is hard to track down what is the actual improvement in terms of degrees. Again is 4.66 degrees or 0.61 degrees actually important? and if so for what application? do users actually notice a difference?}

\textit{It would significantly improve the readability and ultimate impact of the manuscript if the authors can present their results in a clear and straight forward manor.}

\textbf{Corresponding revision:}
We thoroughly re-organized the Design section, and \aliasSystem now stands for our complete design.
In the previous submission, we introduce \aliasSystem in different versions (e.g. $MDR_L+D$, $MDR_D$, $MDR$, $MDR+$), which were hard to understand.
In this revision, for better understanding, we name the full system design as \aliasSystem, and cancelled all other version names in the design section.
We introduce the key design of \aliasSystem and its database in Section~\ref{selfDB} (corresponding to $MDR_L+D \rightarrow MDR_D \rightarrow MDR$ in the previous submission)
Specifically in Section~\ref{selfDB}, we proposed a new design named Adaptive Updating, introduced in Section~\ref{adaptive_updating}, which was not included in the previous submission.
In Section~\ref{pro}, we introduce the design of reducing errors in database operations (corresponding to $MDR \rightarrow MDR+$ and subsection 'Improving Database Usage' in the previous submission)

As for comparison experiments, in previous submission, we only compared \aliasSystem with a classical complementary filter (CF), while in this revision, we included MUSE~\cite{muse}, the state-of-the-art orientation estimation method, which also uses a complementary filter as basis.
Additionally, we included another custom baseline named \textit{AVOID} (introduced in Section~\ref{baselines}).

We compare \aliasSystem with MUSE and \textit{AVOID} on overall performance~\ref{eval_overall}, different users~\ref{eval_users}, different places~\ref{pla}, different distortion levels~\ref{eval_distortion}.
The overall orientation accuracy improvement over MUSE is 44.47$\%$ (16.42° vs. 29.57°).
The statistics is different from the previous submission, since all experiments are re-conducted with new designs and an extra portion of newly collected data.

\begin{figure} [H]
    % % \vspace{-0.2cm}
    \hfill
    \begin{minipage}[t]{0.50\linewidth}
        \hspace{-1mm}
        \centering
        % % \vspace{-2cm}
        \includegraphics[width=1\linewidth]{fig/sensys_eval_overall.pdf}
        \captionsetup{labelformat=empty}
        % \vspace{-4mm}
       \caption{Overall orientation error comparison between baselines.}
        % \label{overall}
        % \vspace{-4mm}
    \end{minipage}
    \hfill
    \begin{minipage}[t]{0.40\linewidth}
        \centering
        % % \vspace{-0.1cm}
        \includegraphics[width=1\linewidth]{fig/sensys_eval_dev.pdf}
        \captionsetup{labelformat=empty}
        % \vspace{-7mm}
        \caption{Orientation error of the baselines at different magnetic distortion levels.}
        % \label{result}
    \end{minipage}
    \hfill
    % \vspace{-4mm}
\end{figure}

The \textit{'4.66°'} and \textit{'0.61°'} refer to performance decomposition (Section~\ref{decompose}), where we decompose the design of \aliasSystem to demonstrate the performance contribution of each design component.
In this revision, for better understanding, we listed the decomposed baselines in Section~\ref{decompose_baselines}:

\begin{itemize}
    \small
    \item \textit{\textbf{CF:}} \aliasSystem with neither database nor error-reduction, namely a classical complementary filter.
    \item \textit{\textbf{\aliasSystem w/o DB:}} \aliasSystem with the error-reduction designs, but without database.
    \item \textit{\textbf{\aliasSystem w/o ER:}} \aliasSystem with database, but no error-reduction.
    \item \textit{\textbf{\aliasSystem:}} Complete \aliasSystem with database and error-reduction.
    % with both database and error-reduction.
\end{itemize}

Experiment results show that the error-reduction design (Section~\ref{pro}) improves database usage, and lifts the relative improvement via database from 17.18$\%$ (27.42°-22.71° = 4.71°, 4.71°/27.42°=17.18$\%$) to 25.30$\%$ (21.98°-16.42° = 5.56°, 5.56°/21.98°=25.30$\%$).
This demonstrates the co-effect of database design (Section~\ref{design}) and error-reduction design (Section~\ref{pro}), and verifies that error-reduction improves database operation.
Additionally in this revision, we added performance decomposition on adaptive updating~\ref{eval_adaptive_updating}, in order to evaluate our new design component: adaptive database updating (Section \ref{adaptive_updating}).
Specifically, we compare \aliasSystem with a sub-baseline of \aliasSystem without adaptive updating scheme (denoted as \textbf{\aliasSystem w/o AU}), which naively pile the anchors into datapoints, as shown in Equation \ref{Fupdate}.
% instead of adaptive updating shown in Equation \ref{Fupdate3}.
We use the baselines to run complete data traces.
After that, we record the final database error, namely the average direction error of all anchors stored in the database.
% As shown in Figure \ref{eval_au}, 
Average final database error of \aliasSystem is 12.04°, which is 9.13$\%$ lower than the 13.25° of \textbf{\aliasSystem w/o AU}.
This verifies the capability of enhancing database accuracy of the adaptive updating scheme.
% \textit{AVOID} stands for the methods that avoid the negative effect of magnetic distortion, without modelling it~\cite{fan2017adaptive,ahrs}.
% We take the key idea from \cite{fan2017adaptive} (explained in Section~\ref{baselines}), and incorporate it into a complementary filter, along with all modifications used in \aliasSystem.
% The only difference between \textit{AVOID} and \aliasSystem is the way they deal with magnetic distortion.
% Therefore via comparing \aliasSystem and AVOID, we prove that fundamentally modelling the distorted magnetic field provides better resistance to magnetic distortion in orientation estimation.

\subsection{}

\textbf{Original review:} 

\textit{Furthermore there are a variety of app for IOS and Android that allow researchers to log and download IMU data, including the 3D compass. I encourage the authors to do a side by side comparison of their algorithm compared to a stock smart phone and show the improvement and orientation accuracy for a clear and repeatable testing scenario.}

\textbf{Corresponding revision:}

We added a IMU hardware comparison in Section~\ref{hardware}, which compares the IMU raw readings between our smart watch, a Samsung Galaxy S21 5G, and an iPhone XS max.
Figure~\ref{compare} shows the visualized results, and statistics shows that  the sensors’ relative similarities between the smartwatch and the Samsung
Galaxy S21 are 91.91$\%$, 95.18$\%$, and 97.76$\%$, for accelerometer, gyroscope, and magnetometer respectively. 
Similarities between the smartwatch and the iPhone are 97.25$\%$ 97.34$\%$, and 98.16$\%$.
This should prove that \aliasSystem's performance can scale to other smart phone.

\begin{figure} [H] 
    \subfigure[Watch Acc.]{\includegraphics[width=0.3\linewidth]{fig/compare_watch_acc.pdf}}
    \subfigure[Samsung Acc.]{\includegraphics[width=0.3\linewidth]{fig/compare_sam_acc.pdf}}
    \subfigure[iPhone Acc.]{\includegraphics[width=0.3\linewidth]{fig/compare_apple_acc.pdf}}
    
    \subfigure[Watch Gyro.]{\includegraphics[width=0.3\linewidth]{fig/compare_watch_gyro.pdf}}
    \subfigure[Samsung Gyro.]{\includegraphics[width=0.3\linewidth]{fig/compare_sam_gyro.pdf}}
    \subfigure[iPhone Gyro.]{\includegraphics[width=0.3\linewidth]{fig/compare_apple_gyro.pdf}}
    
    \subfigure[Watch Mag.]{\includegraphics[width=0.3\linewidth]{fig/compare_watch_mag.pdf}}
    \subfigure[Samsung Mag.]{\includegraphics[width=0.3\linewidth]{fig/compare_sam_mag.pdf}}
    \subfigure[iPhone Mag.]{\includegraphics[width=0.3\linewidth]{fig/compare_apple_mag.pdf}}
    
    % \vspace{-5mm}
    
    \captionsetup{labelformat=empty}
    \caption{Sensor comparison between smart devices}
    % \vspace{-5mm}
\end{figure}

As for comparison experiments, we compare \aliasSystem with MUSE and \textit{AVOID} on the same arm motion data set.
The overall average orientation errors are 16.42°, 29.57°,and 21.67° for \aliasSystem, MUSE, and $AVOID$, respectively.
\aliasSystem has an overall improvement of 44.47$\%$ over MUSE and 24.23$\%$ over $AVOID$.
Experiments are repeatable with our data set.
(We collect data by ourselves, since online data sets rarely contain magnetically-distorted scenarios of different levels)

\subsection{}

\textbf{Original review:} 
\textit{Writing. }

\textit{While I appreciate that the authors have put a significant amount of time and effort into preparing the manuscript, there are a significant number of grammatical errors, cut-off sentences, and odd language choices that make the paper difficult and confusing to understand.}
\textit{Some examples:}

\subsubsection{}

\textbf{Original review:} \textit{In the abstract the authors state "they often regard the magnetic field distortion as a mist and take magnetometer abnormality as a random error."}
\textit{it is unclear how the authors are using the word "Mist" given that the definition of mist is: a cloud of tiny water droplets suspended in the atmosphere.}

\textbf{Corresponding revision:} This description has been removed.

\subsubsection{}

\textbf{Original review:} 
\textit{Page 1 Paragraph 3:}
\textit{"However, noise is also being integrated, causing an eternal drifting in the orientation result, making it gradually deviate from the truth."}
 \textit{definition of eternal: lasting or existing forever; without end or beginning.}

\textbf{Corresponding revision:} This sentence has been revised into: \textit{'However, any gyroscope reading error will be integrated, and the accumulated error will cause a drift in orientation estimation'}

\subsubsection{}

\textbf{Original review:} \textit{"As introduced above, they point the north and down"}

\textbf{Corresponding revision:} This description has been removed, and Figure~\ref{W&G} has been added to visualize the function of accelerometer and magnetometer measurements.

\subsubsection{}

\textbf{Original review:} \textit{"For gyroscope integration, it is a deterministic procedure, and there is not much we can do about it."}

\textbf{Corresponding revision:} This description has been removed in order to avoid misunderstanding.

\subsubsection{}

\textbf{Original review:} \textit{"Even though magnetic calibration brings CF big trouble, it is still unwise not to use it."}

\textbf{Corresponding revision:} This description has been removed in order to avoid misunderstanding.

\section{Reviewer 2 (Reviewer)}

\subsection{}
\textbf{Original review:} \textit{- Introduction includes too much details. Please focus on the high-level motivation of this work and make it concise to be within 1 page.}

\textbf{Corresponding revision:} 
We have concentrated the Introduction section and moved detailed description to related sections in later parts of the paper.
In this revision, in the Introduction, we mainly focus on the distortion problem identification and our motivation and observation to solve the magnetic distortion problem.
As for the design, we cover the high-level motivations and solution ideas in the introductions and do not discuss much on detailed information and experiments, while they are still available in later sections like Design~\ref{design} and \ref{pro}, and Evaluation~\ref{sec_evaluation}.

\subsection{}
\textbf{Original review:} \textit{- In introduction, the flow of writing, MUSE says that magnetometer can be trusted more than accelerometer. But then, in the next paragraph, authors say that magnetic field distortion makes magnetic filed not trustworthy. This is explained much later in the paragraph. Please elaborate more here regarding this contradicting statements.}

\textbf{Corresponding revision:} 
MUSE does not specifically consider the magnetic distortion issue in their design, but did identify it in their paper. 
In this revision, we changed the sentence into: \textit{'However, MUSE ignores magnetic distortion that commonly exists in buildings'}.
Following the introduction of MUSE, we introduce the magnetic distortion, which hopefully would provide better explanation.

\subsection{}

\textbf{Original review:} \textit{- Bold character is used too often. Please only use few times that needs most emphasis across the manuscript.}

\textbf{Corresponding revision:}
We have cleared most of the bold characters.
It now only appears as sub-sub-section titles or the names of baselines for evaluation.

\subsection{}

\textbf{Original review:} \textit{- Section 2 Background contains important but basic information on orientation and complementary filter, which is well known and established in IMWUT community. }

\textit{Thus, I suggest moving this section into entirely as Appendix, and authors can assume the readers who are interested in this work already is equipped with those backgrounds.}

\textbf{Corresponding revision:}
Background section is now Section~\ref{secBackground} in this revision.
In Section~\ref{secBackground}, we only kept necessary information and briefly introduce complementary filter for orientation estimation and particle filter for location estimation.

\subsection{}
\textbf{Original review:} \textit{- Section 3.2 where does this error comes from? Is the author referring to the motion drift noise from accelerometer? Please clarify.}

\textbf{Corresponding revision:}
Error in accelerometer measurement direction (if we assume it should point to the direction of gravity) mainly come from the linear acceleration.

Section 3.2 in the previous submission introduced the error in calibration via accelerometer.
However, we decided to remove Section 3.2 in the previous submission, since we want to focus on error in magnetometer calibration, and error in accelerometer calibration is somewhat irrelevant to the main topic.

\subsection{}
\textbf{Original review:} \textit{- Section 3.3 includes too much details. As the section 3 says, please focus on discussing motivations. move 3.3 to later experiment part after discussing the proposed methodologies.}

\textit{- In figure 10, is the small orientation error coming from horizontal (x, y) orientation? what about the orientation error from vertical (z) movement that is most related to gravity direction? Please correct y-axis of the graph to horizontal orientation error, if this is the case.}

\textit{- Experiment implementation in 3.3 needs to be explained before showing the results to help read understand how those results are derived first. Regardless, I consider 3.3 needs to be discussed later in the experiment section, and use this space solely on motivations.}

\textit{- I consider the authors are only considering horizontal orientation where magnetometer is more relevant compared to accelerometer. But overly claiming as if full 3D orientation is affected only by magnetometer. The entire motivation here sounds invalid without clarification regarding the vertical orientation that will be most influenced by the errors in gravity direction from accelerometer which is also pretty huge up to ~25 degrees.}

\textbf{Corresponding revision:}
Section 3.3 'Comparison Between the Two Errors' from the previous submission is now Section~\ref{muse in distortion} in this revision.
Since we have discarded the analysis on accelerometer error, we no longer compare the two errors, i.e. accelerometer and magnetometer errors.
We kept the important part of this subsection: the experiment on magnetic distortion's impact on orientation estimation, which is now Section~\ref{muse in distortion}.
We change the tested algorithm from the classical complementary filter to MUSE, and test it under different distortion levels to demonstrate the impact of magnetic distortion on orientation estimation.

Figure 10 in the previous submission refers to the total 3-D orientation error, and the small difference in the error of complementary filter (CF) comes from increased accelerometer error.
It appears to be small since the other curve's value is too large, and thus expands the scale of y-axis.
However, we have also decided to remove this experiment and Figure 9 and 10, since they are not highly related to magnetic distortion.
In this revision, we only kept the highly related part: Section~\ref{muse in distortion}, in which we test MUSE under different distortion levels to demonstrate the impact of magnetic distortion on orientation estimation.
Figure~\ref{muse_devM} shows the corresponding result of MUSE, and is also shown below:

\begin{figure}[tbp]
    % % \vspace{-0.3cm}
    \begin{minipage}[t]{0.3\linewidth}
        \centering
        \includegraphics[width=\textwidth]{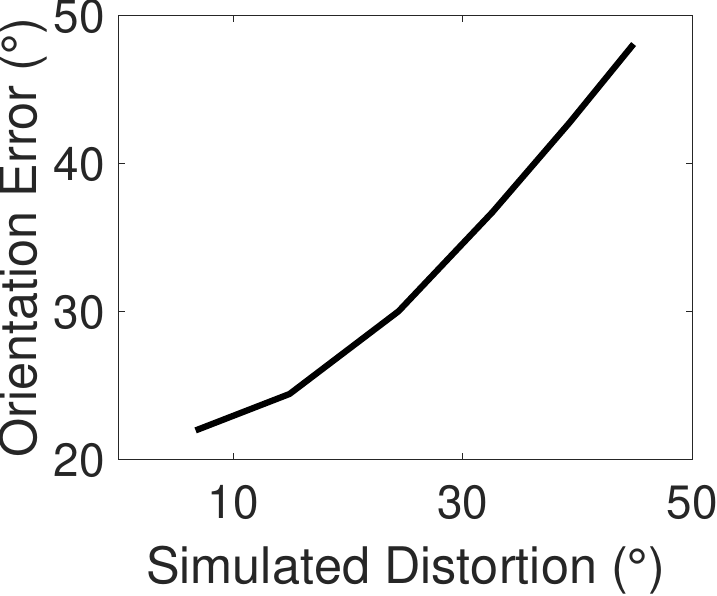}
         % % \vspace{-7.5mm}
        % \caption{Impact of different magnetic distortion levels.}
        \captionsetup{labelformat=empty}
        \caption{Impact of magnetic distortion on MUSE.}
        % % \vspace{0cm}
        % \label{muse_devM}
    \end{minipage}
    % \hspace{0.1cm}
    % \begin{minipage}[t]{0.46\linewidth}
    %     \centering
    %     \includegraphics[width=\textwidth]{fig/mobi_chrono.pdf}
    %      % \vspace{-7.5mm}
    %     \caption{Temporal stability of magnetic field.}
    %     % % \vspace{0cm}
    %     \label{temporal}
    % \end{minipage}
    % % \vspace{-4mm}
\end{figure}

\subsection{}

\textbf{Original review:} \textit{- I consider Section 1 intro and section 3 can be combined and reduced down to 1 page with concise and get-to-the-point motivation and moving any details and analysis to the later points.}

\textbf{Corresponding revision:} 
Section 3 in the previous submission was the motivation section, which is now Section \ref{secMotivation} in this revision.
Comparing to Section 3 in Section \ref{secMotivation}'s length has been largely reduced, as we mainly discuss magnetometer and magnetic distortion related information and experiments, and have omitted the accelerometer related introductions, as they are not highly relevant to the main topic.
However, there are still accelerometer related discussion in Section \ref{pro}, where we focus on improving orientation and location accuracy based on necessary discovery and experiments on accelerometer usage.

\subsection{}

\textbf{Original review:} \textit{- For section 4 system design, I would suggest introducing the final system design and discuss the previous versions as a part of ablation study and how the model behavior and system overhead differs. Being this said, I suggest only keeping 4.5.4 and relevant part of the system in other subsections, and move everything else to the ablation analysis section in the later part.}

\textbf{Corresponding revision:}
We thoroughly re-organized the Design section (Section~\ref{design} in this revision).
In the previous submission, we introduce \aliasSystem in different versions (e.g. $MDR_L+D$, $MDR_D$, $MDR$, $MDR+$), which were probably hard to understand.
In this revision, for better understanding, we name the full system design as \aliasSystem, and cancelled all other version names in the design section.
We introduce the key design of \aliasSystem and its database in Section~\ref{selfDB} (corresponding to $MDR_L+D \rightarrow MDR_D \rightarrow MDR$ in the previous submission)
Specifically in Section~\ref{selfDB}, we proposed a new design named Adaptive Updating, introduced in Section~\ref{adaptive_updating}, which was not included in the previous submission.
In Section~\ref{pro}, we introduce the design of reducing errors in database operations (corresponding to $MDR \rightarrow MDR+$ and subsection 'Improving Database Usage' in the previous submission)

As for the ablation study, in Section~\ref{decompose} we decompose the design of \aliasSystem to demonstrate the performance contribution of each design component.
In this revision, for better understanding, we listed the decomposed baselines in Section~\ref{decompose_baselines}:

\begin{itemize}
    \small
    \item \textit{\textbf{CF:}} \aliasSystem with neither database nor error-reduction, namely a classical complementary filter.
    \item \textit{\textbf{\aliasSystem w/o DB:}} \aliasSystem with the error-reduction designs, but without database.
    \item \textit{\textbf{\aliasSystem w/o ER:}} \aliasSystem with database, but no error-reduction.
    \item \textit{\textbf{\aliasSystem:}} Complete \aliasSystem with database and error-reduction.
    % with both database and error-reduction.
\end{itemize}

We no longer include $MDR_L+D$ and $MDR_D$ from the previous submission, as only the performance of \aliasSystem and its components matters.
Experiment results show that the error-reduction design (Section~\ref{pro}) improves database usage, and lifts the relative improvement via database from 17.18$\%$ to 25.30$\%$.
This demonstrates the co-effect of database design (Section~\ref{design}) and error-reduction design (Section~\ref{pro}), and verifies that error-reduction improves database operation.
Additionally in this revision, we added performance decomposition on adaptive updating~\ref{eval_adaptive_updating}, in order to evaluate our new design component: adaptive database updating (Section \ref{adaptive_updating}).

Specifically, we compare \aliasSystem with a sub-baseline of \aliasSystem without adaptive updating scheme (denoted as \textbf{\aliasSystem w/o AU}), which naively pile the anchors into datapoints, as shown in Equation \ref{Fupdate}.
% instead of adaptive updating shown in Equation \ref{Fupdate3}.
We use the baselines to run complete data traces.
After that, we record the final database error, namely the average direction error of all anchors stored in the database.
% As shown in Figure \ref{eval_au}, 
Average final database error of \aliasSystem is 12.04°, which is 9.13$\%$ lower than the 13.25° of \textbf{\aliasSystem w/o AU}.
This verifies the capability of refining database accuracy of the adaptive updating scheme.

\subsection{}

\textbf{Original review:} \textit{- From figure 13, MDR{L+D} looks to have lowest error. I consider this is from the external localization and prepared database. I consider the major difference should be between MDR, CF, MDR+ which does not use extra system overhead. I would explicitly mention in the caption so that readers can better understand this figure in a first glance.}

\textbf{Corresponding revision:}
Indeed, $MDR_{L+D}$ had the advantage of external localization and prepared database, and thus had the lowest error.
If we would draw Figure 13 again, we would mention the major difference.
However, $MDR_{L+D}$, along with $MDR_{D}$ no longer exist in this new revision, as we introduce the design with no extra system overhead in the first place, i.e. \aliasSystem, thus cancelling the long story line that could cause misunderstanding.

In the previous submission, Figure 13 demonstrates the performance of different baselines under different levels of distortion.
In this revision, it is Figure~\ref{result}, which also shows the performance of different baselines under different levels of distortion, but the baselines are different: 
In this revision, we mainly compare \aliasSystem with a more meaningful baseline: the current state-of-the-art orientation estimation method MUSE~\cite{muse}, which also uses complementary filter as basis.
Additionally we included a custom baseline named \textit{AVOID}, via taking the idea from \cite{fan2017adaptive,ahrs}, i.e. to reduce magnetometer usage when magnetic distortion is severe, therefore avoiding its negative impact (Section~\ref{baselines}).
% We mainly refer to the strategy from the later work~\cite{fan2017adaptive}, and incorporate it into a complementary filter, with all modifications used in \aliasSystem, except the database design of \aliasSystem, so that the only difference between \textit{AVOID} and \aliasSystem is the way they resist magnetic distortion.
% Later in Evaluation we compare \aliasSystem and AVOID, which proves that fundamentally modelling the distorted magnetic field via a database provides stronger resistance to the distortion (Section~\ref{eval_distortion}).

\subsection{}

\textbf{Original review:} \textit{- Section 4.3.1 particle filter is a very standard tracking method, which many in imwut community are aware of. I will move this section to appendix, and describe system design assuming that this is known by the reader.}

\textbf{Corresponding revision:}

We have largely reduced the length of introduction of particle filter used for location estimation.
Background section is now Section~\ref{secBackground} in this revision.
In Section~\ref{secBackground}, we only kept necessary information and briefly introduce complementary filter for orientation estimation and particle filter for location estimation.

\subsection{}
\textbf{Original review:} \textit{- I suggest moving any performance evaluation and related figures and dataset description to later part, and purely focus on describing the system design in Section 4.}

\textbf{Corresponding revision:}
The half-way design, $MDR_{L+D}$ and $MDR_{D}$ no longer exist in this new revision, and we now introduce the design with no extra system overhead in the first place, i.e. \aliasSystem.
% thus cancelling the long story line that could cause misunderstanding.
Therefore there is no longer half-way evaluation anymore in the design section (Section~\ref{design}).
The design part (Section~\ref{design} and \ref{pro}) now consists of overview~\ref{DB}, query~\ref{deadlock}, updating~\ref{selfDB}, workflow~\ref{workflow}, and error-reduction design~\ref{pro}.
All design components have their corresponding experiment in the evaluation.
The data collection content has also been concentrated into Section~\ref{data}.

We kept all experiments from previous submission evaluation, including experiments on overall performance~\ref{eval_overall}, different users~\ref{eval_users}, different places~\ref{pla}, different distortion levels~\ref{eval_distortion}, performance decomposition~\ref{decompose}, impact of database resolution~\ref{secDatabaseResolution}, database construction efficiency (Section~\ref{DBeval}), latency (Section~\ref{computation latency}), and memory cost~\ref{eval_memory}.
In this revision, we added performance decomposition on adaptive updating~\ref{eval_adaptive_updating}, in order to evaluate our new design component: adaptive database updating (Section \ref{adaptive_updating}).
We also examined location estimation accuracy in Section~\ref{eval_loc}.
% as it is one important factor in arm tracking and activity recognition.
% We also revised the evaluation on analysis on database construction efficiency (Section~\ref{DBeval}).
% In Figure~\ref{build up}, beside the old curve 'Database Size', we added another curve 'Database Error', which demonstrates that the database refines its accuracy over time, indicating \aliasSystem's reliability in self-exploring new scenarios.
% Additionally in the latency section (Section~\ref{computation latency}), we conducted new real experiment, in which we migrated \aliasSystem onto the Iphone XS Max and tested \aliasSystem's computation latency. 
% Result shows, for every 1 second, \aliasSystem can process data of 3.37 seconds, demonstrating its real-time capability on mobile platform.
All experiments are re-conducted with new designs and an extra portion of newly collected data.

\subsection{}
\textbf{Original review:} \textit{- In section 4.4, MDR can run in real-time? generating database, tracking, and estimating orientation at the same time?}

\textbf{Corresponding revision:}
\aliasSystem can run in real-time as it executes complementary filter, particle filter, and database operations all together.
In this revision, in the latency section (Section~\ref{computation latency}), we conducted new real experiment, in which we migrated \aliasSystem onto the Iphone XS Max and tested \aliasSystem's computation latency. 
Result shows, for every 1 second, \aliasSystem can process data of 3.37 seconds, demonstrating its real-time capability on mobile platform.

\begin{figure} [H]
    \centering
    \hspace{-7mm}
    \includegraphics[width=0.7\linewidth]{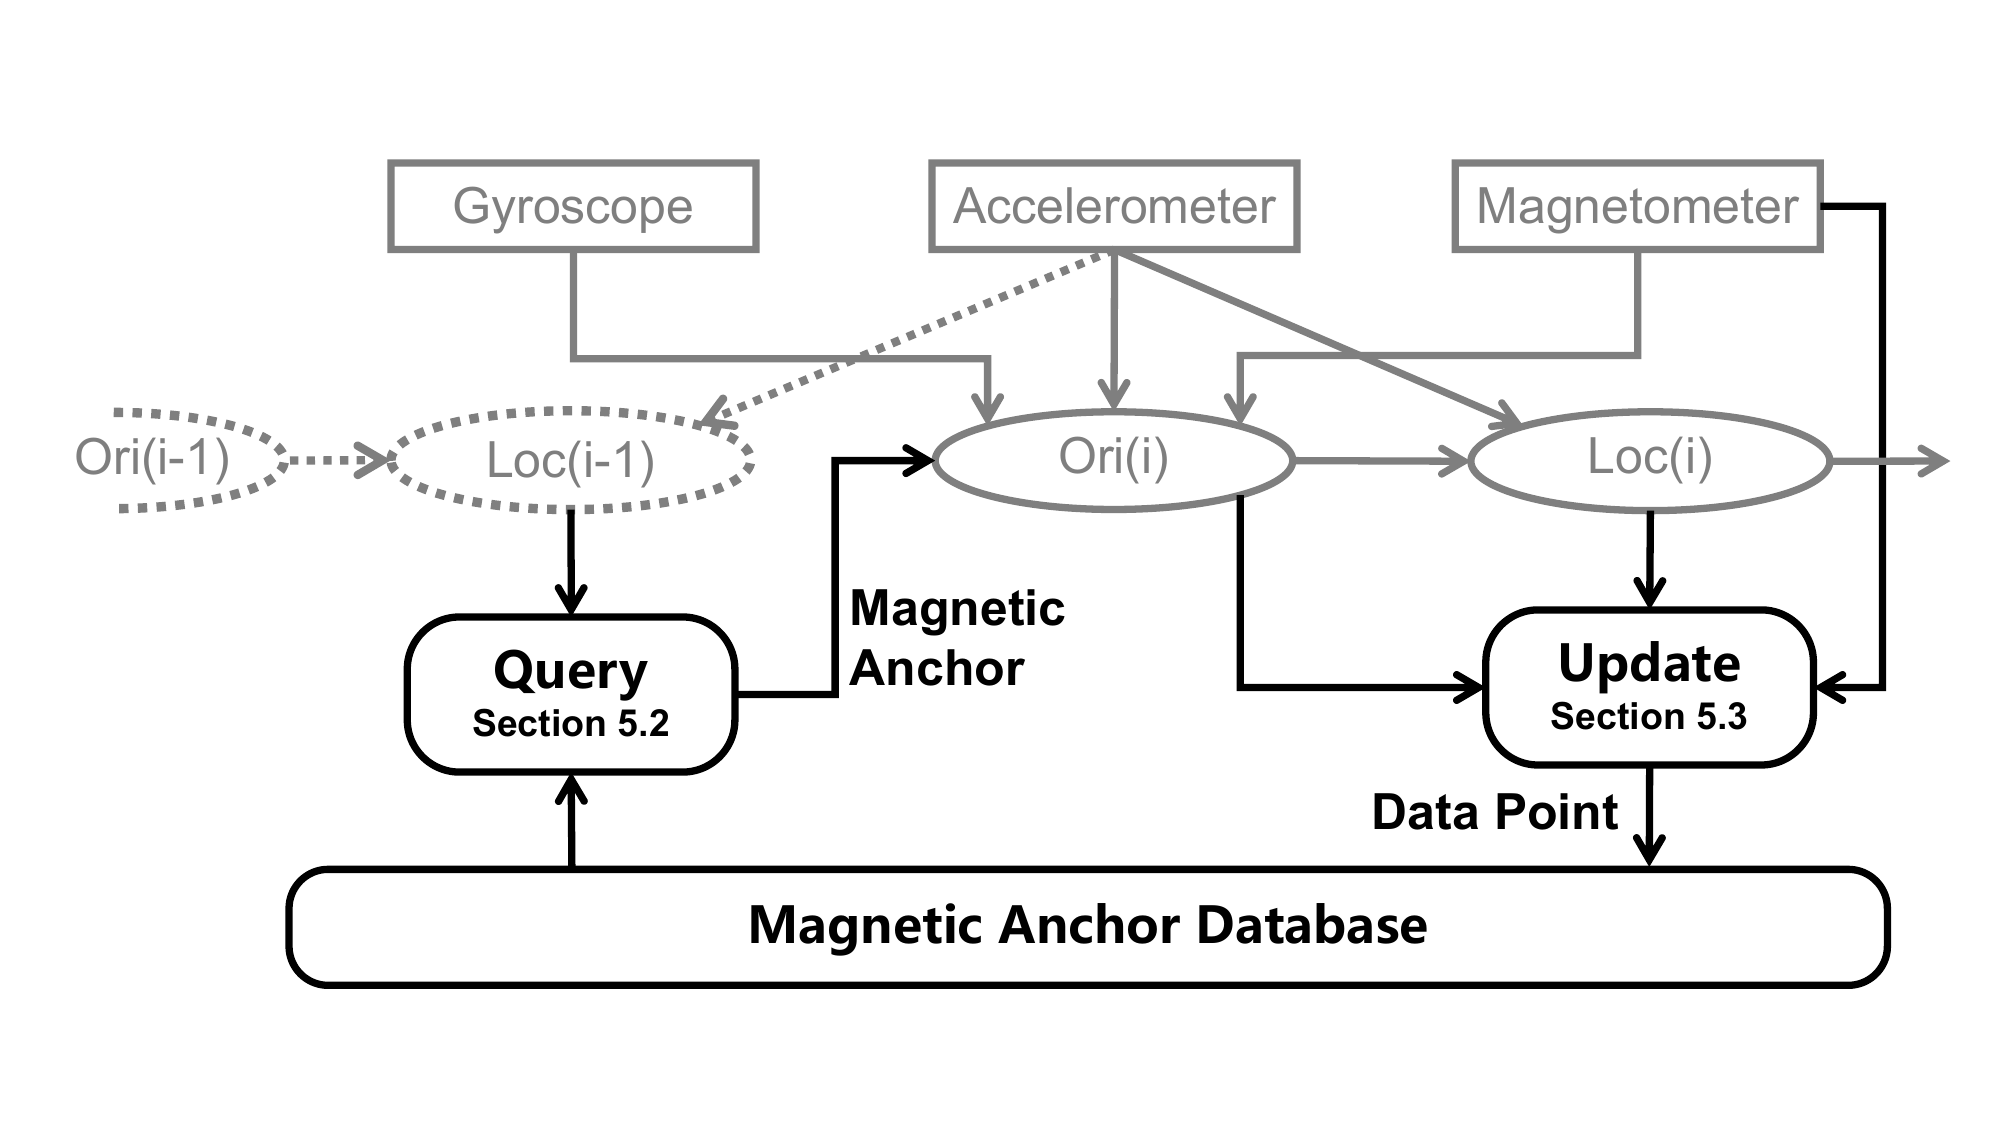}
    % % \vspace{-3.5mm}
    \captionsetup{labelformat=empty}
    \caption{MDR System Workflow.}
    % \label{flow}
    % \vspace{-5mm}
\end{figure}

\subsection{}

\textbf{Original review:} \textit{- There is no blue arrows in figure 16. I think the pdf supposed to have color, which is missing in the submitted manuscript.}

\textbf{Corresponding revision:}
% We are sorry about this terrible mistake.
Figure 16 workflow from the previous submission is now Figure~\ref{flow}, which uses black and white only.
In Figure~\ref{flow}, we have also re-organized flow chart topology and simplified representations, for better understanding.
We added the names of the key design components into the work flow, i.e. query and update, and marked the corresponding sections, in which they are introduced.

\subsection{}

\textbf{Original review:} \textit{- how do you determine K{cali} and K{gyro} in the real-world scenario when using new IMU sensors for other kinds of arm motions?}

\textbf{Corresponding revision:}
$K_{cali}$ and $K_{gyro}$ were introduced in Section 4.5.2 in the previous submission.
They are now $K_c$ and $K_g$ in Section~\ref{boost_ori_2} in this revision.
They control the frequency of using accelerometer+magnetometer calibrations and the frequency of gyroscope integration, respectively.
We have conducted real experiment on the smart watch's IMU sensors, and set $K_{c}=24$ and $K_{g}=1$.
The result is shown in Figure~\ref{kk}, and also shown below:

\begin{figure} [H]
    \centering
    \hspace{-0.3cm}
    % \vspace{-0.2cm}
    \includegraphics[width=0.5\linewidth]{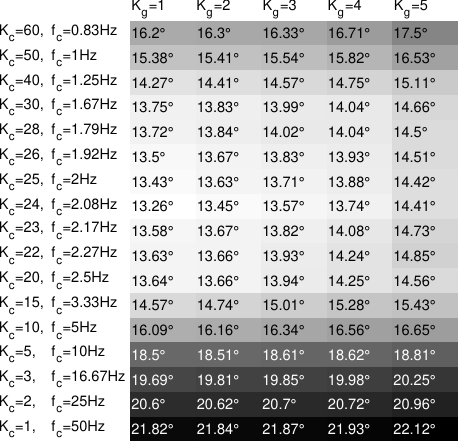}
    % \vspace{-1mm}
    \captionsetup{labelformat=empty}
    \caption{Orientation error with different gyroscope integration frequency $K_g$ and calibration frequency $K_c$.}
    % \vspace{-5mm}
    % \label{kk}
\end{figure}

However, we think $K_{c}$ and $K_{g}$ are related to the sensor noise nature.
If the system is to scale to other IMU sensors, $K_{c}$ and $K_{g}$ may need to be re-determined to their best setting.
This experiment is meant to demonstrate an insight that it may not be best to set $K_{c}=1$.

\subsection{}

\textbf{Original review:} \textit{- In section 5.2, I suggest including figure examples for the motion taken and rooms for data collection.}

\textbf{Corresponding revision:} 
For the data collection, we invite 12 users to collect 100+ data traces, at 10 different places, in 2 different cities, with a total duration of 27+ hours.
Each data trace is around 10 $\sim$ 20 minutes. 
At the beginning of each data trace, the user stands still for 10 seconds, so that the system can initialize the GRF.
During the data collection, the user performs daily arm motion, such as:
\begin{itemize}
    \item Point to front, left, and right.
    \item Draw straight lines
    \item Write letters in air, from 'A' to 'Z'.
    \item Exercising, e.g. lift dumbbells.
    \item Stay still and rest.
\end{itemize}
To better simulate daily arm movement, we allow the users to perform the above activities in any order.
Users may sometimes perform customized arm motion, which is also recorded in the data traces, so that they can better simulate more complex daily activities.
Here is a figure on the data collection demo: 

\begin{figure} [H]
    \centering
    \includegraphics[width=0.4\linewidth]{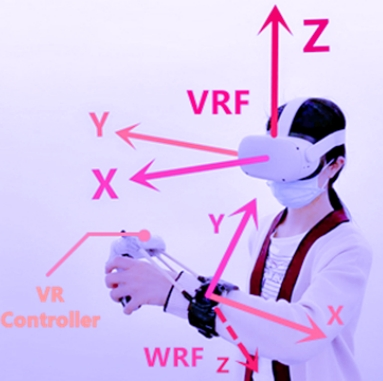}
    \captionsetup{labelformat=empty}
    \caption{Data collection}
    % \label{fig:enter-label}
\end{figure}

The user wears a VR headset and a VR controller, for ground truth data collection.
The VR is not required during the independent online inference of \aliasSystem, as the inputs, i.e. IMU sensors, are all integrated within the smart watch.

\subsection{}

\textbf{Original review:} \textit{- If the performance varies by the motion speed or arm length, I suggest users include the correlation graph speed/arm length vs error for the clarity. Fig 23 shows the individual differences, but does not show this important factor. And more systematic analysis will demonstrate the break point of the proposed system that will provide very useful intuition on deployment scenario across varying users.}

\textbf{Corresponding revision:}
% Figure \ref{users} shows the average orientation error on different users' data. 
% Performance of \aliasSystem is better than both baselines among all users.
In this revision, we analyze the performance of the baselines on different users' data in Section~\ref{users}, via look into the accelerometer error in their data.
Different users may have different error, depending on the user's motion pattern, which mainly affects the accelerometer accuracy.
We take two users as example.
User D's arm moves fast, having an average accelerometer direction error of 16.72°, while user H moves slowly and has an average accelerometer direction error of 7.79°.
As a result, the overall orientation error on user D is higher than user H.
The users evaluation Figure is attached below:

\begin{figure} [H]
    % \hspace{-0.1cm}
    \centering
    % % \vspace{-2cm}
    \includegraphics[width=0.59\linewidth]{fig/sensys_eval_user.pdf}
    % % \vspace{-4mm}
    \captionsetup{labelformat=empty}
    \caption{Performance among different users.}
    % \label{users}
    % % \vspace{-3mm}
\end{figure}

We also plot an extra figure on the relationship between the accelerometer direction error (°) and the final orientation error (°) of \aliasSystem, as shown below:

\begin{figure}[H]
    \centering
    \includegraphics[width=0.35\linewidth] {fig/ubi_acc_ori.pdf}
    \captionsetup{labelformat=empty}
    \caption{Relationship between accelerometer error and orientation error}
    % \label{fig:enter-label}
\end{figure}

Every dot in the figure represents one data trace.
We can see as accelerometer direction increases, the lower bound of the overall error also increases, since the accelerometer direction serves as a direct input of sensor fusion.
However, it is hard to quantify the overall orientation error simply based on accelerometer error, mainly due to the existence of magnetometer error presence.

\subsection{}

\textbf{Original review:} \textit{- Section 6.1: although briefly discussed in 5.8, 5.9, 5.10, providing actual numbers on the reduction of computation, memory, time lag between CF, MDR, MDR+ should help to understand the impact of this analysis.}

\textbf{Corresponding revision:}

Section 6.1 in the previous submission identifies the Distortion-Free cases.
When distortion is determined to be low (<10°) \aliasSystem will shut down the database function, along with particle filter that supports database with location estimation.
According to Table~\ref{latency}, particle filter consumes the most computation resources: 87$\%$, while complementary filter takes 10$\%$ and database takes less than 3$\%$.
Therefore distortion-free detection module could save 90$\%$ of computation latency when distortion is low.
It basically degrade MDR+ to CF, and MDR+ shares the same computation latency performance with MDR.
However, we removed the distortion-free detection part in this revision as it is not related to our main topic, i.e. 'handling distortion'.

\begin{table} [H]
    \centering
        \captionsetup{labelformat=empty}
        \caption{Latency of major components in \aliasSystem.}
         % \vspace{-4mm}
    \begin{tabular}{|l|c|c|c|}
        \hline
         Component & Complem. F. & Particle F. & Database \\
         \hline
         Relative latency & 10.05$\%$ & 87.08$\%$ &  2.87$\%$ \\
         \hline
    \end{tabular}
    % \vspace{-2mm}
    % \label{latency}
\end{table}

\subsection{}

\textbf{Original review:} \textit{- Section 6.5 can be included in the introduction section or as a footnote where first Magnetic Field Intensity is introduced.}

\textbf{Corresponding revision:}
We use standard terms in this revision, thus terminology correction is no longer need.
Therefore we have removed Section 6.5 Terminology Correction in this revision, and hopefully could avoid unnecessary misunderstanding.

%%%%%%%%%%%%%%%%%%%%%%%%%%%%%%%%%%%%%%%%%%%%%%%%%%%%%%%%%%

\section{Reviewer 3 (Reviewer)}

\subsection{}

\textbf{Original review:} \textit{2.1, the authors claim that their work is the first to fundamentally model and resist magnetic field distortion in orientation estimation. However, the same/similar topic has been explored by other works, like:
“An Adaptive Orientation Estimation Method for Magnetic and Inertial Sensors in the Presence of Magnetic Disturbances”, where the proposed orientation estimation system performs online detection and compensation for magnetic disturbances, and also the work
“Accurate Orientation Estimation Using AHRS under Conditions of Magnetic Distortion”, where an adaptive method to improve the accuracy of orientation estimations in the presence of magnetic disturbances is proposed.
So be careful with the words ”the first” or the described subject following it.}

\textbf{Corresponding revision:}
We have looked into the two works and implemented into experiment for comparison:
“An Adaptive Orientation Estimation Method for Magnetic and Inertial Sensors in the Presence of Magnetic Disturbances” \cite{fan2017adaptive}.
“Accurate Orientation Estimation Using AHRS under Conditions of Magnetic Distortion” \cite{ahrs}.

Specifically, we included a custom baseline named \textit{AVOID}, via taking the idea from \cite{fan2017adaptive,ahrs}, i.e. to reduce magnetometer usage when magnetic distortion is severe, therefore avoiding its negative impact.
We mainly refer to the strategy from the later work~\cite{fan2017adaptive}, and incorporate it into a complementary filter, with all modifications used in \aliasSystem, except the database design of \aliasSystem, so that the only difference between \textit{AVOID} and \aliasSystem is the way they resist magnetic distortion.
Later in evaluation (Section~\ref{eval_distortion}) we compare \aliasSystem and AVOID, which proves that fundamentally modelling the distorted magnetic field via a database provides stronger resistance to the distortion (Section~\ref{eval_distortion}).
\aliasSystem is not the first that tries to resist magnetic distortion in orientation estimation.
However, in this work we study the solution of 'fundamentally model magnetic field distortion in orientation estimation', and the experiment in Section~\ref{eval_distortion} verifies the distortion resistant capability of \aliasSystem.
Figures of the experiments are attached below:

\begin{figure} [H]
    % % \vspace{-0.2cm}
    \hfill
    \begin{minipage}[t]{0.50\linewidth}
        % \hspace{-1mm}
        \centering
        % % \vspace{-2cm}
        \includegraphics[width=1\linewidth]{fig/sensys_eval_overall.pdf}
        \captionsetup{labelformat=empty}
        % % \vspace{-4mm}
       \caption{Overall orientation error comparison between baselines.}
        % \label{overall}
        % % \vspace{-4mm}
    \end{minipage}
    \hfill
    \begin{minipage}[t]{0.40\linewidth}
        \centering
        % % \vspace{-0.1cm}
        \includegraphics[width=1\linewidth]{fig/sensys_eval_dev.pdf}
        \captionsetup{labelformat=empty}
        % % \vspace{-7mm}
        \caption{Orientation error of the baselines at different magnetic distortion levels.}
        % \label{result}
    \end{minipage}
    \hfill
    % % \vspace{-4mm}
\end{figure}

\subsection{}

\textbf{Original review:} \textit{And please eliminate unnecessary adjectives and adverbs. Like the word “greatly”, which is not quantitative and therefore does not clarify the writing.}

\textbf{Corresponding revision:}
We have thoroughly revised the paper and its writing, and have removed most of the non-quantitative descriptions.
In this revision, we focus on concise introduction on the system and its workflow, with plain language.

\subsection{}

\textbf{Original review:}
\textit{Rewrite related work with the more close topic, namely the magnetic field distortion approaches presented by other works.}

\textit{2.2 The related works (mostly related to distortion itself, fingerprinting for positioning) mentioned in the manuscript are not representative and close to the subject. It is highly recommended to cite works more related to addressing the magnetic field distortion and make comparisons to the state-of-the-art or different approaches for the solutions.}

\textbf{Corresponding revision:}
In this new version, we have thoroughly revised Section~\ref{related}: Related Work.
Since our system is closely related to the fingerprinting technique for localization, we hope to use the Related Work section to identify our position relative to that.
Specifically, Section~\ref{related} include three major parts: Magnetic Fingerprint, IMU-based Orientation Estimation, and Magnetic Distortion in Orientation Estimation.

We first discuss the magnetic fingerprinting technique used in localization, as it is closely related with \aliasSystem's magnetic anchor database design.
We justify that the way \aliasSystem uses magnetic anchor database is different from magnetic fingerprint.
Moreover, we discuss that the spatial resolution requirement for magnetic anchor database for orientation estimation is higher than magnetic fingerprint for localization, and based on which, we argue that the database preparation overhead is greater.
That is where the Automatic Updating (Section~\ref{selfDB}) design of \aliasSystem comes in to reduce the overhead of database preparation.

Next, we briefly introduce the related works in IMU-based orientation estimation. 
We identify MUSE~\cite{muse} as the state-of-the-art orientation estimation method, inspired by which, we also adopt a complementary filter for orientation estimation.
We then discuss the current researches that deal with magnetic distortion in orientation estimation (\cite{fan2017adaptive,ahrs}).
We argue that, although they reduce the negative impact of magnetic distortion to a certain extent, they do not fundamentally model the distorted magnetic field. 
Therefore they fail to resist distortion when it is high (as to be verified in Section~\ref{eval_distortion}).
As comparison, \aliasSystem uses a magnetic anchor database to model the magnetic field to resist distortion, and thus has better resistance performance.

\subsection{}

\textbf{Original review:} \textit{2.3 Orientation estimation is mostly used in edge scenarios. Regarding the latency (1.43s for 60s/50hz data) and memory footprint(678Kb for one cubic meter database) of the proposed method, which is obviously not acceptable for a real-time or timely orientation update on edge devices that has very limited hardware resources and power budget. A detailed power and latency estimation of the proposed different solutions on different platforms could be described in order to show readers the potential of the approach in practical usage.}

\textit{2, Either remove the subsection on latency and memory or provide sufficient calculation results regarding latency and memory. Since orientation estimation is more deployed on edge devices with very limited hardware resources and power budget in practical scenarios, if the authors want to cover this subtopic in the current manuscript, more detailed results are needed, like the memory footprint, power consumption, and latency on different hardware edge platforms.}

\textbf{Corresponding revision:}
In the previous submission, Section 5.9 evaluates the latency of \aliasSystem+: \textit{'According to the overall experiments, MDR+ requires 1.43 s to process one-minute 50 Hz IMU readings,'}.
That experiment was conducted with Matlab on a laptop, but this time we conducted real experiment on real mobile platform.
In this revision, in the latency section (Section~\ref{computation latency}), we conducted new real experiment, in which we migrated \aliasSystem onto the IPhone XS Max and tested \aliasSystem's computation latency. 
Result shows, for every 1 second, \aliasSystem can process data of 3.37 seconds, demonstrating its real-time capability on mobile platform.
On the mobile platform (i.e. the IPhone XS Max), \aliasSystem can run in real-time as it executes complementary filter, particle filter, and database operations all together.
As for the case where a smart watch is used as IMU sensor platform, it could transmit raw IMU data to a smart phone for data processing via Bluetooth, and could also reach real-time.
We also refined the storage of the database (avoiding wasting memory for empty datapoints in the cube matrix, which we did not explicitly mention in the paper, since this is a comparison between the previous submission and this revision), and examined the memory cost on the mobile smart platform (i.e. the IPhone XS Max) in this revision.
In Section~\ref{eval_memory}, result shows that with the current implementation, 21.63KB is needed for every 1$m^3$ database with 0.1m resolution.

\subsection{}

\textbf{Original review:} \textit{3, Since the location information will be used both in the updating process and query process of the database. It would be better to explain why the particle filter is used and to show also what's the result of the location in real-life experiments compared with the state-of-the-art.}

\textbf{Corresponding revision:}
In this revision, in Section~\ref{particle}, we introduce particle filter, and that \aliasSystem follows the state-of-the-art arm tracking solution MUSE, and adopts particle filter to estimate the device's location.

We examined location estimation accuracy in Section~\ref{eval_loc}, as it is one important factor.
We compare \aliasSystem with MUSE.
The result shows that \aliasSystem has an average error of 0.1083m, 20.60$\%$ lower than the existing state-of-the-art solution, MUSE (0.1364m).

\begin{figure}[H]
    \begin{minipage}[t]{0.6\linewidth}
        % \hspace{-0.1cm}
        \centering
        % % \vspace{-2cm}
        \includegraphics[width=1\linewidth]{fig/sensys_localization.pdf}
        % % \vspace{-7mm}
        \captionsetup{labelformat=empty}
       \caption{Overall location accuracy of \aliasSystem and MUSE.}
        % \label{localization}
    \end{minipage}
    % % \vspace{-3mm}
\end{figure}

%%%%%%%%%%%%%%%%%%%%%%%%%%%%%%%%%%%%%%%%%%%%%%5

\section{Reviewer 4 (Reviewer)}

\subsection{}

\textbf{Original review:} \textit{1. quantitative comparison with the SOTA.
The comparison to the state of the art (SOTA) is insufficient. The reported performance is compared against the baseline algorithm of complimentary filters - which I believe is not being actually used currently. There are many other algorithms as the authors also pointed to in 7 related work. But there is no quantitive comparison, especially this work's main contribution is incremental performance in a very classic domain with the novel distortion database. For the paper to have better impact, there should be a more quantitive comparison (preferably in the form of a table), to show the readers how much performance gain the proposed work demonstrates compare with the SOTA.}

\textbf{Corresponding revision:}

We expanded the Evaluation section with more baselines for comparison.
In the previous submission, we only compared \aliasSystem with classical complementary filter (CF), while in this revision, we mainly compare with a more meaningful baseline: the current state-of-the-art orientation estimation method MUSE~\cite{muse}, which also uses complementary filter as basis.
Additionally we included a custom baseline named \textit{AVOID}, via taking the idea from \cite{fan2017adaptive,ahrs}, i.e. to reduce magnetometer usage when magnetic distortion is severe, therefore avoiding its negative impact.
We mainly refer to the strategy from the later work~\cite{fan2017adaptive}, and incorporate it into a complementary filter, with all modifications used in \aliasSystem, except the database design of \aliasSystem, so that the only difference between \textit{AVOID} and \aliasSystem is the way they resist magnetic distortion.
Later in evaluation (Section~\ref{eval_distortion}) we compare \aliasSystem and AVOID, which proves that fundamentally modelling the distorted magnetic field via a database provides stronger resistance to the distortion (Section~\ref{eval_distortion}).

Experiment result (Section~\ref{eval_overall}) shows that the overall average orientation errors are 16.42°, 29.57°,and 21.67° for \aliasSystem, MUSE, and $AVOID$, respectively.
The figure for the experiment is attached below:

\begin{figure} [H]
    % % \vspace{-0.2cm}
    \hfill
    \begin{minipage}[t]{0.50\linewidth}
        \hspace{-1mm}
        \centering
        % % \vspace{-2cm}
        \includegraphics[width=1\linewidth]{fig/sensys_eval_overall.pdf}
        \captionsetup{labelformat=empty}
        % \vspace{-4mm}
       \caption{Overall orientation error comparison between baselines.}
        % \label{overall}
        % \vspace{-4mm}
    \end{minipage}
    \hfill
    \begin{minipage}[t]{0.40\linewidth}
        \centering
        % % \vspace{-0.1cm}
        \includegraphics[width=1\linewidth]{fig/sensys_eval_dev.pdf}
        \captionsetup{labelformat=empty}
        % \vspace{-7mm}
        \caption{Orientation error of the baselines at different magnetic distortion levels.}
        % \label{result}
    \end{minipage}
    \hfill
    % \vspace{-4mm}
\end{figure}

\aliasSystem has an overall improvement of 44.47$\%$ over MUSE and 24.23$\%$ over $AVOID$.
We also examined location estimation accuracy in Section~\ref{eval_loc}, as it is one important factor.
We compare \aliasSystem with MUSE.
The result shows that \aliasSystem has an average error of 0.1083m, 20.60$\%$ lower than the existing state-of-the-art solution, MUSE (0.1364m).

\begin{figure}[H]
    \begin{minipage}[t]{0.6\linewidth}
        % \hspace{-0.1cm}
        \centering
        % % \vspace{-2cm}
        \includegraphics[width=1\linewidth]{fig/sensys_localization.pdf}
        % % \vspace{-7mm}
        \captionsetup{labelformat=empty}
       \caption{Overall location accuracy of \aliasSystem and MUSE.}
        % \label{localization}
    \end{minipage}
    % \vspace{-3mm}
\end{figure}

\subsection{}

\textbf{Original review:} \textit{IMU algorithms rely heavily on the physical sensors used. Also for wearable IMU, the fixing mechanism of the wearable device will also introduce artefacts from the users' actual motion. This work has a single hardware setup: Fossil Gen 5 smartwatch with AK0991X magnetometer and LSM6DSO 6-axis accelerometer with gyroscope sampling at 50Hz. The manuscript would gain strength if other hardware setups with different IMU chips are used in at least one of the testing environments to demonstrate generalisation capabilities. Some 9DOF IMU chips even have built-in absolute orientation output, for example Bosh BNO085. It would be interesting to compare the proposed algorithm to the built-in offering of those chips.}

\textbf{Corresponding revision:}
To justify that \aliasSystem could be capable of scaling to other smart platforms that equips different sensors, we add a IMU hardware comparison in Section~\ref{hardware}, which compares the IMU raw reading between our smart watch, a Samsung Galaxy S21 5G, and an iPhone XS max.
Specifically we bind all three devices onto one solid plate and collect motion data in a hallway, so that they collect the same motion.
Figure~\ref{compare} shows the visualized results, and statistics shows that  the sensors’ relative similarities between the smartwatch and the Samsung
Galaxy S21 are 91.91$\%$, 95.18$\%$, and 97.76$\%$, for accelerometer, gyroscope, and magnetometer respectively. 
Similarities between the smartwatch and the iPhone are 97.25$\%$ 97.34$\%$, and 98.16$\%$.
This should verify \aliasSystem's scalability to other smart platforms.
The figure of experimental comparison between smart platforms is attached below:

\begin{figure} [H] 
    \subfigure[Watch Acc.]{\includegraphics[width=0.3\linewidth]{fig/compare_watch_acc.pdf}}
    \subfigure[Samsung Acc.]{\includegraphics[width=0.3\linewidth]{fig/compare_sam_acc.pdf}}
    \subfigure[iPhone Acc.]{\includegraphics[width=0.3\linewidth]{fig/compare_apple_acc.pdf}}
    
    \subfigure[Watch Gyro.]{\includegraphics[width=0.3\linewidth]{fig/compare_watch_gyro.pdf}}
    \subfigure[Samsung Gyro.]{\includegraphics[width=0.3\linewidth]{fig/compare_sam_gyro.pdf}}
    \subfigure[iPhone Gyro.]{\includegraphics[width=0.3\linewidth]{fig/compare_apple_gyro.pdf}}
    
    \subfigure[Watch Mag.]{\includegraphics[width=0.3\linewidth]{fig/compare_watch_mag.pdf}}
    \subfigure[Samsung Mag.]{\includegraphics[width=0.3\linewidth]{fig/compare_sam_mag.pdf}}
    \subfigure[iPhone Mag.]{\includegraphics[width=0.3\linewidth]{fig/compare_apple_mag.pdf}}
    
    % \vspace{-5mm}
    
    \captionsetup{labelformat=empty}
    \caption{Sensor comparison between smart devices}
    % \vspace{-5mm}
\end{figure}

\subsection{}

\textbf{Original review:} \textit{I did not find how the ground truth of the absolute orientation is established during the experiment. Is there computer vision based reflective markers? Could the ground truth introduce errors? Some visual depiction or photos of the experiment setup is recommended.}

\textbf{Corresponding revision:}
In the previous submission, in Data Collection section, we briefly introduced our ground truth data collection process.
In this revision, we assigned a separate subsection (Section~\ref{ground truth}) to introduce our data collection method.
We bind a smart watch (with IMU sensors in it) to a VR controller, and use the technique from~\cite{miao} to convert the controller's orientation and location to the smart watch, so that we can acquire the smart watch's orientation and location.
The VR device adopts computer vision based tracking technique to
locate the controller, and thus can provide accurate ground truth.
Its orientation error is below 0.85° and location error is below 0.7 cm (\cite{miao}).

\subsection{}

\textbf{Original review:} 
\textit{Re-write the dramatic languages with calm technical writing (which could also shorten the paper).
The writing requires significant revision. There are many overly-dramatic sentences.
% Examples are:
% -Magnetic field distortion is a devil hiding within the magnetic field and makes the magnetic field not trustworthy.
% - Also the artificial metal structures are not going anywhere, ...
% - whose performance is entirely at the mercy of magnetic distortion.
% - With PF joining the family, we observe a new problem among the family members.
% - However, database is also waiting for PF to give her the location to perform query. Then PF says, without orientation result from MCF he could not generate an estimation on current location. Therefore, we arrived in a deadlock.
% - thus we need not worry that MCF will run into the disaster as Gyro+Acc did in Section 3.4.
% - When the ratio reaches 100$\%$, it means forever using accelerometer, which changes MUSE into CF.
While the writing style provides a vivid narrative, I could imagine it be suitable for some books, it is not appropriate for technical academic publications. The authors need to go through the entire paper, perhaps with the help of a native English speaker, and keep a calm and objective tone.
}

\textbf{Corresponding revision:}
% We are sorry about the writing in the previous submission.
In this revision, we have thoroughly rewrote the paper and its writing, and have removed most of the non-quantitative and dramatic descriptions.
In this revision, we focus on concise introduction on the system and its workflow and design components, with plain language.

\subsection{}

\textbf{Original review:} \textit{Why is there a terminology correction section, if the authors could just replace the terms all over the manuscript?}

\textbf{Corresponding revision:}
We use uniform terms through out the paper in this revision, thus terminology correction is no longer needed.
Therefore we have removed Section 6.5 Terminology Correction in this revision, and hopefully could avoid unnecessary misunderstanding.
