# Supplementary material for: Magnetic Distortion Resistant Orientation Estimation
Source: arXiv:2410.12304 source file (2024-10-16)
Supplement: Supplementary file 2 [file Appendix_2.tex]

\appendix

\vspace{180mm}
\section*{Appendix B: Revision Report}

We thank the reviewers for the constructive comments. 
We revised the paper according to all the reviews.
% As the major differences between this revision and the previous submission, we first added more baselines for comparison experiments and more real experiments for evaluation.
% Second, we paid a lot of attention on reorganizing the paper for better understanding and reading experience.
As a major change, we added a new application study: in-air writing, using smartwatch as platform.
We also paid great attention on addressing the updating mechanism of the proposed system, to validate its robustness to magnetic environment changes, and made corresponding changes to related sections, such as Introduction, Observation, Updating design, and evaluation on the database robustness.
Other sections have also been updated in response to the reviews and suggestions.
% Third, we thoroughly revised the related work section, in order to better distinguish our work's position relevant to other existing works.
% We also added a new design component, the adaptive updating, in the design section, and many other detailed revisions.
In the following part, we present our corresponding revisions to the reviewers' comments. 
Again we thank all reviewers for their insightful reviews.

\section{Reviewer 1 (1AE)}

We first would like to thank you for the review and summarizing the comments.
The following revisions list the original review comments, followed by our corresponding updates to the paper and responses to the concerns.
Some revisions may be split into multiple sub-revisions and are answered individually.

\subsection{}
\textbf{Review:}
\textit{1. Provide more details about the novelty of the work (R2, R4). In particular, R2 points out that reference [26] also tackles the same problem with a different methodology. }

\textbf{Revision:} 
\subsubsection{R2's concern: reference [26] tackles the same problem}

To better address this concern, we updated the related description in Introduction: \textit{'They use the intensity and angle of the magnetic field to indicate if distortion is strong, based on which they adjust the weight of magnetometer usage.'}, and also in Related Work Section: 
\textit{'However, if distortion is high, they will have very low weight for magnetometer, and thus suffer from either the absence of magnetic calibration or magnetic distortion (to be verified in Section \ref{eval_distortion}).
Instead, in this paper, we propose a novel system that models and corrects magnetic distortion in orientation estimation, even when distortion is high.'}.

In the Related Work Section \ref{related} we introduced reference \cite{fan2017adaptive} and compared their strategy with our strategy in handling distortion.

Reference \cite{fan2017adaptive} mainly decreases the weight for magnetometer as distortion rises (or we could also say increasing weight when distortion is absent), thus avoiding the negative impact of magnetic distortion.
% This feature is most reveal when the distortion is high.
However, if distortion is high, reference \cite{fan2017adaptive} will have very low weight for magnetometer, and thus suffers from either the absence of magnetic calibration or magnetic distortion (verified in Section \ref{eval_distortion}).
On the other hand, our proposed approach, \aliasSystem, models the magnetic distortion using a magnetic anchor database, which is a major difference compared to reference \cite{fan2017adaptive}.
This extra information can help orientation estimation algorithm better resist distortion, as the database corrects the wrong anchor, so that the algorithm does not need to avoid using magnetometer for calibration, and does not face the issue of absent magnetic calibration.

\begin{figure}[H]
    \vspace{-1mm}
    \hfill
    \begin{minipage}[t]{0.43\linewidth}
        \centering
        \small
        % \vspace{-0.1cm}
        \includegraphics[width=1\linewidth]{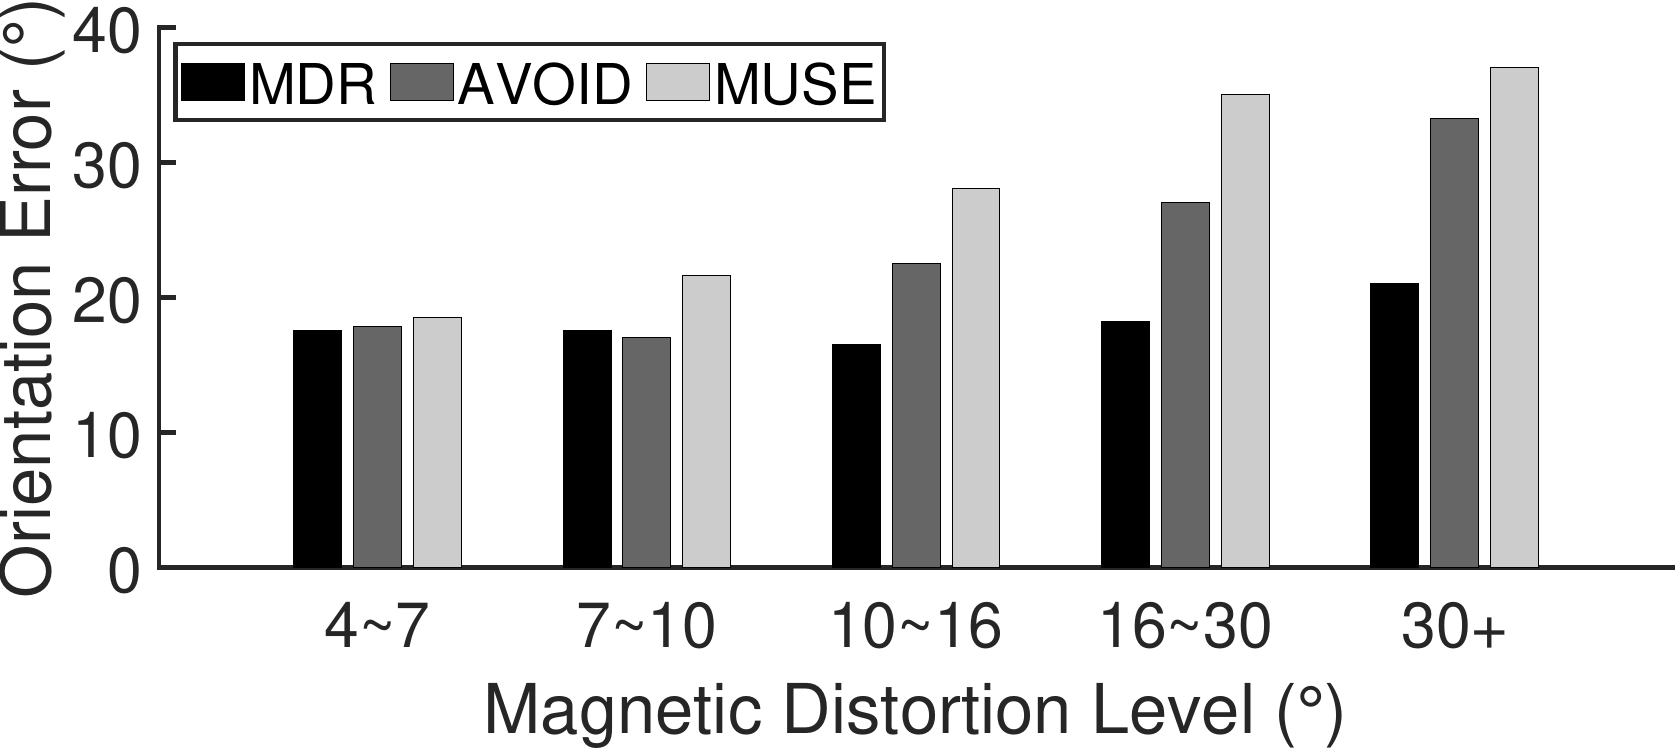}
        \vspace{-8mm}
        \captionsetup{labelformat=empty}
        \caption{Performance at different distortion levels.}
        % \label{result}
    \end{minipage}
    \hfill
    \begin{minipage}[t]{0.45\linewidth}
            % \hspace{-0.1cm}
        \centering
        % \vspace{-2cm}
        \includegraphics[width=\linewidth]{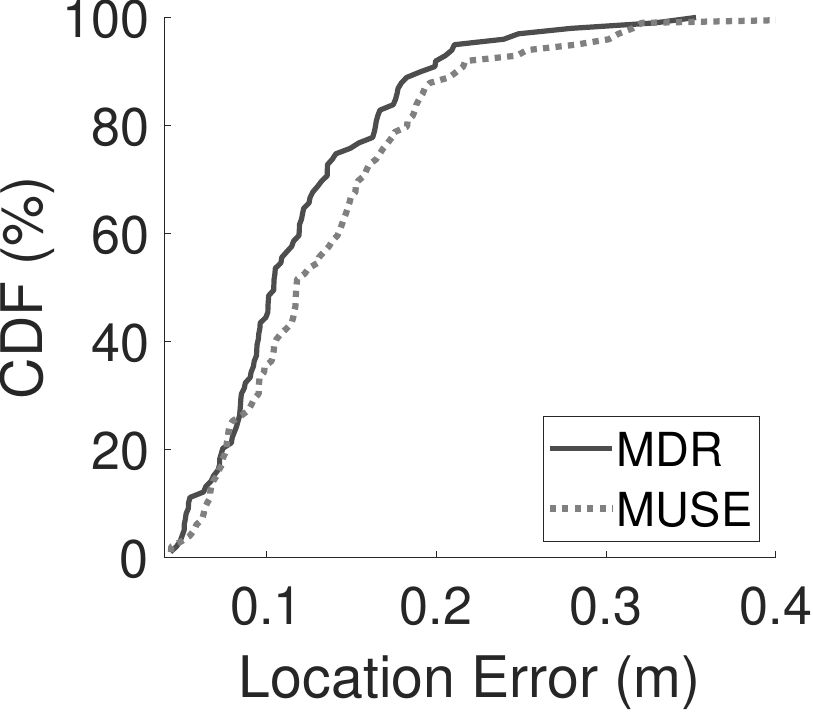}
        \vspace{-3mm}
        \captionsetup{labelformat=empty}
        \caption{Overall location estimation error.}
        \vspace{-3mm}
    \end{minipage}
    \hfill
    \vspace{-4mm}
\end{figure}

To verify our speculations we also implemented reference \cite{fan2017adaptive} into a baseline algorithm \textit{AVOID} (introduced in Section \ref{baselines}).
As a result of the experiments, the overall average orientation errors are 16.42°, 29.57°,and 21.67° for \aliasSystem, MUSE, and $AVOID$, respectively.
\aliasSystem has an overall improvement of 44.47$\%$ over MUSE and 24.23$\%$ over $AVOID$.
To explain this improvement, we also zoomed into the magnetic distortion resistance capability in Section \ref{eval_distortion}.
Figure \ref{result} demonstrated that reference \cite{fan2017adaptive} is not effective at resisting high distortion, while \aliasSystem maintains a relatively stable performance as distortion level increases.

More detailed information can be found in the response to sub-review \ref{26}.

\subsubsection{R4's concern of the novelty of the work}

To better address this concern, we first updated the relevant introduction in the Related Work Section \ref{related}:
\textit{'Therefore, we focus heavily on orientation error and how it flows within the system.
We design novel techniques to reduce orientation error and its impact, such as adaptive updating (to be introduced in Section \ref{adaptive_updating}) and orientation error-reduction (to be introduced in Section~\ref{boost_ori_1} and \ref{boost_ori_2}).'}

The database design in this work is a new approach that cannot be easily substituted by existing solutions in the context of resisting magnetic distortion in orientation estimation (Section \ref{related}).

% To better address this concern, we first updated the relevant description in the Related Work section:

% \textit{'However, if distortion is high, they \cite{fan2017adaptive, ahrs, madgwick} will have very low weight for magnetometer, and thus suffer from either the absence of magnetic calibration or magnetic distortion (to be verified in Section \ref{eval_distortion}).
% Instead, in this paper, we propose a novel system that models and corrects magnetic distortion in orientation estimation, even when distortion is high.'}

% This paragraph is to identify our system's difference compared to existing distortion-handling methods \cite{fan2017adaptive, ahrs, madgwick}.
% They use magnetic field's magnitude and dip angle as indicator of distortion, and tune the weight for magnetometer accordingly.
% Therefore, they either lose the effect of magnetic calibration or suffer from distortion, and this issue is especially serious when distortion is high, as verified in Section \ref{result}.

Specifically, the most related magnetic field modelling technique is the fingerprinting method for localization.
However, our database, i.e., the magnetic anchor database, stores the magnetic field direction, and is used to correct orientation estimation, while fingerprinting is used to locate devices.
The major differences between them are:

First, the magnetic anchor database requires a higher spatial resolution than fingerprinting that usually conducts meter-level positioning (e.g., MVP \cite{wang2021mvp} locates cars with accuracy of 3.89 m), since short distance (e.g., 0.1m) can make the magnetic field direction largely vary (studied in Section \ref{spatial corr} and Figure \ref{spatial}).
High resolution requirement largely increases the database preparation overhead.
To that end, we propose a novel automatic database updating mechanism in Section \ref{db_updating} to cancel the database preparation overhead.

Second, the error sourcing in the magnetic anchor database is a novel issue to be solved, due to its unique purpose of modelling and correcting magnetic distortion in orientation estimation (discussed in detail in the beginning of Section \ref{pro}).
Specifically, building and updating a database requires two factors: location and anchor, where the location information is inferred by the particle filter and shares its error, and the magnetic anchor is calculated using estimated orientation and magnetometer readings, which is affected by orientation error.
Additionally, the database will be queried to provide distortion-correction information to assist orientation estimation, which will also contain error if the query location is wrong.
The errors in query and updating process will also have correlation as the system workflow iterates (Section \ref{workflow}).
Based on these observations and motivations, we proposed novel techniques in Section \ref{pro} to reduce errors in database operations, whose improvements are also verified with experiments and presented in Section \ref{decompose}.

% Our key novelties in solving these issues are the auto-updating mechanism (Section \ref{selfDB}) that cancels the and the error-reduction designs, both

Detailed response can be found in sub-revision \ref{revision_new_or_not}.

Thank you for the review.

\subsection{}
\textbf{Review:}
\textit{There is a need to rewrite the second paragraph of the introduction section and make it more precise (R2).}

\textbf{Revision:} 

We re-wrote the second paragraph of Introduction to address the concern on reference \cite{fan2017adaptive}:
\textit{Current distortion handling methods \cite{fan2017adaptive, ahrs, madgwick} either reduce or avoid the usage of magnetometer upon detecting magnetic distortion.
They use the intensity and angle of the magnetic field to indicate if distortion is strong, based on which they adjust the weight of magnetometer usage.
However, they partially avoid the impact of magnetic distortion, but then suffer from the absence of magnetometer calibration, thus fail when distortion is high.}

Thank you for the suggestion.

\subsection{}
\textbf{Review:}
\textit{R4 is also concerned if the proposed method is realistic / feasible in actual applications.}

\textbf{Revision:} 

Based on our best understanding, R4 seems to be concerned on whether location accuracy can reach 0.1m level and support magnetic-field-modelling-database operations.

To better address this concern, we first updated the relevant introduction in the Background Section \ref{secBackground}:
\textit{'While many studies have been done in location estimation of arm tracking \cite{cutti2008ambulatory,el2012shoulder,riaz2015motion, tautges2011motion, shen2016smartwatch, liu2019real, muse}, \aliasSystem follows the state-of-the-art arm tracking solution MUSE, and adopts the particle filter to estimate the smartwatch's location.'}

The key to answering this is that we followed the particle filter design from the previous work MUSE \cite{muse} for location estimation, and made an improvement to it in Section \ref{secCorrectedPF}.
It could reach such error level, with its methodology introduced in Background Section \ref{particle}: Location Estimation via Particle Filter.
It mainly make use of the restrain of human skeleton to acquire possible locations with a specific posture (specifically, wrist posture, since the smartwatch is there).
It uses a particle filter to deploy particles onto the possible locations, and uses the measured acceleration to distinguish whether the particles are tracking the wrist accurately.
The particle filter then refines the particles based on their tracking accuracy in every iteration, and selects the particle with the highest accuracy as the inferred location of the wrist, and thus enables relatively accurate wrist tracking.

Based on experiments, \aliasSystem has a location estimation error of 0.1083m (Evaluation on location estimation error, Section \ref{eval_loc}).
This 0.1-meter-level location accuracy is enough for magnetic distortion modelling, verified in Section \ref{spatial corr} and Figure \ref{spatial}.

% We also conducted experiment with different spatial resolution of the database in Section \ref{secDatabaseResolution}, which indicates that 0.1m$^3$ is the optimal database spatial resolution in current system setting.

% This 0.1-meter-level error is enabled by the particle filter-based stochastic location estimation frame work propose by a previous work MUSE (0.1364m location error in our experiment).
% We followed MUSE's overall location estimation framework in our system design, and introduced it in Background Section \ref{particle}: Location Estimation via Particle Filter.

% As for the error level of the \textit{'positional information'}, based on experiments, \aliasSystem has a location estimation error of 0.1083m (Evaluation on location estimation error, Section \ref{eval_loc}).
% This 0.1-meter-level location accuracy is enough for magnetic distortion modelling.
% As introduced in Section \ref{spatial corr} and Figure \ref{spatial}, 0.1-meter distance only results in limited angular difference in the magnetic field directions.
% Therefore, even with 0.1-meter-level location error, the database is still able to model the magnetic distortion with enough accuracy.

\begin{figure}[H]
    \vspace{-1mm}
    \hfill
    \begin{minipage}[t]{0.25\linewidth}
        \centering
        \includegraphics[width=\linewidth]{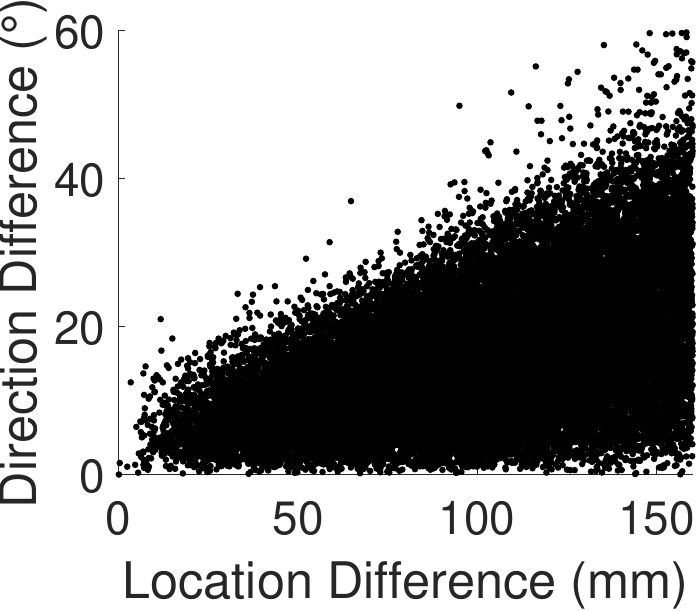}
         \vspace{-7mm}
        \captionsetup{labelformat=empty}
        \caption{Spatial correlation of the magnetic field.}
        % \vspace{0cm}
        % \label{spatial}
    \end{minipage}
    \hfill
    \begin{minipage}[t]{0.45\linewidth}
            % \hspace{-0.1cm}
        \centering
        % \vspace{-2cm}
        \includegraphics[width=\linewidth]{fig/sensys_localization.pdf}
        \vspace{-3mm}
        \captionsetup{labelformat=empty}
        \caption{Overall location estimation error.}
        \vspace{-3mm}
    \end{minipage}
    \hfill
    \vspace{-4mm}
\end{figure}

Additionally, the database updating mechanism makes use of the feature that one location can be visited multiple times, resulting in an aggregated datapoint based on all historical measurements, which will reduce overall noise and improve the database's accuracy overtime, as verified in Section \ref{DBeval} and Figure \ref{build up} and Figure \ref{build up 2}:

\begin{figure}[H]
    % \vspace{-0.2cm}
    \hfill
    \begin{minipage}[t]{0.26\linewidth}
        \centering
        % \vspace{-0.1cm}
        \includegraphics[width=1\linewidth]{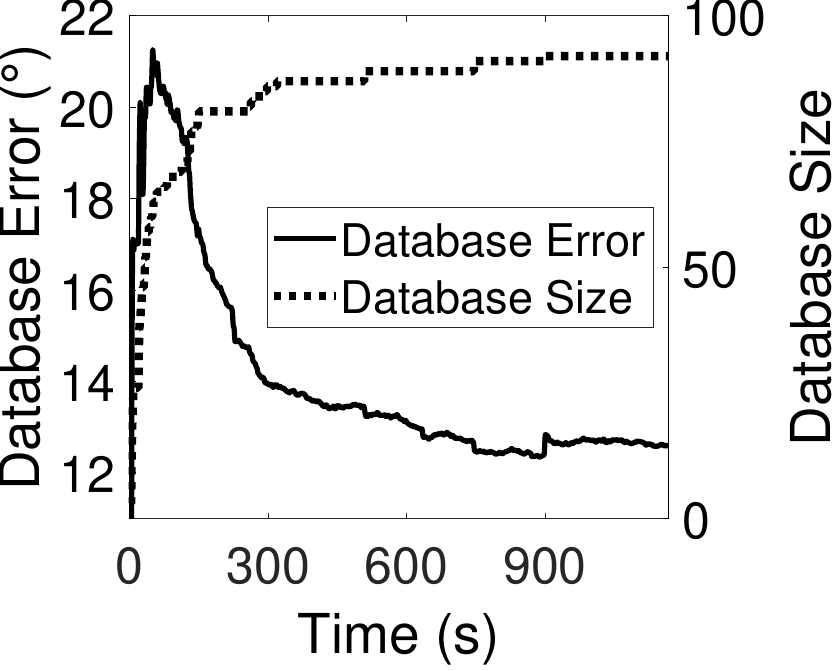}
        \vspace{-7mm}
        \captionsetup{labelformat=empty}
        \caption{Database accuracy and database size during self-construction.}
        % \vspace{-0.5cm}
        % \label{build up}
    \end{minipage}
    \hfill
    \begin{minipage}[t]{0.26\linewidth}
        \centering
        % \vspace{-0.1cm}
        \includegraphics[width=1\linewidth]{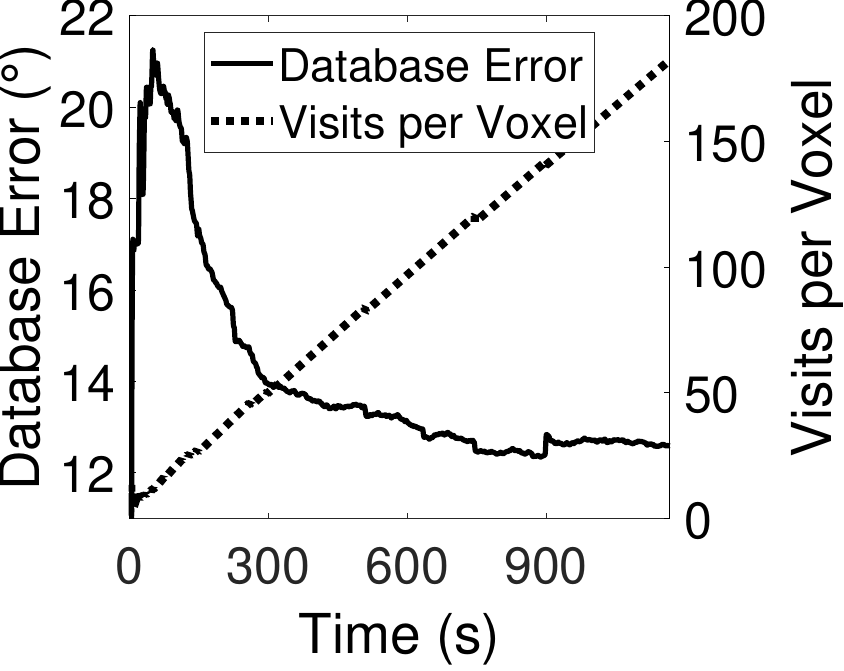}
        \vspace{-7mm}
        \captionsetup{labelformat=empty}
        \caption{Database accuracy and visits per voxel during self-construction.}
        % \vspace{-0.5cm}
        % \label{build up 2}
    \end{minipage}
    \hfill
    \begin{minipage}[t]{0.19\linewidth}
        \centering
        % \vspace{-0.1cm}
        \includegraphics[width=1\linewidth]{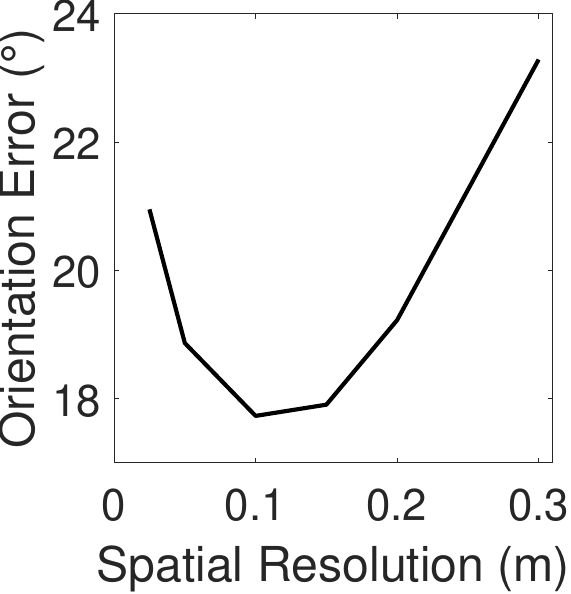}
        \vspace{-7mm}
        \captionsetup{labelformat=empty}
        \caption{\aliasSystem error with different spatial resolution.}
        % \vspace{-0.5cm}
        % \label{prec}
    \end{minipage}
    \hfill
    \vspace{-2mm}
\end{figure}

We also conducted experiment with different spatial resolution of the database in Section \ref{secDatabaseResolution}, with results shown in Figure \ref{prec}, which indicates that 0.1m is the optimal database spatial resolution in current system setting.

More details can also be found in the revision response to sub-revision \ref{10cm}.
% and sub-revision \ref{stochastic}.

Thank you for the review.

\subsection{}
\textbf{Review:}

\textit{2. There still is a need to clarify how the proposed method could be applied in practical applications (R3, R4).} 

\textbf{Revision:} 

\subsubsection{R3's concern on practical application}

Based on our best understanding, \textbf{R3's first concern} on practical applications seems to be 'how the proposed method would enable new applications? Or make existing applications significantly different (e.g., from unable to usable?).'.

As an answer to that, \aliasSystem  enables new applications via making it possible for applications to be deployed in magnetically distorted indoor scenarios, which were not possible due to missing or incapable magnetic distortion handling mechanism.
% Other than the case study on Star Sky Rendering (Section \ref{eval_star}), in this revision we also added another case study in Section \ref{writing}, which demonstrates an in-air writing application.
% This new application is mainly based on location information, which also requires orientation estimation results (via particle filter).
Taking the new in-air writing case study (Section \ref{writing}) as example, from the in-air writing traces inferred by MUSE, we can see it is not very capable of supporting this indoor smart application, since the letters it infers are barely recognizable (Figure \ref{demo_muse}, also listed below).
On the other hand, \aliasSystem is capable of resisting the indoor magnetic distortion and track the writing with relatively clear shape (Figure \ref{demo_mdr}).
Therefore, we could say that \aliasSystem enables smart applications in magnetically distorted scenarios, where existing solutions could not well support them.
% Magnetic distortion makes the magnetometer’s reading deviate from true north and point to different directions at different locations, resulting in large errors in orientation estimation.

Detailed response can be found in \ref{revision_r3_enable}.

\begin{figure} [h]
    \vspace{-3mm}
    \subfigure['A']{\includegraphics[width=0.04\linewidth]{fig/gt/1_20°_220°.png}}
    \hfill
    \subfigure['B']{\includegraphics[width=0.04\linewidth]{fig/gt/2_20°_220°.png}}
    \hfill
    \subfigure['C']{\includegraphics[width=0.04\linewidth]{fig/gt/3_20°_220°.png}}
    \hfill
    \subfigure['D']{\includegraphics[width=0.04\linewidth]{fig/gt/4_20°_220°.png}}
    \hfill
    \subfigure['E']{\includegraphics[width=0.04\linewidth]{fig/gt/5_20°_220°.png}}
    \hfill
    \subfigure['F']{\includegraphics[width=0.04\linewidth]{fig/gt/6_20°_220°.png}}
    \hfill
    \subfigure['G']{\includegraphics[width=0.04\linewidth]{fig/gt/7_20°_220°.png}}
    \hfill
    \subfigure['H']{\includegraphics[width=0.04\linewidth]{fig/gt/8_20°_220°.png}}
    \hfill
    \subfigure['I']{\includegraphics[width=0.035\linewidth]{fig/gt/9_20°_220°.png}}
    \hfill
    \subfigure['J']{\includegraphics[width=0.04\linewidth]{fig/gt/10_20°_220°.png}}
    \hfill
    \subfigure['K']{\includegraphics[width=0.04\linewidth]{fig/gt/11_20°_220°.png}}
    \hfill
    \subfigure['L']{\includegraphics[width=0.04\linewidth]{fig/gt/12_20°_220°.png}}
    \hfill
    \subfigure['M']{\includegraphics[width=0.04\linewidth]{fig/gt/13_20°_220°.png}}
    \hfill
    \subfigure['N']{\includegraphics[width=0.04\linewidth]{fig/gt/14_20°_220°.png}}
    \hfill
    \subfigure['1']{\includegraphics[width=0.04\linewidth]{fig/gt/15_20°_220°.png}}
    \hfill
    \subfigure['2']{\includegraphics[width=0.04\linewidth]{fig/gt/16_20°_220°.png}}
    \hfill
    \subfigure['3']{\includegraphics[width=0.04\linewidth]{fig/gt/17_20°_220°.png}}
    \hfill
    \subfigure['4']{\includegraphics[width=0.04\linewidth]{fig/gt/18_20°_220°.png}}
    \hfill
    \subfigure[Tri.]{\includegraphics[width=0.04\linewidth]{fig/gt/19_20°_220°.png}}
    \hfill
    \subfigure[Rect.]{\includegraphics[width=0.04\linewidth]{fig/gt/20_20°_220°.png}}
    \vspace{-3mm}
        \captionsetup{labelformat=empty}
    \caption{In-Air Writing Trace Ground Truth Collected by VR System}
    % \label{demo_gt}
    
    % \vspace{-1mm}
    % \vspace{-1mm}
    \subfigure['A']{\includegraphics[width=0.04\linewidth]{fig/mdr/1_20°_220°.png}}
    \hfill
    \subfigure['B']{\includegraphics[width=0.04\linewidth]{fig/mdr/2_20°_220°.png}}
    \hfill
    \subfigure['C']{\includegraphics[width=0.04\linewidth]{fig/mdr/3_20°_220°.png}}
    \hfill
    \subfigure['D']{\includegraphics[width=0.04\linewidth]{fig/mdr/4_20°_220°.png}}
    \hfill
    \subfigure['E']{\includegraphics[width=0.04\linewidth]{fig/mdr/5_20°_220°.png}}
    \hfill
    \subfigure['F']{\includegraphics[width=0.04\linewidth]{fig/mdr/6_20°_220°.png}}
    \hfill
    \subfigure['G']{\includegraphics[width=0.04\linewidth]{fig/mdr/7_20°_220°.png}}
    \hfill
    \subfigure['H']{\includegraphics[width=0.04\linewidth]{fig/mdr/8_20°_220°.png}}
    \hfill
    \subfigure['I']{\includegraphics[width=0.035\linewidth]{fig/mdr/9_20°_220°.png}}
    \hfill
    \subfigure['J']{\includegraphics[width=0.04\linewidth]{fig/mdr/10_20°_220°.png}}
    \hfill
    \subfigure['K']{\includegraphics[width=0.04\linewidth]{fig/mdr/11_20°_220°.png}}
    \hfill
    \subfigure['L']{\includegraphics[width=0.04\linewidth]{fig/mdr/12_20°_220°.png}}
    \hfill
    \subfigure['M']{\includegraphics[width=0.04\linewidth]{fig/mdr/13_20°_220°.png}}
    \hfill
    \subfigure['N']{\includegraphics[width=0.04\linewidth]{fig/mdr/14_20°_220°.png}}
    \hfill
    \subfigure['1']{\includegraphics[width=0.04\linewidth]{fig/mdr/15_20°_220°.png}}
    \hfill
    \subfigure['2']{\includegraphics[width=0.04\linewidth]{fig/mdr/16_20°_220°.png}}
    \hfill
    \subfigure['3']{\includegraphics[width=0.04\linewidth]{fig/mdr/17_20°_220°.png}}
    \hfill
    \subfigure['4']{\includegraphics[width=0.04\linewidth]{fig/mdr/18_20°_220°.png}}
    \hfill
    \subfigure[Tri.]{\includegraphics[width=0.04\linewidth]{fig/mdr/19_20°_220°.png}}
    \hfill
    \subfigure[Rect.]{\includegraphics[width=0.04\linewidth]{fig/mdr/20_20°_220°.png}}
    \vspace{-3mm}
        \captionsetup{labelformat=empty}
    \caption{In-Air Writing Trace Inferred by \aliasSystem}
    % \label{demo_mdr}
    
    % \vspace{-1mm}
    \vspace{1mm}
    \subfigure['A']{\includegraphics[width=0.04\linewidth]{fig/muse/1_20°_220°.png}}
    \hfill
    \subfigure['B']{\includegraphics[width=0.04\linewidth]{fig/muse/2_20°_220°.png}}
    \hfill
    \subfigure['C']{\includegraphics[width=0.04\linewidth]{fig/muse/3_20°_220°.png}}
    \hfill
    \subfigure['D']{\includegraphics[width=0.04\linewidth]{fig/muse/4_20°_220°.png}}
    \hfill
    \subfigure['E']{\includegraphics[width=0.04\linewidth]{fig/muse/5_20°_220°.png}}
    \hfill
    \subfigure['F']{\includegraphics[width=0.04\linewidth]{fig/muse/6_20°_220°.png}}
    \hfill
    \subfigure['G']{\includegraphics[width=0.04\linewidth]{fig/muse/7_20°_220°.png}}
    \hfill
    \subfigure['H']{\includegraphics[width=0.04\linewidth]{fig/muse/8_20°_220°.png}}
    \hfill
    \subfigure['I']{\includegraphics[width=0.035\linewidth]{fig/muse/9_20°_220°.png}}
    \hfill
    \subfigure['J']{\includegraphics[width=0.04\linewidth]{fig/muse/10_20°_220°.png}}
    \hfill
    \subfigure['K']{\includegraphics[width=0.04\linewidth]{fig/muse/11_20°_220°.png}}
    \hfill
    \subfigure['L']{\includegraphics[width=0.04\linewidth]{fig/muse/12_20°_220°.png}}
    \hfill
    \subfigure['M']{\includegraphics[width=0.04\linewidth]{fig/muse/13_20°_220°.png}}
    \hfill
    \subfigure['N']{\includegraphics[width=0.04\linewidth]{fig/muse/14_20°_220°.png}}
    \hfill
    \subfigure['1']{\includegraphics[width=0.04\linewidth]{fig/muse/15_20°_220°.png}}
    \hfill
    \subfigure['2']{\includegraphics[width=0.04\linewidth]{fig/muse/16_20°_220°.png}}
    \hfill
    \subfigure['3']{\includegraphics[width=0.04\linewidth]{fig/muse/17_20°_220°.png}}
    \hfill
    \subfigure['4']{\includegraphics[width=0.04\linewidth]{fig/muse/18_20°_220°.png}}
    \hfill
    \subfigure[Tri.]{\includegraphics[width=0.04\linewidth]{fig/muse/19_20°_220°.png}}
    \hfill
    \subfigure[Rect.]{\includegraphics[width=0.04\linewidth]{fig/muse/20_20°_220°.png}}
    \vspace{-3mm}
     \captionsetup{labelformat=empty}
    \caption{In-Air Writing Trace Inferred by MUSE}
    % \label{demo_muse}
\end{figure}

R3's \textbf{second concern} is on whether the proposed method is robust when the context has been changed.

To better address this issue, we have updated Section \ref{DBeval} with more explanation:
\textit{'In conclusion, a database can adapt to new places with exploration of a few minutes, with adequate size and accuracy.
For new scenarios, \aliasSystem requires no pre-scanning or past database history, but instead builds a new database from scratch in a few minutes.'}

Also in Section \ref{secExperimentSetting}, where we specify the experiment setting, we added:
\textit{
'Specifically, for all real experiments in this work, \aliasSystem has no access to any pre-scan or any information on past-built databases in the same places. 
Instead, \aliasSystem regards all scenarios as new, and has to build its own database from scratch to model the local magnetic field.'
}

For the issue itself, in Section \ref{stability}, we conducted experiments to show that magnetic distortion pattern is stable.
On the other hand, in Section \ref{DBeval}, evaluation shows that the database takes 5 minutes to built itself to a decent size and accuracy.
Taking the two factors above and put in another way, given that the time for database build-up is short, we can assume there will be no change in the pattern of magnetic distortion during the build up of \aliasSystem.

\begin{figure}[h]
    \vspace{-1mm}
    \hfill
    \begin{minipage}[t]{0.25\linewidth}
        \centering
        \includegraphics[width=\linewidth]{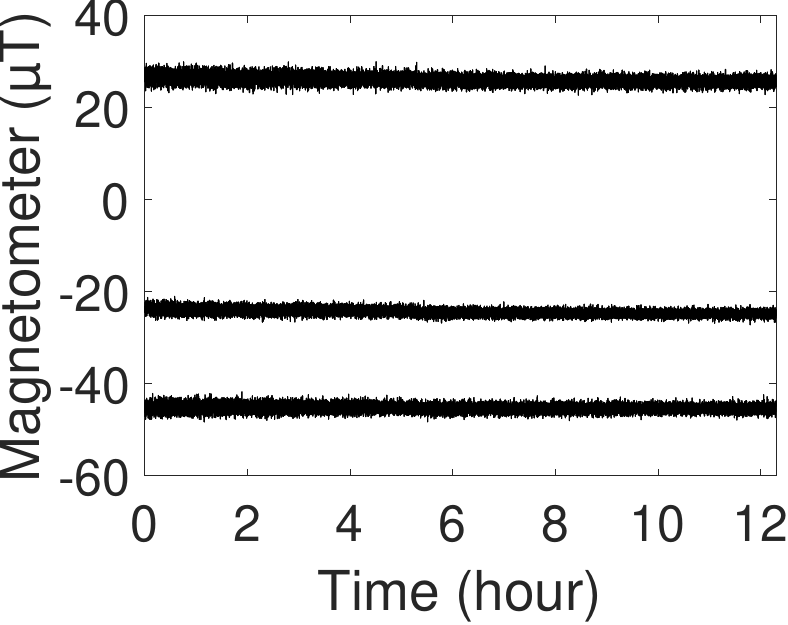}
         \vspace{-7mm}
     \captionsetup{labelformat=empty}
        \caption{Temporal stability of the magnetic field.}
        % \vspace{0cm}
        % \label{temporal}
    \end{minipage}
    \hfill
    \vspace{-4mm}
\end{figure}

As for the issue of location changes of appliances, \aliasSystem can solve this issue as it auto-adapts to new scenarios. It constructs and updates its own database via utilizing estimated orientation and location.
MDR uses estimated orientation and location, along with the magnetometer reading 
to automatically build and update the database.
For any new scenario, MDR relies on automatic updating to explore and adapt to it, without any pre-modelling (Section \ref{workflow}). 
Section \ref{DBeval} also verifies the efficiency and accuracy of the database auto-construction with experimental results.

\begin{figure}[H]
    % \vspace{-0.2cm}
    \hfill
    \begin{minipage}[t]{0.26\linewidth}
        \centering
        % \vspace{-0.1cm}
        \includegraphics[width=1\linewidth]{fig/sensys_db_during_build_up_1.pdf}
        \vspace{-7mm}
        \captionsetup{labelformat=empty}
        \caption{Database accuracy and database size during self-construction.}
        % \vspace{-0.5cm}
        % \label{build up}
    \end{minipage}
    \hfill
    \begin{minipage}[t]{0.26\linewidth}
        \centering
        % \vspace{-0.1cm}
        \includegraphics[width=1\linewidth]{fig/sensys_db_during_build_up_2.pdf}
        \vspace{-7mm}
        \captionsetup{labelformat=empty}
        \caption{Database accuracy and visits per voxel during self-construction.}
        % \vspace{-0.5cm}
        % \label{build up 2}
    \end{minipage}
    \hfill
    \vspace{-2mm}
\end{figure}
% With this mechanism

In conclusion, \aliasSystem does not require any beforehand-information, such as pre-scanning or historical database, and regards all deployments as new scenarios.
It starts from scratch to explore the new location, and is able to build a usable database for the new scenario in minutes.
After each deployment, \aliasSystem does not save the database, but discard it and builds a new one in the next new deployment.
Therefore \aliasSystem is robust when the magnetic distortion context has changed, as all experiments we conducted for \aliasSystem are regarded as new scenarios, where \aliasSystem has no access to pre-scanning or past-built databases.

Detailed response can be found in sub-revision \ref{revision_robust}.

\subsubsection{R4's concern on practical application}

Based on our best understanding, we assume R4 is \textbf{first concerned} on the practicality of the particle filter having enough accuracy to support the database (sub-review \ref{10cm}), which we have answered in the previous question, and also in the response to sub-review \ref{10cm}.
In a word, the particle filter uses human skeleton information and wrist orientation to track the location of the wrist and the smartwatch on it, and is capable of supporting the system with 10cm-level-accuracy (0.1086m in Section \ref{eval_loc}).
Therefore the system is practical on this perspective.

\textbf{Another concern of R4} is on the application case study, and whether the real-case application can be realized on the smartwatch platform.

Our case studies (including the previous Star Sky Rendering), are targeting the IMU sensors, as many smartphones and smartwatches share the same IMU settings.
% For example, the smartwatch we used is equipped with AK0991X magnetometer and LSM6DSO 6-axis accelerometer with gyroscope.
% Its sampling rate is 50 Hz for all three sensors.
% There are also other mobile devices that use the same sensors, such as Sony Xperia 1 III, Oneplus 7, Motorola moto g fast, MiWatch, Xiaomi Mi 10T Pro, and TicWatch Pro 3. 
% To prove the \aliasSystem's scalability to other platforms, we conducted real experiments to compare the IMU sensors between the smartwatch and a a Samsung Galaxy S21 5G and an iPhone XS max, which shows high similarities and implies that \aliasSystem should be able to conveniently deploy on other platforms with similar performance.

As response in practice to that concern, we conducted a new case study using smartwatch as platform in Section \ref{writing}.
This new application is mainly based on location information, which also requires orientation estimation results (via particle filter).
Specifically, we use the smartwatch to write symbols in-air.
% Finally, we demonstrate the in-air writing application of \aliasSystem using smartwatch.
A potential real use case is that a user wears a smartwatch and write symbols in air to interact with smart devices.
We write 20 symbols in the corridor, where magnetic distortion affects orientation estimation, and thus affects location estimation, causing inaccurate writing traces inference.
The symbols include letters and numbers, and a triangle and a rectangle, as shown in Figure \ref{demo_gt}, which are the ground truth writing trace collected by the VR device.
% captured at a proper camera angle (20° down to the user's facing direction).
We run \aliasSystem and MUSE on the same trace using only IMU sensors' data, and show their inferred traces in Figure \ref{demo_mdr} and Figure \ref{demo_muse}.
\aliasSystem is demonstrating a better performance in tracking the writing trace of the smartwatch.

Detailed response can be found in sub-revision \ref{revision_case_2}

Thank you for the review.

\begin{figure} [h]
    \vspace{-3mm}
    \subfigure['A']{\includegraphics[width=0.04\linewidth]{fig/gt/1_20°_220°.png}}
    \hfill
    \subfigure['B']{\includegraphics[width=0.04\linewidth]{fig/gt/2_20°_220°.png}}
    \hfill
    \subfigure['C']{\includegraphics[width=0.04\linewidth]{fig/gt/3_20°_220°.png}}
    \hfill
    \subfigure['D']{\includegraphics[width=0.04\linewidth]{fig/gt/4_20°_220°.png}}
    \hfill
    \subfigure['E']{\includegraphics[width=0.04\linewidth]{fig/gt/5_20°_220°.png}}
    \hfill
    \subfigure['F']{\includegraphics[width=0.04\linewidth]{fig/gt/6_20°_220°.png}}
    \hfill
    \subfigure['G']{\includegraphics[width=0.04\linewidth]{fig/gt/7_20°_220°.png}}
    \hfill
    \subfigure['H']{\includegraphics[width=0.04\linewidth]{fig/gt/8_20°_220°.png}}
    \hfill
    \subfigure['I']{\includegraphics[width=0.035\linewidth]{fig/gt/9_20°_220°.png}}
    \hfill
    \subfigure['J']{\includegraphics[width=0.04\linewidth]{fig/gt/10_20°_220°.png}}
    \hfill
    \subfigure['K']{\includegraphics[width=0.04\linewidth]{fig/gt/11_20°_220°.png}}
    \hfill
    \subfigure['L']{\includegraphics[width=0.04\linewidth]{fig/gt/12_20°_220°.png}}
    \hfill
    \subfigure['M']{\includegraphics[width=0.04\linewidth]{fig/gt/13_20°_220°.png}}
    \hfill
    \subfigure['N']{\includegraphics[width=0.04\linewidth]{fig/gt/14_20°_220°.png}}
    \hfill
    \subfigure['1']{\includegraphics[width=0.04\linewidth]{fig/gt/15_20°_220°.png}}
    \hfill
    \subfigure['2']{\includegraphics[width=0.04\linewidth]{fig/gt/16_20°_220°.png}}
    \hfill
    \subfigure['3']{\includegraphics[width=0.04\linewidth]{fig/gt/17_20°_220°.png}}
    \hfill
    \subfigure['4']{\includegraphics[width=0.04\linewidth]{fig/gt/18_20°_220°.png}}
    \hfill
    \subfigure[Tri.]{\includegraphics[width=0.04\linewidth]{fig/gt/19_20°_220°.png}}
    \hfill
    \subfigure[Rect.]{\includegraphics[width=0.04\linewidth]{fig/gt/20_20°_220°.png}}
    \vspace{-3mm}
        \captionsetup{labelformat=empty}
    \caption{In-Air Writing Traces}
\end{figure}

% As for R3, we assume the concern of practicality is on 'whether changes of building structure (magnetic environment) have any impact on the updating section' (sub-review \ref{revision_reconstruction}).
% The short answer is: \aliasSystem is immune to such issue, unless the building structure is constantly, frequently, and drastically changing, which is rare in real life.

\subsection{}
\textbf{Review:}

\textit{The paper describes the star sky rendering scenario, however, it does not seem to clarify how the technical improvements can benefit the application itself. Also, explain the application-relevant values of this paper's technical contribution in view of the availability of many devices/applications such as AR/VR headsets (R3).}

\textbf{Revision:} 

\subsubsection{How the technical improvements can benefit the application itself}

To the best of our understanding, R3's concern is how the improvement of rendering accuracy of can benefit the application itself (mainly for the star sky rendering application).

To answer that question, we updated the star sky rendering case study Section \ref{eval_star} with more explanation on the matter:
\textit{'Inaccurate star sky rendering leads to impaired App user experience, and may also cause misleading guidance for astronomy fans.
For example, astronomy fans usually use star sky Apps to find the approximate area of a constellation (which may not be directly found by human eyes) before precisely aligning the telescope, and thus inaccurate star sky information would decrease the efficiency of this coarse searching.'}

% We deploy \aliasSystem and evaluate its star sky rendering accuracy, with MUSE as comparison.
% We evaluate the algorithms in this application with the metric of 'how much percent of the stars in the ground truth view port are covered by the estimated view port'.
% The overall accuracy for the star sky rendering is 86.69$\%$ for \aliasSystem, and 70.92$\%$ for MUSE.

Star sky App users would expect the rendering result to be as accurate as possible, so that they may efficiently search for the stars they want to observe.
Additionally, many constellations in the actual star sky are not directly visible to human eyes.
Although a telescope can clearly visualize them, the outlook of a telescope is limited, therefore it would inefficient to use telescope to search for constellations.
To that end, users may rely on star sky Apps to coarsely find the constellations before they use the telescope for fine searching.
If the user is using a telescope indoor and observe the stars through the window, indoor magnetic distortion may affect the orientation estimation of his/her smartphone, causing the star sky App to provide inaccurate constellation information.
In this case, \aliasSystem would be able to help resist distortion and maintain efficiency for the user to search for the constellation to be observed, and thus potentially improve user experience.

Detailed response can be found in sub-revision \ref{revision_r3_app}.

\subsubsection{Comparing to AR/VR headsets and other CV-based methods}

First, to better address this concern, we updated the related paragraph in the Background Section \ref{secBackground}:
\textit{'Compared to other computer vision or wireless sensing-based works, IMU-based orientation estimation has an advantage of independence, as it only requires the IMU sensors on the mobile platform.
Additionally, as IMU sensors are vastly available on smart platforms, IMU-based methods can also be conveniently and ubiquitously deployed.'}

IMU-based methods have a great advantage of independence, compared to other infrastructure-based methods (e.g., computer vision, wireless sensing).
CV-based methods requires designated hardware, e.g., depth cameras, infrared sensors and emitters, which can be expensive and need to specifically prepared and calibrated.
For example, the Meta Quest 2 we used to collect ground truth data costs 300 dollars, and require a wide-range scan of the nearby floor and walls for initialization.
While on the other hand, IMU sensor are relatively cheap and pervasive on smart device and provides convenient and independent tracking.
As smartwatches become pervasively accepted, they provide a convenient, ubiquitous way for arm tracking. Inertial Measurement Unit (IMU) sensors (i.e., gyroscope, accelerometer, and magnetometer) in smartwatches measure and track the orientation and location of the user’s wrist.
The only condition that an IMU-based system requires may be asking the user to stand still for a few seconds (e.g., 5 seconds), so that the accelerometer and magnetometer can acquire stable reading to establish the global reference frame using gravity and north directions.

Detailed response can be found in sub-revision \ref{revision_r3_cv}

Thank you for the review.

\subsection{}
\textbf{Review:}

\textit{R4 felt that the purpose of the star sky application is unclear, and suggest evaluating/testing the application on a wristwatch, etc.}

\textbf{Revision:} 

% This issue has been partially 
In response to the concern, we conducted a new case study using smartwatch as platform in Section \ref{writing}.
% This new application is mainly based on location information, which also requires orientation estimation results (via particle filter).
Specifically, we use the smartwatch to write symbols in-air, including letters and numbers, and a triangle and a rectangle, as shown in Figure \ref{demo_gt}.
% Finally, we demonstrate the in-air writing application of \aliasSystem using smartwatch.
A potential real use case is that a user wears a smartwatch and write symbols in air to interact with smart devices.
We write 20 symbols in the corridor, where magnetic distortion affects orientation estimation, and thus affects location estimation, causing inaccurate writing traces inference.
% The symbols, which are the ground truth writing trace collected by the VR device.
% captured at a proper camera angle (20° down to the user's facing direction).
We run \aliasSystem and MUSE on the same trace using only IMU sensors' data, and show their inferred traces in Figure \ref{demo_mdr} and Figure \ref{demo_muse}.
\aliasSystem is demonstrating a better performance in tracking the writing trace of the smartwatch.

\begin{figure} [h]
    % \vspace{-3mm}
    \subfigure['A']{\includegraphics[width=0.04\linewidth]{fig/gt/1_20°_220°.png}}
    \hfill
    \subfigure['B']{\includegraphics[width=0.04\linewidth]{fig/gt/2_20°_220°.png}}
    \hfill
    \subfigure['C']{\includegraphics[width=0.04\linewidth]{fig/gt/3_20°_220°.png}}
    \hfill
    \subfigure['D']{\includegraphics[width=0.04\linewidth]{fig/gt/4_20°_220°.png}}
    \hfill
    \subfigure['E']{\includegraphics[width=0.04\linewidth]{fig/gt/5_20°_220°.png}}
    \hfill
    \subfigure['F']{\includegraphics[width=0.04\linewidth]{fig/gt/6_20°_220°.png}}
    \hfill
    \subfigure['G']{\includegraphics[width=0.04\linewidth]{fig/gt/7_20°_220°.png}}
    \hfill
    \subfigure['H']{\includegraphics[width=0.04\linewidth]{fig/gt/8_20°_220°.png}}
    \hfill
    \subfigure['I']{\includegraphics[width=0.035\linewidth]{fig/gt/9_20°_220°.png}}
    \hfill
    \subfigure['J']{\includegraphics[width=0.04\linewidth]{fig/gt/10_20°_220°.png}}
    \hfill
    \subfigure['K']{\includegraphics[width=0.04\linewidth]{fig/gt/11_20°_220°.png}}
    \hfill
    \subfigure['L']{\includegraphics[width=0.04\linewidth]{fig/gt/12_20°_220°.png}}
    \hfill
    \subfigure['M']{\includegraphics[width=0.04\linewidth]{fig/gt/13_20°_220°.png}}
    \hfill
    \subfigure['N']{\includegraphics[width=0.04\linewidth]{fig/gt/14_20°_220°.png}}
    \hfill
    \subfigure['1']{\includegraphics[width=0.04\linewidth]{fig/gt/15_20°_220°.png}}
    \hfill
    \subfigure['2']{\includegraphics[width=0.04\linewidth]{fig/gt/16_20°_220°.png}}
    \hfill
    \subfigure['3']{\includegraphics[width=0.04\linewidth]{fig/gt/17_20°_220°.png}}
    \hfill
    \subfigure['4']{\includegraphics[width=0.04\linewidth]{fig/gt/18_20°_220°.png}}
    \hfill
    \subfigure[Tri.]{\includegraphics[width=0.04\linewidth]{fig/gt/19_20°_220°.png}}
    \hfill
    \subfigure[Rect.]{\includegraphics[width=0.04\linewidth]{fig/gt/20_20°_220°.png}}
    \vspace{-3mm}
        \captionsetup{labelformat=empty}
    \caption{In-Air Writing Trace Ground Truth Collected by VR System}
    % \label{demo_gt}
    
    % \vspace{-1mm}
    % \vspace{-1mm}
    \subfigure['A']{\includegraphics[width=0.04\linewidth]{fig/mdr/1_20°_220°.png}}
    \hfill
    \subfigure['B']{\includegraphics[width=0.04\linewidth]{fig/mdr/2_20°_220°.png}}
    \hfill
    \subfigure['C']{\includegraphics[width=0.04\linewidth]{fig/mdr/3_20°_220°.png}}
    \hfill
    \subfigure['D']{\includegraphics[width=0.04\linewidth]{fig/mdr/4_20°_220°.png}}
    \hfill
    \subfigure['E']{\includegraphics[width=0.04\linewidth]{fig/mdr/5_20°_220°.png}}
    \hfill
    \subfigure['F']{\includegraphics[width=0.04\linewidth]{fig/mdr/6_20°_220°.png}}
    \hfill
    \subfigure['G']{\includegraphics[width=0.04\linewidth]{fig/mdr/7_20°_220°.png}}
    \hfill
    \subfigure['H']{\includegraphics[width=0.04\linewidth]{fig/mdr/8_20°_220°.png}}
    \hfill
    \subfigure['I']{\includegraphics[width=0.035\linewidth]{fig/mdr/9_20°_220°.png}}
    \hfill
    \subfigure['J']{\includegraphics[width=0.04\linewidth]{fig/mdr/10_20°_220°.png}}
    \hfill
    \subfigure['K']{\includegraphics[width=0.04\linewidth]{fig/mdr/11_20°_220°.png}}
    \hfill
    \subfigure['L']{\includegraphics[width=0.04\linewidth]{fig/mdr/12_20°_220°.png}}
    \hfill
    \subfigure['M']{\includegraphics[width=0.04\linewidth]{fig/mdr/13_20°_220°.png}}
    \hfill
    \subfigure['N']{\includegraphics[width=0.04\linewidth]{fig/mdr/14_20°_220°.png}}
    \hfill
    \subfigure['1']{\includegraphics[width=0.04\linewidth]{fig/mdr/15_20°_220°.png}}
    \hfill
    \subfigure['2']{\includegraphics[width=0.04\linewidth]{fig/mdr/16_20°_220°.png}}
    \hfill
    \subfigure['3']{\includegraphics[width=0.04\linewidth]{fig/mdr/17_20°_220°.png}}
    \hfill
    \subfigure['4']{\includegraphics[width=0.04\linewidth]{fig/mdr/18_20°_220°.png}}
    \hfill
    \subfigure[Tri.]{\includegraphics[width=0.04\linewidth]{fig/mdr/19_20°_220°.png}}
    \hfill
    \subfigure[Rect.]{\includegraphics[width=0.04\linewidth]{fig/mdr/20_20°_220°.png}}
    \vspace{-3mm}
        \captionsetup{labelformat=empty}
    \caption{In-Air Writing Trace Inferred by \aliasSystem}
    % \label{demo_mdr}
    
    % \vspace{-1mm}
    \vspace{1mm}
    \subfigure['A']{\includegraphics[width=0.04\linewidth]{fig/muse/1_20°_220°.png}}
    \hfill
    \subfigure['B']{\includegraphics[width=0.04\linewidth]{fig/muse/2_20°_220°.png}}
    \hfill
    \subfigure['C']{\includegraphics[width=0.04\linewidth]{fig/muse/3_20°_220°.png}}
    \hfill
    \subfigure['D']{\includegraphics[width=0.04\linewidth]{fig/muse/4_20°_220°.png}}
    \hfill
    \subfigure['E']{\includegraphics[width=0.04\linewidth]{fig/muse/5_20°_220°.png}}
    \hfill
    \subfigure['F']{\includegraphics[width=0.04\linewidth]{fig/muse/6_20°_220°.png}}
    \hfill
    \subfigure['G']{\includegraphics[width=0.04\linewidth]{fig/muse/7_20°_220°.png}}
    \hfill
    \subfigure['H']{\includegraphics[width=0.04\linewidth]{fig/muse/8_20°_220°.png}}
    \hfill
    \subfigure['I']{\includegraphics[width=0.035\linewidth]{fig/muse/9_20°_220°.png}}
    \hfill
    \subfigure['J']{\includegraphics[width=0.04\linewidth]{fig/muse/10_20°_220°.png}}
    \hfill
    \subfigure['K']{\includegraphics[width=0.04\linewidth]{fig/muse/11_20°_220°.png}}
    \hfill
    \subfigure['L']{\includegraphics[width=0.04\linewidth]{fig/muse/12_20°_220°.png}}
    \hfill
    \subfigure['M']{\includegraphics[width=0.04\linewidth]{fig/muse/13_20°_220°.png}}
    \hfill
    \subfigure['N']{\includegraphics[width=0.04\linewidth]{fig/muse/14_20°_220°.png}}
    \hfill
    \subfigure['1']{\includegraphics[width=0.04\linewidth]{fig/muse/15_20°_220°.png}}
    \hfill
    \subfigure['2']{\includegraphics[width=0.04\linewidth]{fig/muse/16_20°_220°.png}}
    \hfill
    \subfigure['3']{\includegraphics[width=0.04\linewidth]{fig/muse/17_20°_220°.png}}
    \hfill
    \subfigure['4']{\includegraphics[width=0.04\linewidth]{fig/muse/18_20°_220°.png}}
    \hfill
    \subfigure[Tri.]{\includegraphics[width=0.04\linewidth]{fig/muse/19_20°_220°.png}}
    \hfill
    \subfigure[Rect.]{\includegraphics[width=0.04\linewidth]{fig/muse/20_20°_220°.png}}
    \vspace{-3mm}
     \captionsetup{labelformat=empty}
    \caption{In-Air Writing Trace Inferred by MUSE}
    % \label{demo_muse}
\end{figure}

Statistically, the average orientation and location error during the writing are 8.27° and 0.056m for \aliasSystem, and for MUSE, 22.41° and 0.112m, as their CDFs shown in Figure \ref{fig_demo_ori} and Figure \ref{fig_demo_loc}.
We then use the popular LPIPS (Learned Perceptual Image Patch Similarity) metric \cite{Zhang_2018_CVPR} to evaluate the similarity between the inferred writing traces and the ground truth traces.
The LPIPS metric is designed to be more aligned with human perception compared to traditional metrics like PSNR (Peak Signal-to-Noise Ratio) and SSIM (Structural Similarity Index).
Lower LPIPS values indicate better perceptual similarity between images. 
Figure \ref{lpips} shows the CDFs of the LPIPS of \aliasSystem and MUSE, both compared to the ground truth traces.
We can see that the LPIPS of \aliasSystem (with an average of 0.1216) is smaller than MUSE (with an average of 0.2461), which demonstrates that \aliasSystem can better track the smartwatch using IMU sensors, and provide more robust support for indoor smart applications.

Detailed response can be found in sub-revision \ref{revision_case_2}

Thank you for the review.

\begin{figure} [H]
    \vspace{-1mm}
    \begin{minipage}[t]{0.28\linewidth}
        \hspace{-0.1cm}
        \centering
        % \vspace{-2cm}
        \includegraphics[width=1\linewidth]{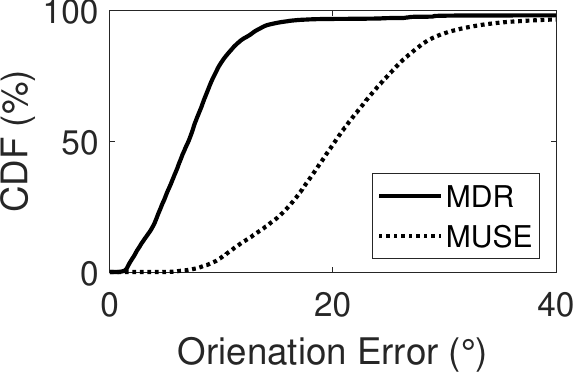}
        % \captionsetup{labelformat=empty}
        \vspace{-7mm}
        \captionsetup{labelformat=empty}
       \caption{\small CDF of orientation estimation error during in-air writing.}
        % \label{fig_demo_ori}
    \end{minipage}
    \hfill
    \begin{minipage}[t]{0.28\linewidth}
        \hspace{-0.1cm}
        \centering
        % \vspace{-2cm}
        \includegraphics[width=1\linewidth]{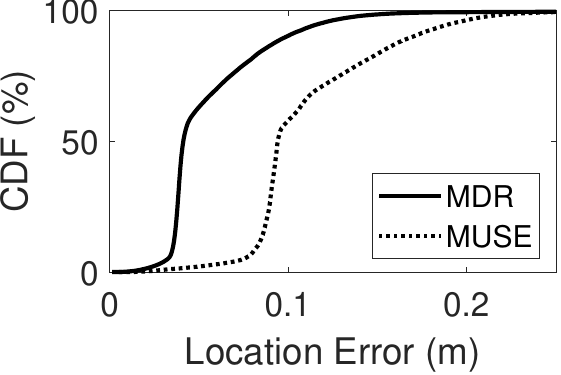}
        % \captionsetup{labelformat=empty}
        \vspace{-7mm}
        \captionsetup{labelformat=empty}
       \caption{\small CDF of location estimation error during in-air writing.}
        % \label{fig_demo_loc}
    \end{minipage}
    \hfill
    \begin{minipage}[t]{0.36\linewidth}
        \hspace{-0.1cm}
        \centering
        % \vspace{-2cm}
        \includegraphics[width=1\linewidth]{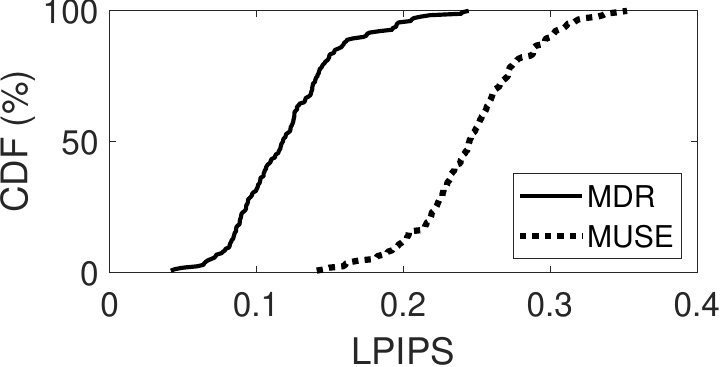}
        % \captionsetup{labelformat=empty}
        \vspace{-7mm}
        \captionsetup{labelformat=empty}
       \caption{\small CDF of LPIPS of writing traces compared to ground truth traces.}
        % \label{lpips}
    \end{minipage}
    \vspace{-1mm}
\end{figure}

\subsection{}
\textbf{Review:}
\textit{3. R3 felt that the data collection in this paper's experiments was not convincing, and the current experiments do not clearly show the robustness of the proposed method. Thus, the authors are suggested to clarify the issue about the data collection and show additional experimental results related to robustness.}

\textbf{Revision:} 

\subsubsection{Data collection}

% R3 stated: \textit{'In particular, it is unclear how the drawn lines and letters correlate to the targeted applications. 
% This relates to the aforementioned motivation problem. 
% For example, drawing letters can be done in seconds which may not be impacted by magnetic field distortion.'}

According to our best understanding, the concern seems to be: since drawing letters can be done in seconds, thus it may not be impacted by magnetic field distortion.

First, \textit{'drawing letters can be done in seconds'} is true, but the application would still be at the mercy of magnetic distortion if it is not properly addressed.
That is because magnetic distortion mainly relates to location, rather than time, as introduced in Section \ref{stability} and Section \ref{spatial corr}.
Experiments shows that the magnetic field is temporally stable in Figure \ref{temporal}, but instead, changes its direction (if distorted) as location varies, shown in Figure \ref{spatial}.
Therefore, as a letter is drawn by a user wearing a smartwatch, the smartwatch would cover a relatively long distance (e.g., 0.5m to 1m), which according to Figure \ref{spatial}, could induce the affect of magnetic distortion, making the magnetometer \textit{'point to different directions at different locations'} (Paragraph 2, Introduction).
The arm motions in our collection data typically reach the distance span of 0.6m, and 1.1m for Z-axis (the up and down direction) specifically.
Therefore the collected motion data will take in the influence from magnetic distortion, which then requires our system design \aliasSystem to solve the problem.

\begin{figure}[h]
    \vspace{-1mm}
    \hfill
    \begin{minipage}[t]{0.25\linewidth}
        \centering
        \includegraphics[width=\linewidth]{fig/mobi_chrono.pdf}
         \vspace{-7mm}
     \captionsetup{labelformat=empty}
        \caption{Temporal stability of the magnetic field.}
        % \vspace{0cm}
        % \label{temporal}
    \end{minipage}
    \hfill
    \begin{minipage}[t]{0.23\linewidth}
        \centering
        \includegraphics[width=\linewidth]{fig/sensys_spatial.pdf}
         \vspace{-7mm}
     \captionsetup{labelformat=empty}
        \caption{Spatial correlation of the magnetic field.}
        % \vspace{0cm}
        % \label{spatial}
    \end{minipage}
    \hfill
    \vspace{-4mm}
\end{figure}

Second, drawing lines and letters are basic forms of interaction with smart devices.
The data collection also include many other forms like pointing directions and exercising.
Additionally, as we stated in Section \ref{data}, to better simulate daily arm movement, we allow the users to perform the above activities in any order they want.
Users may sometimes perform customized arm motion, which is also recorded in the data traces. The data collection should be complex enough to represent real use case with various linear and angular acceleration patterns.
Adding on the different places with different magnetic nature, in which we collect data, the data set thus also includes vast range of magnetic variation patterns.

Detailed response can be found in sub-revision \ref{revision_r3_data}

\subsubsection{Robustness}

Experimental results on the robustness of the system can be found in Section \ref{DBeval}.
To clarify the concerns, we updated Section \ref{secExperimentSetting} and \ref{DBeval} with more detailed explanation.

For the issue itself, in Section \ref{stability}, we conducted experiments to show that magnetic distortion pattern is stable.
On the other hand, in Section \ref{DBeval}, evaluation shows that the database takes 5 minutes to built itself to a decent size and accuracy.
Taking the two factors above and put in another way, given that the time for database build-up is short, we can assume there will be no change in the pattern of magnetic distortion during the build up of \aliasSystem.

Second, as for the issue of location changes of appliances (R3's concern), \aliasSystem can solve this issue as it auto-adapts to new scenarios. It constructs and updates its own database via utilizing estimated orientation and location.

% in the 4-th paragraph in Introduction Section, we first briefly introduced the auto-database-construction mechanism of \aliasSystem: 
% \textit{'Automatic Database Construction. Database preparation can be difficult, as MDR requires the magnetic field direction measurement at every location. To cancel that overhead and auto-adapt to new scenarios, MDR constructs and updates its own database via utilizing estimated orientation and location.'}

In Section \ref{selfDB}, we introduce the Automatic and Adaptive Database Updating.
MDR uses estimated orientation and location, along with the magnetometer reading 
to automatically build and update the database.
For any new scenario, MDR relies on automatic updating to explore and adapt to it, without any pre-modelling (Section \ref{workflow}). 
Section \ref{DBeval} also verifies the efficiency and accuracy of the database auto-construction with experimental results.

\begin{figure}[H]
    % \vspace{-0.2cm}
    \hfill
    \begin{minipage}[t]{0.26\linewidth}
        \centering
        % \vspace{-0.1cm}
        \includegraphics[width=1\linewidth]{fig/sensys_db_during_build_up_1.pdf}
        \vspace{-7mm}
        \captionsetup{labelformat=empty}
        \caption{Database accuracy and database size during self-construction.}
        % \vspace{-0.5cm}
        % \label{build up}
    \end{minipage}
    \hfill
    \begin{minipage}[t]{0.26\linewidth}
        \centering
        % \vspace{-0.1cm}
        \includegraphics[width=1\linewidth]{fig/sensys_db_during_build_up_2.pdf}
        \vspace{-7mm}
        \captionsetup{labelformat=empty}
        \caption{Database accuracy and visits per voxel during self-construction.}
        % \vspace{-0.5cm}
        % \label{build up 2}
    \end{minipage}
    \hfill
    \vspace{-2mm}
\end{figure}
% With this mechanism

% In answering the question of previous reviewers on how our system generates to new scenarios and location changes, we added Section \ref{sec_app_flow}, where we stated that:
% \textit{'An empty database will be initialized. After initialization, orientation estimation algorithm starts working, along with the database performing ’Query’ and ’Update’, so that it can construct itself based on sensor measurements. When the user ends the application, MDR does not need to save the database, but instead, builds a new one next time.'}

In conclusion, \aliasSystem does not require any beforehand-information, such as pre-scanning or historical database, and regards all deployments as new scenarios.
It starts from scratch to explore the new location, and is able to build a usable database for the new scenario in minutes.
After each deployment, \aliasSystem does not save the database, but discard it and builds a new one in the next new deployment.
Therefore \aliasSystem is robust when the magnetic distortion context has changed, as all experiments we conducted for \aliasSystem are regarded as new scenarios, where \aliasSystem has no access to pre-scanning or past-built databases.

To address this concern, in this revision, we have added more explanation in Section \ref{secExperimentSetting}:
\textit{
'Specifically, for all real experiments in this work, \aliasSystem has no access to any pre-scan or any information on past-built databases in the same places. 
Instead, \aliasSystem regards all scenarios as new, and has to build its own database from scratch to model the local magnetic field.'
}
Also in Section \ref{DBeval}:
\textit{'In conclusion, a database can adapt to new places with exploration of a few minutes, with adequate size and accuracy.
For new scenarios, \aliasSystem requires no pre-scanning or past database history, but instead builds a new database from scratch in a few minutes.'}

Detailed response can be found in sub-revision \ref{revision_robust}

Thank you for the review.

\subsection{}
\textbf{Review:}
\textit{4. Provide more information about the impact of the temporal aspect on the updating section of the MDR method in the discussion section (R2).}

\textbf{Revision:} 

R2's question is \textit{'Does the temporal stability affect the updating part of the MDR design? Does redesigning or reconstruction of the structure of the building have any impact on the updating section of the MDR method?'}

To better address this question, we added more explanation on this issue in Section \ref{DBeval} Database Self-Construction Efficiency.

To answer the first question, the temporal stability does not affect the updating mechanism of the database.
Instead, the temporal stability is a prerequisite of the database design, since the magnetic field and its distortion pattern can only be modelled and used as reference for future if the magnetic field is not drastically changing over time.

\begin{figure}[h]
    \begin{minipage}[t]{0.25\linewidth}
        \centering
        \includegraphics[width=\linewidth]{fig/mobi_chrono.pdf}
         \vspace{-7mm}
        \captionsetup{labelformat=empty}
        \caption{Temporal stability of the magnetic field.}
        % \vspace{0cm}
        % \label{temporal}
    \end{minipage}
\end{figure}

Therefore as we state in Section \ref{stability}, this temporal stability verifies that it is possible to model the magnetic distortion at certain location and use it to assist the algorithm in the future when the device visits the same location.
% However, we do not discuss much on extreme cases, such as drastic change in indoor magnetic environments that only happens when build structures significantly change.

Second, as for the possible case that \textit{'at some point the structure of the building might change due to the redesigning or reconstruction'}, and its impact on updating mechanism, \aliasSystem will not be significantly influenced by those situations.
\aliasSystem does not save the database after each usage, but instead always builds a new one in a new deployment.
Therefore, as long as the build reconstruction does not instantly happen while \aliasSystem is build a new database, it will not hurt \aliasSystem.
After the changes are made to the building, and not more change is to be made in the near future, if \aliasSystem is going to be deployed, it will just regard that place as a new scenario, and use the auto-updating mechanism to build a decent database in a short time.
We added more explanation on this issue in Section \ref{DBeval} Database Self-Construction Efficiency:

\textit{For new scenarios, \aliasSystem requires no pre-scanning or past database history, but instead builds a new database from scratch in a few minutes.
This can also solve the extreme case we mentioned in Section \ref{stability}, in which the building structure significantly changes.
% Since \aliasSystem does not save the database, 
As long as the environment changes do not happen during the usage of \aliasSystem, \aliasSystem will be immune.
After the changes are complete, \aliasSystem will regard it as a new scenario and adapt to it within minutes.
\aliasSystem will only fail if the magnetic environment changes constantly and significantly, which is rare in real life.}
% After the environment has changed does not change much anymore

Detailed response can be found in sub-revision \ref{revision_reconstruction}

Thank you for the review.

\subsection{}
\textbf{Review:}

\textit{5. The writing / readability should be improved (R2, R3, R4). R4 also points out a need to improve math formulas representations. Also, there is a need to explain WRF and GRF in more detail (R2), and explain the stochastic tracking aspect of MDR more clearly (R4).}

\textbf{Revision:} 

We thank the reviewers for their suggestions regarding the math presentations, circled numbers, explanation of WRF and GRF, figure grouping, figure top-alignment, missing commas and colons, and paper length.
We have made corresponding updates in the revised paper, to all these comments and suggestions.

As for the \textit{'stochastic tracking aspect'}, based on our best understanding, we assume this it refers to the particle filter for location estimation, as it is the only module in this work related to stochastic inference.

To better address this issue, we updated the corresponding paragraph in the Background Section \ref{secBackground}:
\textit{'While many studies have been done in location estimation of arm tracking \cite{cutti2008ambulatory,el2012shoulder,riaz2015motion, tautges2011motion, shen2016smartwatch, liu2019real, muse}, \aliasSystem follows the state-of-the-art arm tracking solution MUSE, and adopts the particle filter to estimate the smartwatch's location.'}

% However, we borrowed this particle filter design from previous work
Our system design, \aliasSystem, uses the same particle filter for location estimation as the previous work MUSE does, except for the improvements we made for it introduced in Section \ref{secCorrectedPF}.
% The overall stochastic location estimation idea follows MUSE: 
It mainly utilizes the restriction that the human skeleton can only reach certain locations give certain posture of the hand and wrist.
Therefore, a particle filter can randomize a number of particles onto the area of possible locations of the wrist (where also the smartwatch is), based on estimated orientation.
Additionally, using the similarity between the measured acceleration, and the acceleration calculated from the particles' trajectory, the particle filter can determine which particles are tracking the smartwatch's motion more accurately, and refine the particles in every iteration to keep tracking the smartwatch location.

As we introduced the related backgrounds of particle filter in Section \ref{secBackground}, \aliasSystem follows the state-of-the-art arm tracking solution MUSE, and adopts particle filter to estimate the device's location.
% which will be used in our database query and updating.
Due to the constrain of human skeleton, the space of possible smartwatch locations is limited for specific wrist orientations.
% In this subsection we give a brief introduction on how particle filter works.
% \textbf{particle filter Initialization:}
% We know the human wrist has limited possible positions under certain orientation, due to the limitation of human skeleton.
% This information can be modelled in a point cloud.
Particle filter randomly samples a set of particles onto the possible locations.
Based on the orientation estimation result at each time step, it samples new locations for the particles, which forms a temporal trajectory.
Based on the trajectory of particles, particle filter uses accelerometer to
% calculates the velocity, then the acceleration of each particle.
% By comparing the acceleration anticipated from the particle's trajectory and the acceleration measured by accelerometer, particle filter 
evaluate how well each particle tracks the motion.
It then discards bad particles and regenerates new particles around the survivors. 
As this process repeats, the particles are continuously refined to track the device's location.'

Detailed response can be found in sub-revision \ref{stochastic}.

Thank you again for the suggestions.
% However, worth noticing, the focus of this paper is on handling magnetic distortion in orientation estimation, while location information is needed in the database operations (query and updating).
% Therefore, we do not discuss too much on the particle filter for location estimation.
% Section \ref{secCorrectedPF} is the only sub-section where we look deep into particle filter and try to improve it for better database operations.

\section{Reviewer 4 (2AE)}

\subsection{} 
\textbf{Review:}
\textit{The key to this paper is the construction and updating of the database. I do not think that such a database-based approach is very new, but I think it is a useful idea. However, I wonder if the assumption that positional information can be estimated in units of 10cm3 is really valid in realistic applications. To be honest, the technology of location estimation with such accuracy is still being researched by the ubicomp community. In other words, the construction of the database itself is unrealistic. Also, without a specific posture, the correct position and posture cannot be obtained, and the strain estimation itself may not be possible.}

\textbf{Revision:} 

\subsubsection{Whether such a database-based approach is new} \label{revision_new_or_not}

The database design in this work is a new approach that cannot be substituted by existing solutions in the context of resisting magnetic distortion in orientation estimation (explained in Background Section \ref{related}, Magnetic Fingerprint).

To better address this concern, we first updated the relevant introduction in the Related Work Section:
\textit{'Therefore, we focus heavily on orientation error and how it flows within the system.
We design novel techniques to reduce orientation error and its impact, such as adaptive updating (to be introduced in Section \ref{adaptive_updating}) and orientation error-reduction (to be introduced in Section~\ref{boost_ori_1} and \ref{boost_ori_2}).'}

Specifically, the most related magnetic field modelling technique is the fingerprinting method for localization.
However, our database, i.e., the magnetic anchor database, stores the magnetic field direction, and is used to correct orientation estimation, while fingerprinting is used to locate devices.
Difference in their purposes leads to different technical problems:

First, the magnetic anchor database requires a higher spatial resolution than fingerprinting that usually conducts meter-level positioning (e.g., MVP \cite{wang2021mvp} locates cars with accuracy of 3.89 m), since short distance (e.g., 0.1m) can make the magnetic field direction largely vary (studied in Section \ref{spatial corr} and Figure \ref{spatial}).
High resolution requirement largely increases the database preparation overhead.
To that end, we propose a novel automatic database updating mechanism in Section \ref{db_updating} to cancel the database preparation overhead.

Second, the error sourcing in the magnetic anchor database is a novel issue to be solved, due to its unique purpose of modelling and correcting magnetic distortion in orientation estimation (discussed in detail in the beginning of Section \ref{pro}).
Specifically, building and updating a database requires two factors: location and anchor, where the location information is inferred by the particle filter and shares its error, and the magnetic anchor is calculated using estimated orientation and magnetometer readings, which is affected by orientation error.
Additionally, the database will be queried to provide distortion-correction information to assist orientation estimation, which will also contain error if the query location is wrong.
The errors in query and updating process will also have correlation as the system workflow iterates (Section \ref{workflow}).
Based on these observations and motivations, we proposed novel techniques in Section \ref{pro} to reduce errors in database operations, whose improvements are also verified with experiments and presented in Section \ref{decompose}.

\subsubsection{Whether it is valid to estimate positional information can be in units of 10cm3 (10cm, or 0.001m$^3$)} \label{10cm}

As for the error level of the \textit{'positional information'}, based on experiments, \aliasSystem has a location estimation error of 0.1083m (Evaluation on location estimation error, Section \ref{eval_loc}).
This 0.1-meter-level location accuracy is enough for magnetic distortion modelling.
As introduced in Section \ref{spatial corr} and Figure \ref{spatial}, 0.1-meter distance only results in limited angular difference in the magnetic field directions.
Therefore, even with 0.1-meter-level location error, the database is still able to model the magnetic distortion with enough accuracy.

\begin{figure}[H]
    \vspace{-1mm}
    \hfill
    \begin{minipage}[t]{0.25\linewidth}
        \centering
        \includegraphics[width=\linewidth]{fig/sensys_spatial.pdf}
         \vspace{-7mm}
        \captionsetup{labelformat=empty}
        \caption{Spatial correlation of the magnetic field.}
        % \vspace{0cm}
        % \label{spatial}
    \end{minipage}
    \hfill
    \vspace{-4mm}
\end{figure}

Additionally, the database updating mechanism makes use of the feature that one location can be visited multiple times, resulting in an aggregated datapoint based on all historical measurements, which will reduce overall noise and improve the database's accuracy overtime, as verified in Section \ref{DBeval} and Figure \ref{build up} and Figure \ref{build up 2}:

\begin{figure}[H]
    % \vspace{-0.2cm}
    \hfill
    \begin{minipage}[t]{0.26\linewidth}
        \centering
        % \vspace{-0.1cm}
        \includegraphics[width=1\linewidth]{fig/sensys_db_during_build_up_1.pdf}
        \vspace{-7mm}
        \captionsetup{labelformat=empty}
        \caption{Database accuracy and database size during self-construction.}
        % \vspace{-0.5cm}
        % \label{build up}
    \end{minipage}
    \hfill
    \begin{minipage}[t]{0.26\linewidth}
        \centering
        % \vspace{-0.1cm}
        \includegraphics[width=1\linewidth]{fig/sensys_db_during_build_up_2.pdf}
        \vspace{-7mm}
        \captionsetup{labelformat=empty}
        \caption{Database accuracy and visits per voxel during self-construction.}
        % \vspace{-0.5cm}
        % \label{build up 2}
    \end{minipage}
    \hfill
    \begin{minipage}[t]{0.19\linewidth}
        \centering
        % \vspace{-0.1cm}
        \includegraphics[width=1\linewidth]{fig/sensys_prec.pdf}
        \vspace{-7mm}
        \captionsetup{labelformat=empty}
        \caption{\aliasSystem error with different spatial resolution.}
        % \vspace{-0.5cm}
        % \label{prec}
    \end{minipage}
    \hfill
    \vspace{-2mm}
\end{figure}

We also conducted experiment with different spatial resolution of the database in Section \ref{secDatabaseResolution}, with results shown in Figure \ref{prec}, which indicates that 0.1m is the optimal database spatial resolution in current system setting.

Last, this 0.1-meter-level error is enabled by the particle filter-based stochastic location estimation frame work propose by a previous work MUSE (0.1364m location error in our experiment).
We followed MUSE's overall location estimation framework in our system design, and introduced it in Background Section \ref{particle}: Location Estimation via Particle Filter.
It mainly make use of the restrain of human skeleton to acquire possible locations with a specific posture (specifically, wrist posture, since the smartwatch is there).
It uses a particle filter to deploy particles onto the possible locations, and uses the measured acceleration to distinguish whether the particles are tracking the wrist accurately.
The particle filter then refines the particles based on their tracking accuracy in every iteration, and selects the particle with the highest accuracy as the inferred location of the wrist, and thus enables relatively accurate wrist tracking.

To better address this concern, we updated the relevant introduction in the Background Section \ref{secBackground}:
\textit{'While many studies have been done in location estimation of arm tracking \cite{cutti2008ambulatory,el2012shoulder,riaz2015motion, tautges2011motion, shen2016smartwatch, liu2019real, muse}, \aliasSystem follows the state-of-the-art arm tracking solution MUSE, and adopts the particle filter to estimate the smartwatch's location.'}

More detailed description can also be found in the revision response to sub-review \ref{stochastic}.

We thank you for the review.

\subsection{}
\textbf{Review:}
\textit{In addition, the descriptions in this paper, especially the mathematical formulas, are different from those used in general engineering papers, and I believe that they are in great need of revision. In (2), the authors seem to have included an arrow representing a vector above the anchor, but I think it is unnecessary in the first place, and I hope that the string "anchor" is not used as a variable. Normally, a variable is a single character. Similarly, in (5), x is listed, but usually a scalar for scaling a vector does not require a multiplication (x) mark.}

\textbf{Revision:} 
% Do you not fucking have better things to say? Go home.
According to your suggestion, we have changed the equations.
For Equation \ref{Fanchor} and \ref{Fupdate}, we changed $\overrightarrow{anchor}$ to $\overrightarrow{N}$, and removed the multiplication '$\times$' mark.
We also checked the other equations and we believe that they follow the practice of general engineering papers.

Thank you for the suggestion.

\subsection{}
\textbf{Review:} \label{stochastic}
\textit{This MDR is supposed to introduce stochastic tracking, but the mechanism is not specifically described, making it impossible to follow the details of the method.}

\textbf{Revision:} 

Based on our best understanding, we assume this \textit{'stochastic tracking'} refers to the particle filter for location estimation, as it is the only module in this work related to stochastic inference.
% However, we borrowed this particle filter design from previous work
Our system design, \aliasSystem, uses the same particle filter for location estimation as the previous work MUSE does, except for the improvements we made for it introduced in Section \ref{secCorrectedPF}.
% The overall stochastic location estimation idea follows MUSE: 
It mainly utilizes the restriction that the human skeleton can only reach certain locations give certain posture of the hand and wrist.
Therefore, a particle filter can randomize a number of particles onto the area of possible locations of the wrist (where also the smartwatch is), based on estimated orientation.
Additionally, using the similarity between the measured acceleration, and the acceleration calculated from the particles' trajectory, the particle filter can determine which particles are tracking the smartwatch's motion more accurately, and refine the particles in every iteration to keep tracking the smartwatch location.

As we introduced the related backgrounds of particle filter in Section \ref{secBackground}, \aliasSystem follows the state-of-the-art arm tracking solution MUSE, and adopts particle filter to estimate the device's location.
% which will be used in our database query and updating.
Due to the constrain of human skeleton, the space of possible smartwatch locations is limited for specific wrist orientations.
% In this subsection we give a brief introduction on how particle filter works.
% \textbf{particle filter Initialization:}
% We know the human wrist has limited possible positions under certain orientation, due to the limitation of human skeleton.
% This information can be modelled in a point cloud.
Particle filter randomly samples a set of particles onto the possible locations.
Based on the orientation estimation result at each time step, it samples new locations for the particles, which forms a temporal trajectory.
Based on the trajectory of particles, particle filter uses accelerometer to
% calculates the velocity, then the acceleration of each particle.
% By comparing the acceleration anticipated from the particle's trajectory and the acceleration measured by accelerometer, particle filter 
evaluate how well each particle tracks the motion.
It then discards bad particles and regenerates new particles around the survivors. 
As this process repeats, the particles are continuously refined to track the device's location.'

However, worth noticing, the focus of this paper is on handling magnetic distortion in orientation estimation, while location information is needed in the database operations (query and updating).
Therefore, we do not discuss too much on the particle filter for location estimation.
Section \ref{secCorrectedPF} is the only sub-section where we look deep into particle filter and try to improve it for better database operations.

We thank you for the review.

\subsection{}
\textbf{Review:}
\textit{The purpose of the last star skyp application is not clear. The purpose is to estimate the posture of a wristwatch, right? I didn't understand the purpose of estimating the posture of a mobile phone. In other words, it is desirable to evaluate the application on a wristwatch or on a different device used together with a wristwatch, which can be done only because of the robustness of the posture estimation of the wristwatch.}

\textbf{Revision:}  \label{revision_case_2}

Thank you for the constructive comment.
According to your suggestion, we conducted a new case study using smartwatch as platform in Section \ref{writing}.
This new application is mainly based on location information, which also requires orientation estimation results (via particle filter).
Specifically, we use the smartwatch to write symbols in-air.
% Finally, we demonstrate the in-air writing application of \aliasSystem using smartwatch.
A potential real use case is that a user wears a smartwatch and write symbols in air to interact with smart devices.
We write 20 symbols in the corridor (31° distortion), where magnetic distortion affects orientation estimation, and thus affects location estimation, causing inaccurate writing traces inference.
The symbols include letters and numbers, and a triangle and a rectangle, as shown in Figure \ref{demo_gt}, which are the ground truth writing trace collected by the VR device.
% captured at a proper camera angle (20° down to the user's facing direction).
We run \aliasSystem and MUSE on the same trace using only IMU sensors' data, and show their inferred traces in Figure \ref{demo_mdr} and Figure \ref{demo_muse}.
\aliasSystem is demonstrating a better performance in tracking the writing trace of the smartwatch.

\begin{figure} [h]
    % \vspace{-3mm}
    \subfigure['A']{\includegraphics[width=0.04\linewidth]{fig/gt/1_20°_220°.png}}
    \hfill
    \subfigure['B']{\includegraphics[width=0.04\linewidth]{fig/gt/2_20°_220°.png}}
    \hfill
    \subfigure['C']{\includegraphics[width=0.04\linewidth]{fig/gt/3_20°_220°.png}}
    \hfill
    \subfigure['D']{\includegraphics[width=0.04\linewidth]{fig/gt/4_20°_220°.png}}
    \hfill
    \subfigure['E']{\includegraphics[width=0.04\linewidth]{fig/gt/5_20°_220°.png}}
    \hfill
    \subfigure['F']{\includegraphics[width=0.04\linewidth]{fig/gt/6_20°_220°.png}}
    \hfill
    \subfigure['G']{\includegraphics[width=0.04\linewidth]{fig/gt/7_20°_220°.png}}
    \hfill
    \subfigure['H']{\includegraphics[width=0.04\linewidth]{fig/gt/8_20°_220°.png}}
    \hfill
    \subfigure['I']{\includegraphics[width=0.035\linewidth]{fig/gt/9_20°_220°.png}}
    \hfill
    \subfigure['J']{\includegraphics[width=0.04\linewidth]{fig/gt/10_20°_220°.png}}
    \hfill
    \subfigure['K']{\includegraphics[width=0.04\linewidth]{fig/gt/11_20°_220°.png}}
    \hfill
    \subfigure['L']{\includegraphics[width=0.04\linewidth]{fig/gt/12_20°_220°.png}}
    \hfill
    \subfigure['M']{\includegraphics[width=0.04\linewidth]{fig/gt/13_20°_220°.png}}
    \hfill
    \subfigure['N']{\includegraphics[width=0.04\linewidth]{fig/gt/14_20°_220°.png}}
    \hfill
    \subfigure['1']{\includegraphics[width=0.04\linewidth]{fig/gt/15_20°_220°.png}}
    \hfill
    \subfigure['2']{\includegraphics[width=0.04\linewidth]{fig/gt/16_20°_220°.png}}
    \hfill
    \subfigure['3']{\includegraphics[width=0.04\linewidth]{fig/gt/17_20°_220°.png}}
    \hfill
    \subfigure['4']{\includegraphics[width=0.04\linewidth]{fig/gt/18_20°_220°.png}}
    \hfill
    \subfigure[Tri.]{\includegraphics[width=0.04\linewidth]{fig/gt/19_20°_220°.png}}
    \hfill
    \subfigure[Rect.]{\includegraphics[width=0.04\linewidth]{fig/gt/20_20°_220°.png}}
    \vspace{-3mm}
        \captionsetup{labelformat=empty}
    \caption{In-Air Writing Trace Ground Truth Collected by VR System}
    % \label{demo_gt}
    
    % \vspace{-1mm}
    % \vspace{-1mm}
    \subfigure['A']{\includegraphics[width=0.04\linewidth]{fig/mdr/1_20°_220°.png}}
    \hfill
    \subfigure['B']{\includegraphics[width=0.04\linewidth]{fig/mdr/2_20°_220°.png}}
    \hfill
    \subfigure['C']{\includegraphics[width=0.04\linewidth]{fig/mdr/3_20°_220°.png}}
    \hfill
    \subfigure['D']{\includegraphics[width=0.04\linewidth]{fig/mdr/4_20°_220°.png}}
    \hfill
    \subfigure['E']{\includegraphics[width=0.04\linewidth]{fig/mdr/5_20°_220°.png}}
    \hfill
    \subfigure['F']{\includegraphics[width=0.04\linewidth]{fig/mdr/6_20°_220°.png}}
    \hfill
    \subfigure['G']{\includegraphics[width=0.04\linewidth]{fig/mdr/7_20°_220°.png}}
    \hfill
    \subfigure['H']{\includegraphics[width=0.04\linewidth]{fig/mdr/8_20°_220°.png}}
    \hfill
    \subfigure['I']{\includegraphics[width=0.035\linewidth]{fig/mdr/9_20°_220°.png}}
    \hfill
    \subfigure['J']{\includegraphics[width=0.04\linewidth]{fig/mdr/10_20°_220°.png}}
    \hfill
    \subfigure['K']{\includegraphics[width=0.04\linewidth]{fig/mdr/11_20°_220°.png}}
    \hfill
    \subfigure['L']{\includegraphics[width=0.04\linewidth]{fig/mdr/12_20°_220°.png}}
    \hfill
    \subfigure['M']{\includegraphics[width=0.04\linewidth]{fig/mdr/13_20°_220°.png}}
    \hfill
    \subfigure['N']{\includegraphics[width=0.04\linewidth]{fig/mdr/14_20°_220°.png}}
    \hfill
    \subfigure['1']{\includegraphics[width=0.04\linewidth]{fig/mdr/15_20°_220°.png}}
    \hfill
    \subfigure['2']{\includegraphics[width=0.04\linewidth]{fig/mdr/16_20°_220°.png}}
    \hfill
    \subfigure['3']{\includegraphics[width=0.04\linewidth]{fig/mdr/17_20°_220°.png}}
    \hfill
    \subfigure['4']{\includegraphics[width=0.04\linewidth]{fig/mdr/18_20°_220°.png}}
    \hfill
    \subfigure[Tri.]{\includegraphics[width=0.04\linewidth]{fig/mdr/19_20°_220°.png}}
    \hfill
    \subfigure[Rect.]{\includegraphics[width=0.04\linewidth]{fig/mdr/20_20°_220°.png}}
    \vspace{-3mm}
        \captionsetup{labelformat=empty}
    \caption{In-Air Writing Trace Inferred by \aliasSystem}
    % \label{demo_mdr}
    
    % \vspace{-1mm}
    \vspace{1mm}
    \subfigure['A']{\includegraphics[width=0.04\linewidth]{fig/muse/1_20°_220°.png}}
    \hfill
    \subfigure['B']{\includegraphics[width=0.04\linewidth]{fig/muse/2_20°_220°.png}}
    \hfill
    \subfigure['C']{\includegraphics[width=0.04\linewidth]{fig/muse/3_20°_220°.png}}
    \hfill
    \subfigure['D']{\includegraphics[width=0.04\linewidth]{fig/muse/4_20°_220°.png}}
    \hfill
    \subfigure['E']{\includegraphics[width=0.04\linewidth]{fig/muse/5_20°_220°.png}}
    \hfill
    \subfigure['F']{\includegraphics[width=0.04\linewidth]{fig/muse/6_20°_220°.png}}
    \hfill
    \subfigure['G']{\includegraphics[width=0.04\linewidth]{fig/muse/7_20°_220°.png}}
    \hfill
    \subfigure['H']{\includegraphics[width=0.04\linewidth]{fig/muse/8_20°_220°.png}}
    \hfill
    \subfigure['I']{\includegraphics[width=0.035\linewidth]{fig/muse/9_20°_220°.png}}
    \hfill
    \subfigure['J']{\includegraphics[width=0.04\linewidth]{fig/muse/10_20°_220°.png}}
    \hfill
    \subfigure['K']{\includegraphics[width=0.04\linewidth]{fig/muse/11_20°_220°.png}}
    \hfill
    \subfigure['L']{\includegraphics[width=0.04\linewidth]{fig/muse/12_20°_220°.png}}
    \hfill
    \subfigure['M']{\includegraphics[width=0.04\linewidth]{fig/muse/13_20°_220°.png}}
    \hfill
    \subfigure['N']{\includegraphics[width=0.04\linewidth]{fig/muse/14_20°_220°.png}}
    \hfill
    \subfigure['1']{\includegraphics[width=0.04\linewidth]{fig/muse/15_20°_220°.png}}
    \hfill
    \subfigure['2']{\includegraphics[width=0.04\linewidth]{fig/muse/16_20°_220°.png}}
    \hfill
    \subfigure['3']{\includegraphics[width=0.04\linewidth]{fig/muse/17_20°_220°.png}}
    \hfill
    \subfigure['4']{\includegraphics[width=0.04\linewidth]{fig/muse/18_20°_220°.png}}
    \hfill
    \subfigure[Tri.]{\includegraphics[width=0.04\linewidth]{fig/muse/19_20°_220°.png}}
    \hfill
    \subfigure[Rect.]{\includegraphics[width=0.04\linewidth]{fig/muse/20_20°_220°.png}}
    \vspace{-3mm}
     \captionsetup{labelformat=empty}
    \caption{In-Air Writing Trace Inferred by MUSE}
    % \label{demo_muse}
\end{figure}

% We write the symbols nine times, and acquire 180 samples.
Also statistically, the average orientation and location error during the writing are 8.27° and 0.056m for \aliasSystem, and for MUSE, 22.41° and 0.112m, as their CDFs shown in Figure \ref{fig_demo_ori} and Figure \ref{fig_demo_loc}.
We also use the popular LPIPS (Learned Perceptual Image Patch Similarity) metric \cite{Zhang_2018_CVPR} to evaluate the similarity between the inferred writing traces and the ground truth traces.
The LPIPS metric is designed to be more aligned with human perception compared to traditional metrics like PSNR (Peak Signal-to-Noise Ratio) and SSIM (Structural Similarity Index).
Lower LPIPS values indicate better perceptual similarity between images. 
Figure \ref{lpips} shows the CDFs of the LPIPS of \aliasSystem and MUSE, both compared to the ground truth traces.
We can see that the LPIPS of \aliasSystem (with an average of 0.1216) is smaller than MUSE (with an average of 0.2461), which demonstrates that \aliasSystem can better track the smartwatch using IMU sensors, and provide more robust support for indoor smart applications.

We thank you for the review.
% which are also captured at the same camera angle.
% We can see that \aliasSystem has a relatively similar trace inference, while MUSE is not able to accurately track the writing.
% This is because \aliasSystem resists magnetic distortion in the hallway and provides more accurate orientation results, which is necessary to track smartwatch location using IMU sensors.

\begin{figure} [H]
    \vspace{-1mm}
    \begin{minipage}[t]{0.28\linewidth}
        \hspace{-0.1cm}
        \centering
        % \vspace{-2cm}
        \includegraphics[width=1\linewidth]{fig/IMWUT_demo_ori.pdf}
        % \captionsetup{labelformat=empty}
        \vspace{-7mm}
        \captionsetup{labelformat=empty}
       \caption{\small CDF of orientation estimation error during in-air writing.}
        % \label{fig_demo_ori}
    \end{minipage}
    \hfill
    \begin{minipage}[t]{0.28\linewidth}
        \hspace{-0.1cm}
        \centering
        % \vspace{-2cm}
        \includegraphics[width=1\linewidth]{fig/IMWUT_demo_loc.pdf}
        % \captionsetup{labelformat=empty}
        \vspace{-7mm}
        \captionsetup{labelformat=empty}
       \caption{\small CDF of location estimation error during in-air writing.}
        % \label{fig_demo_loc}
    \end{minipage}
    \hfill
    \begin{minipage}[t]{0.36\linewidth}
        \hspace{-0.1cm}
        \centering
        % \vspace{-2cm}
        \includegraphics[width=1\linewidth]{fig/IMWUT_demo.pdf}
        % \captionsetup{labelformat=empty}
        \vspace{-7mm}
        \captionsetup{labelformat=empty}
       \caption{\small CDF of LPIPS of writing traces compared to ground truth traces.}
        % \label{lpips}
    \end{minipage}
    \vspace{-5mm}
\end{figure}

\subsection{}
\textbf{Review:}
\textit{The number of pages seems too long, deviating from the imwut guideline of keeping it to p13-16.}

\textbf{Revision:} 

As the IMWUT author guideline suggests: \textit{'There is no page limit or word limit.  However, a paper length of approximately 8000-10000 words (13-16 pages), not including references or figures, is considered appropriate.'}.
Without figures and references, our paper length is 16 pages, and its word count is around 9975, which are within the proper range.
Our paper has a lot of figures, thus may appear to be extra-long.
A no-figure version of the paper is also attached with this revision for paper length reference.

We thank you for the review .

\section{Reviewer 2}

\subsection{}
\textbf{Review:}
\textit{(1) In the introduction section the authors mentioned; Current distortion handling methods [25-27] either reduce or avoid the usage of a magnetometer upon detecting magnetic distortion. But, in reference [26] (An adaptive orientation estimation method for magnetic and inertial sensors in the presence of magnetic disturbances) they provide a disturbance weight to their algorithm which incorporates the severity of the magnetic disturbance by providing more weights into the algorithm. With that being said;}

\textit{a. This part of the manuscript (i.e., the second paragraph of the introduction section) should be rewritten more precisely}

\textbf{Revision:} 

In repsonse to your suggestion, we added more precise description on reference \cite{fan2017adaptive} at the end of the second paragraph of Introduction:
\textit{Current distortion handling methods \cite{fan2017adaptive, ahrs, madgwick} either reduce or avoid the usage of magnetometer upon detecting magnetic distortion.
They use the intensity and angle of the magnetic field to indicate if distortion is strong, based on which they adjust the weight of magnetometer usage.
However, they partially avoid the impact of magnetic distortion, but then suffer from the absence of magnetometer calibration, thus fail when distortion is high.}

Thank you very much for the suggestion.

\subsection{} \label{26}
\textbf{Review:}
\textit{b. The authors claim that the novelty of their work is the development of the MDR method which is able to model and resist the magnetic distortion in orientation estimation. However, reference [26] also tackles the same problem with a different methodology. It would be great if the authors could provide more details about the novelty of their work.}

\textbf{Revision:} 
In the previous submission we introduced reference \cite{fan2017adaptive} and compared their strategy with our strategy in handling distortion. (Related Work Section \ref{related})
Reference \cite{fan2017adaptive} mainly decreases the weight for magnetometer as distortion rises (or we could also say 'increasing weight when distortion is absent'), thus avoiding the negative impact of magnetic distortion.
% This feature is most reveal when the distortion is high.
If distortion is high, reference \cite{fan2017adaptive} will have very low weight for magnetometer, and thus suffers from either the absence of magnetic calibration or magnetic distortion (verified in Section \ref{eval_distortion}).
On the other hand, our proposed approach, \aliasSystem, models the magnetic distortion using a magnetic anchor database, which is a major difference compared to reference \cite{fan2017adaptive}.
This extra information can help orientation estimation algorithm better resist distortion, as the database corrects the wrong anchor, so that the algorithm does not need to avoid using magnetometer for calibration, and does not face the issue of absent magnetic calibration.

To verify our speculations we also implemented reference \cite{fan2017adaptive} into a baseline algorithm \textit{AVOID} (introduced in Section \ref{baselines})
We mainly used the idea from work \cite{fan2017adaptive, ahrs}: detecting magnetic distortion and adjusting the weight of magnetometer accordingly, it anticipates the distortion intensity via observing the magnitude of magnetic field and the dip angle of the magnetic field.

    \vspace{-4mm}
    
    \begin{align} 
        \lambda_1 &= \frac{(|M-M_0)|}{M_0} \:(if\: \lambda_1>1, let\: \lambda_1=1)
        % \label{baseline1}
        \\ \vspace{-4mm}
        \lambda_2 &= \frac{|\theta_{dip}-\theta_0|}{20\degree} \:(if\: \lambda_2>1, let\: \lambda_2=1) 
        % \label{baseline2}
        \\ \vspace{-1mm}
        \lambda &=\frac{\lambda_1+\lambda_2}{2} 
        % \label{lambda}
    \end{align}

    \vspace{-2mm}
    
It uses the magnetometer to measure the magnetic field magnitude $M$, and compare it with the normal value of geological magnetic field magnitude $M_0$ (usually 45$\mu$T $\sim$ 55$\mu$T). 
It calculates the relative difference between $M$ and $M_0$ as $\lambda_1$.
Then in Equation \ref{lambda}, it transforms the magnetometer direction into GRF using estimated orientation, and then calculates angle between the magnetometer direction and the surface: $\theta_{dip}$.
It further compares the current dip angle with the normal dip angle $\theta_{0}$ ($\theta_{0}$ mainly depends on longitude and latitude), and calculates the difference $\lambda_2$ using a threshold of 20°.
Finally, it averages $\lambda_1$ and $\lambda_2$ into $\lambda$ to represent the intensity of distortion.
A ratio of $(1-\lambda)$ controls the weight of magnetometer, so that it partly avoids the negative impact of magnetic distortion.
We implement the strategy of $(1-\lambda)$ in a complementary filter to control the magnetometer weight: $k_{m}\cdot(1-\lambda)$.
Most importantly, to make direct comparison, we also share our design for improved orientation estimation introduced in Section \ref{boost_ori_1} and Section \ref{boost_ori_2} to boost its performance, so that the only difference between this custom baseline $AVOID$ and our system \aliasSystem lies in the strategy of magnetic distortion handling.
Therefore, via this comparison, we demonstrate the effectiveness of our database design.

As a result of the experiments, the overall average orientation errors are 16.42°, 29.57°,and 21.67° for \aliasSystem, MUSE, and $AVOID$, respectively.
\aliasSystem has an overall improvement of 44.47$\%$ over MUSE and 24.23$\%$ over $AVOID$.

\begin{figure}[h]
    \vspace{-1mm}
    \hfill
    \begin{minipage}[t]{0.47\linewidth}
        \centering
        \includegraphics[width=1\linewidth]{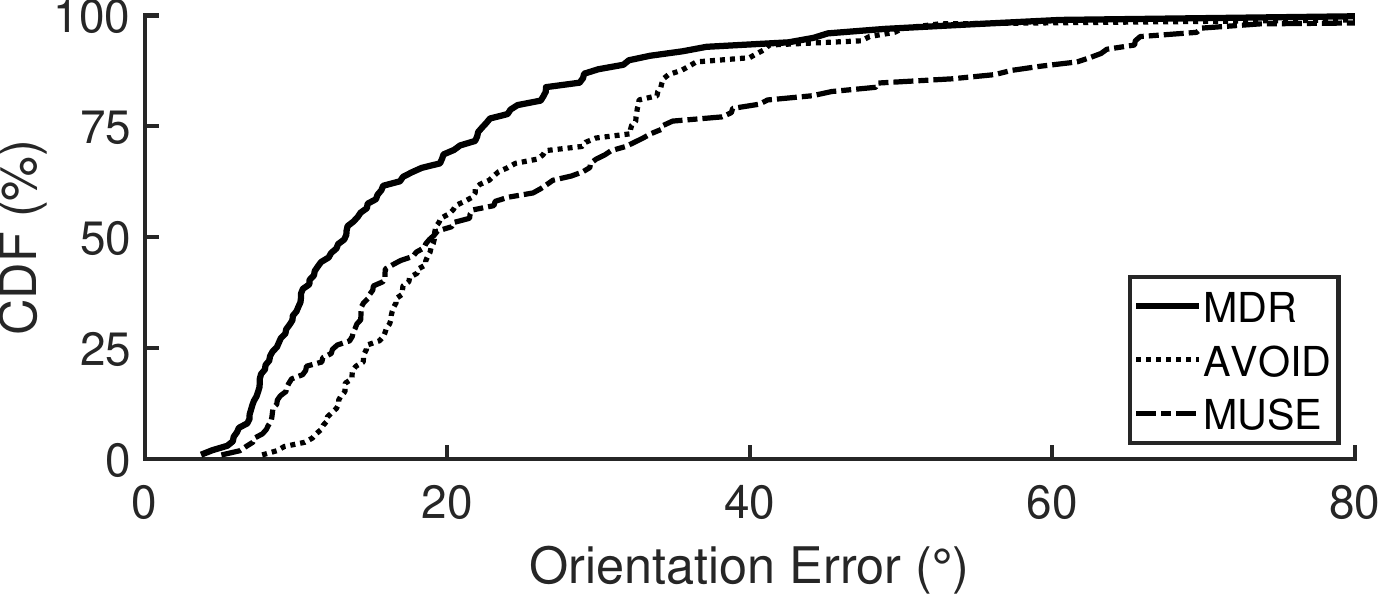}
        \vspace{-7mm}
        \captionsetup{labelformat=empty}
       \caption{Overall orientation estimation error.}
        % \label{overall}
    \end{minipage}
    \hfill
    \begin{minipage}[t]{0.43\linewidth}
        \centering
        \small
        % \vspace{-0.1cm}
        \includegraphics[width=1\linewidth]{fig/sensys_eval_dev.pdf}
        \vspace{-8mm}
        \captionsetup{labelformat=empty}
        \caption{Performance at different distortion levels.}
        % \label{result}
    \end{minipage}
    \hfill
    \vspace{-3mm}
\end{figure}

To explain this improvement, we also zoomed into the magnetic distortion resistance capability in Section \ref{eval_distortion}.
Figure \ref{result} demonstrated that reference \cite{fan2017adaptive} is not effective at resisting high distortion, while \aliasSystem maintains a relatively stable performance as distortion level increases.

We thank you for the review.

\subsection{}
\textbf{Review:} \label{revision_reconstruction}
\textit{(2) Regarding the temporal stability, Figure 4 represents the temporal stability of the magnetic field in 12 hours as proof of considering the magnetic field as a constant. Does this affect the updating part of the MDR design? This is mainly because at some point the structure of the building might change due to the redesigning or reconstruction. Then, does this have any impact on the updating section of the MDR method? If so, it would be great if the authors could provide more information about this in the discussion section.}

\textbf{Revision:} 

First, the temporal stability does not affect the updating mechanism of the database.
Instead, the temporal stability is a prerequisite of the database design, since the magnetic field and its distortion pattern can only be modelled and used as reference for future if the magnetic field is not drastically changing over time.

\begin{figure}[h]
    \begin{minipage}[t]{0.25\linewidth}
        \centering
        \includegraphics[width=\linewidth]{fig/mobi_chrono.pdf}
         \vspace{-7mm}
        \captionsetup{labelformat=empty}
        \caption{Temporal stability of the magnetic field.}
        % \vspace{0cm}
        % \label{temporal}
    \end{minipage}
\end{figure}

Therefore as we state in Section \ref{stability}, this temporal stability verifies that it is possible to model the magnetic distortion at certain location and use it to assist the algorithm in the future when the device visits the same location.
% However, we do not discuss much on extreme cases, such as drastic change in indoor magnetic environments that only happens when build structures significantly change.

Second, as for the possible case that \textit{'at some point the structure of the building might change due to the redesigning or reconstruction'}, and its impact on updating mechanism, \aliasSystem will not be significantly influenced by those situations.
\aliasSystem does not save the database after each usage, but instead always builds a new one in a new deployment.
Therefore, as long as the build reconstruction does not instantly happen while \aliasSystem is build a new database, it will not hurt \aliasSystem.
After the changes are made to the building, and not more change is to be made in the near future, if \aliasSystem is going to be deployed, it will just regard that place as a new scenario, and use the auto-updating mechanism to build a decent database in a short time.
We added more explanation on this issue in Section \ref{DBeval} Database Self-Construction Efficiency:

\textit{For new scenarios, \aliasSystem requires no pre-scanning or past database history, but instead builds a new database from scratch in a few minutes.
This can also solve the extreme case we mentioned in Section \ref{stability}, in which the building structure significantly changes.
% Since \aliasSystem does not save the database, 
As long as the environment changes do not happen during the usage of \aliasSystem, \aliasSystem will be immune.
After the changes are complete, \aliasSystem will regard it as a new scenario and adapt to it within minutes.
\aliasSystem will only fail if the magnetic environment changes frequently and significantly, which is rare in real life.}
% After the environment has changed does not change much anymore

We thank you for the review.

\subsection{}
\textbf{Review:}

\textit{(1) In the introduction section, at the end of the first paragraph, you should either explain the two defined terms in more detail, Watch’s Reference Frame (WRF) and Global Reference Frame (GRF), or provide a citation.}

\textbf{Revision:} 
In response to your suggestion, in this revision we added more description in the first paragraph of Introduction:
\textit{Orientation stands for the relationship between the Watch’s Reference Frame (WRF) and the Global Reference Frame (GRF).
WRF refers to the measurement axis of the IMU sensors, and GRF is established via regarding north as X-axis, west as Y-axis, and up as Z-axis, as shown in Figure \ref{W&G}.
Orientation of the smartwatch represented in GRF describes the relationship between the axes of WRF and GRF.}

The WRF and GRF are notions similar to the classical local reference and global reference.
WRF stands for the axes of the watch, which are exactly the axes, on which the measurements of the IMU sensors are conducted.
GRF can be different in different context, while in our implementation, we defined north as front and X-axis, and the up-direction as Z-axis.
An example of WRF and GRF is shown in Figure \ref{W&G}:

\begin{figure}[h]
    % \hfill
    % \vspace{-0.2cm}
    \begin{minipage}[t]{0.4\linewidth}
        % \vspace{-1cm}
        \centering
        \includegraphics[width=\linewidth]{fig/W&G.pdf}
        \vspace{-7mm}
        \captionsetup{labelformat=empty}
        \caption{WRF and GRF.}
        % \label{W&G}
        % \vspace{-2cm}
    \end{minipage}
    % \hfill
    % \begin{minipage}[t]{0.56\linewidth}
    %     \centering
    %     \includegraphics[width=\linewidth]{fig/scan_2.pdf}
    %     \vspace{-7mm}
    %     \caption{Magnetic distortion in a corridor.}
    %     \label{figScan}
    % \end{minipage}
    % \hfill
    % \vspace{-4mm}
\end{figure}

\subsection{}
\textbf{Review:}
\textit{(2) What is the following sentence: Limitations of Existing Solutions.
a. If it is a subsection, please provide it as 4.1.1
b. If it is just something to emphasize use a colon instead of a period at the end, like what you used for the Inertial Angular Index: on page 8 of the manuscript.}

\textbf{Revision:} 
Thank you for your review.
According to your suggestion, all similar cases have been replaced with colons or with a new subsection titles.

\section{Reviewer 3}

\subsection{}
\textbf{Review:}
\textit{* Motivations
- This is the remaining question from the last round. As the reviewers suggested, in the current revision, it is still unclear how the proposed method could be applied in practical applications. For example, while the authors added a star sky rendering scenario, it is unclear how the improvements can benefit the application itself (i.e., does it make significant changes for a star sky application using the proposed method?) Also, the star sky application is a typical "indoor" scenario as the authors primarily focus on (i.e., addressing the magnetic distortion in an indoor context). In other words, how would the proposed method enable new applications? Or make existing applications significantly different (e.g., from unable to usable?). In addition, many devices/applications such as AR/VR headsets (e.g., Meta Quest 2 as the authors used for collecting groundtruths), they already equipped with accurate and robust orientation systems such as using infrared sensing and CV methods.}

\textbf{Revision:} 

% how the improvements can benefit the application itself ????????????????????
% does it make significant changes for a star sky application using the proposed method?????????????????????
\subsubsection{How the improvements can benefit the application itself} \label{revision_r3_app}
% For \textit{'it is unclear how the improvements can benefit the application itself (i.e., does it make significant changes for a star sky application using the proposed method?)'}, 

We deploy \aliasSystem and evaluate its star sky rendering accuracy, with MUSE as comparison.
We evaluate the algorithms in this application with the metric of 'how much percent of the stars in the ground truth view port are covered by the estimated view port'.
The overall accuracy for the star sky rendering is 86.69$\%$ for \aliasSystem, and 70.92$\%$ for MUSE.

In this revision, to better explain how this improved we added the following explanation in Section \ref{eval_star}:

\textit{'Inaccurate star sky rendering leads to impaired App user experience, and may also cause misleading guidance for astronomy fans.
For example, astronomy fans usually use star sky Apps to find the approximate area of a constellation (which may not be directly found by human eyes) before precisely aligning the telescope, and thus inaccurate star sky information would decrease the efficiency of this coarse searching.'}

As conclusion, star sky App users would expect the rendering result to be as accurate as possible, so that they may efficiently search for the stars they want to observe.
Additionally, many constellations in the actual star sky are not directly visible to human eyes.
Although a telescope can clearly visualize them, the outlook of a telescope is limited (due to zoom magnification), therefore it would inefficient to use telescope to search for constellations.
To that end, users may rely on star sky Apps to coarsely find the constellations before they use the telescope for fine searching.
If the user is using a telescope indoor and observe the stars through the window, indoor magnetic distortion may affect the orientation estimation of his/her smartphone, causing the star sky App to provide inaccurate constellation information.
In this case, \aliasSystem would be able to help resist distortion and maintain efficiency for the user to search for the constellation to be observed.
% we had introduced the star sky rendering application case study in Section \ref{eval_star}, and explicitly demonstrated the direct improvement using the proposed method in Figure~\ref{star_2} and Figure~\ref{star_1}:
% \textit{'We deploy \aliasSystem and evaluate its star sky rendering accuracy, with MUSE as comparison.
% The overall accuracy for the star sky rendering is 86.69$\%$ for \aliasSystem, and 70.92$\%$ for MUSE.
% As shown in Figure~\ref{star_2}, we can see that \aliasSystem's accuracy hardly drops below 50$\%$.
% As shown in Figure~\ref{star_1}, we can also see that \aliasSystem's accuracy is almost constantly better than MUSE.'.
% Being directly deployed in the star sky rendering application, with the metric being 'how much percent of the stars can be correctly rendered', \aliasSystem has an accuracy of 86.69$\%$, while MUSE is 70.92$\%$, which is a significant change for a star sky application.

\begin{figure} [H]
    \hfill
    \begin{minipage}[t]{0.33\linewidth}
        \hspace{-0.1cm}
        \centering
        % % \vspace{-2cm}
        \includegraphics[width=1\linewidth]{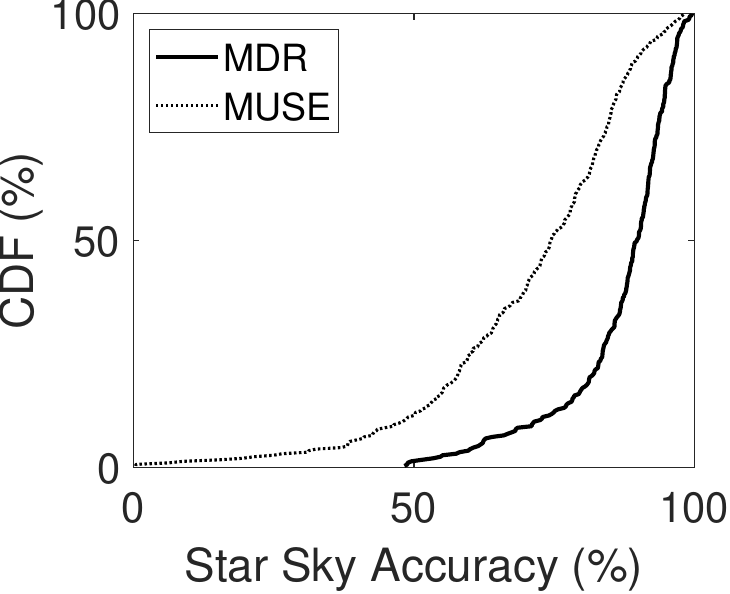}
        \captionsetup{labelformat=empty}
        % \vspace{-7mm}
       \caption{Star sky rendering accuracy CDF.}
        % \label{star_2}
    \end{minipage}
    \hfill
    \begin{minipage}[t]{0.33\linewidth}
        \centering
        % % \vspace{-0.1cm}
        \includegraphics[width=1\linewidth]{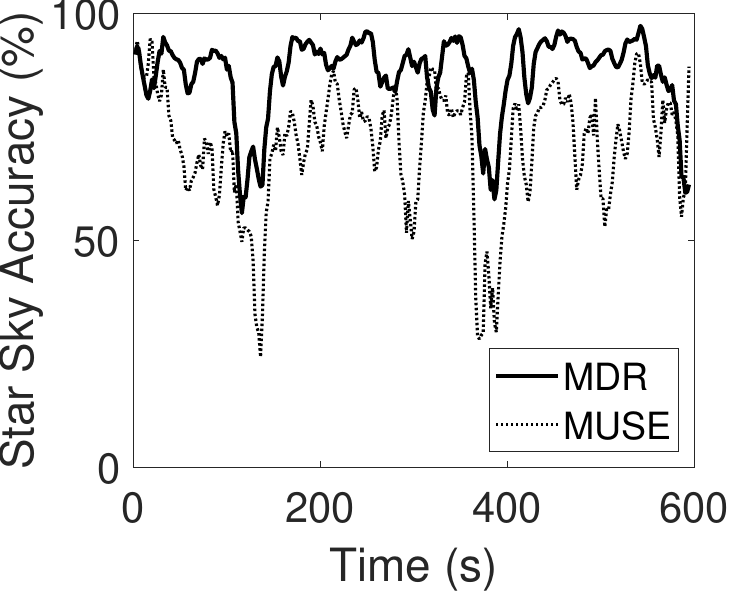}
        \captionsetup{labelformat=empty}
        % \vspace{-7mm}
        \caption{Star sky rendering accuracy over time.}
        % % \vspace{-0.5cm}
        % \label{star_1}
    \end{minipage}
    \hfill
\end{figure}

\subsubsection{How would the proposed method enable new applications?} \label{revision_r3_enable}
% For \textit{In other words, how would the proposed method enable new applications? Or make existing applications significantly different (e.g., from unable to usable?).},
\aliasSystem will enable new applications via making it possible for applications to be deployed in magnetically distorted indoor scenarios, which were not possible due to missing or incapable magnetic distortion handling mechanism.
Other than the case study on Star Sky Rendering (Section \ref{eval_star}), in this revision we also added another case study in Section \ref{writing}, which demonstrates an in-air writing application.
This new application is mainly based on location information, which also requires orientation estimation results (via particle filter).
With that as example, from the in-air writing traces inferred by MUSE, we can see it is not very capable of supporting this indoor smart application, since the letters it infers are barely recognizable (Figure \ref{demo_muse}, also listed below).
On the other hand, \aliasSystem is capable of resisting the indoor magnetic distortion and track the writing with relatively clear shape (Figure \ref{demo_mdr}).
Therefore, we could say that \aliasSystem enables smart applications in magnetically distorted scenarios, where existing solutions could not well support them.
% Magnetic distortion makes the magnetometer’s reading deviate from true north and point to different directions at different locations, resulting in large errors in orientation estimation.

% Magnetic distortion
% \aliasSystem uses a database to model 
\begin{figure} [h]
    \begin{minipage}[t]{0.45\linewidth}
        \hspace{-0.1cm}
        \centering
        % \vspace{-2cm}
        \includegraphics[width=1\linewidth]{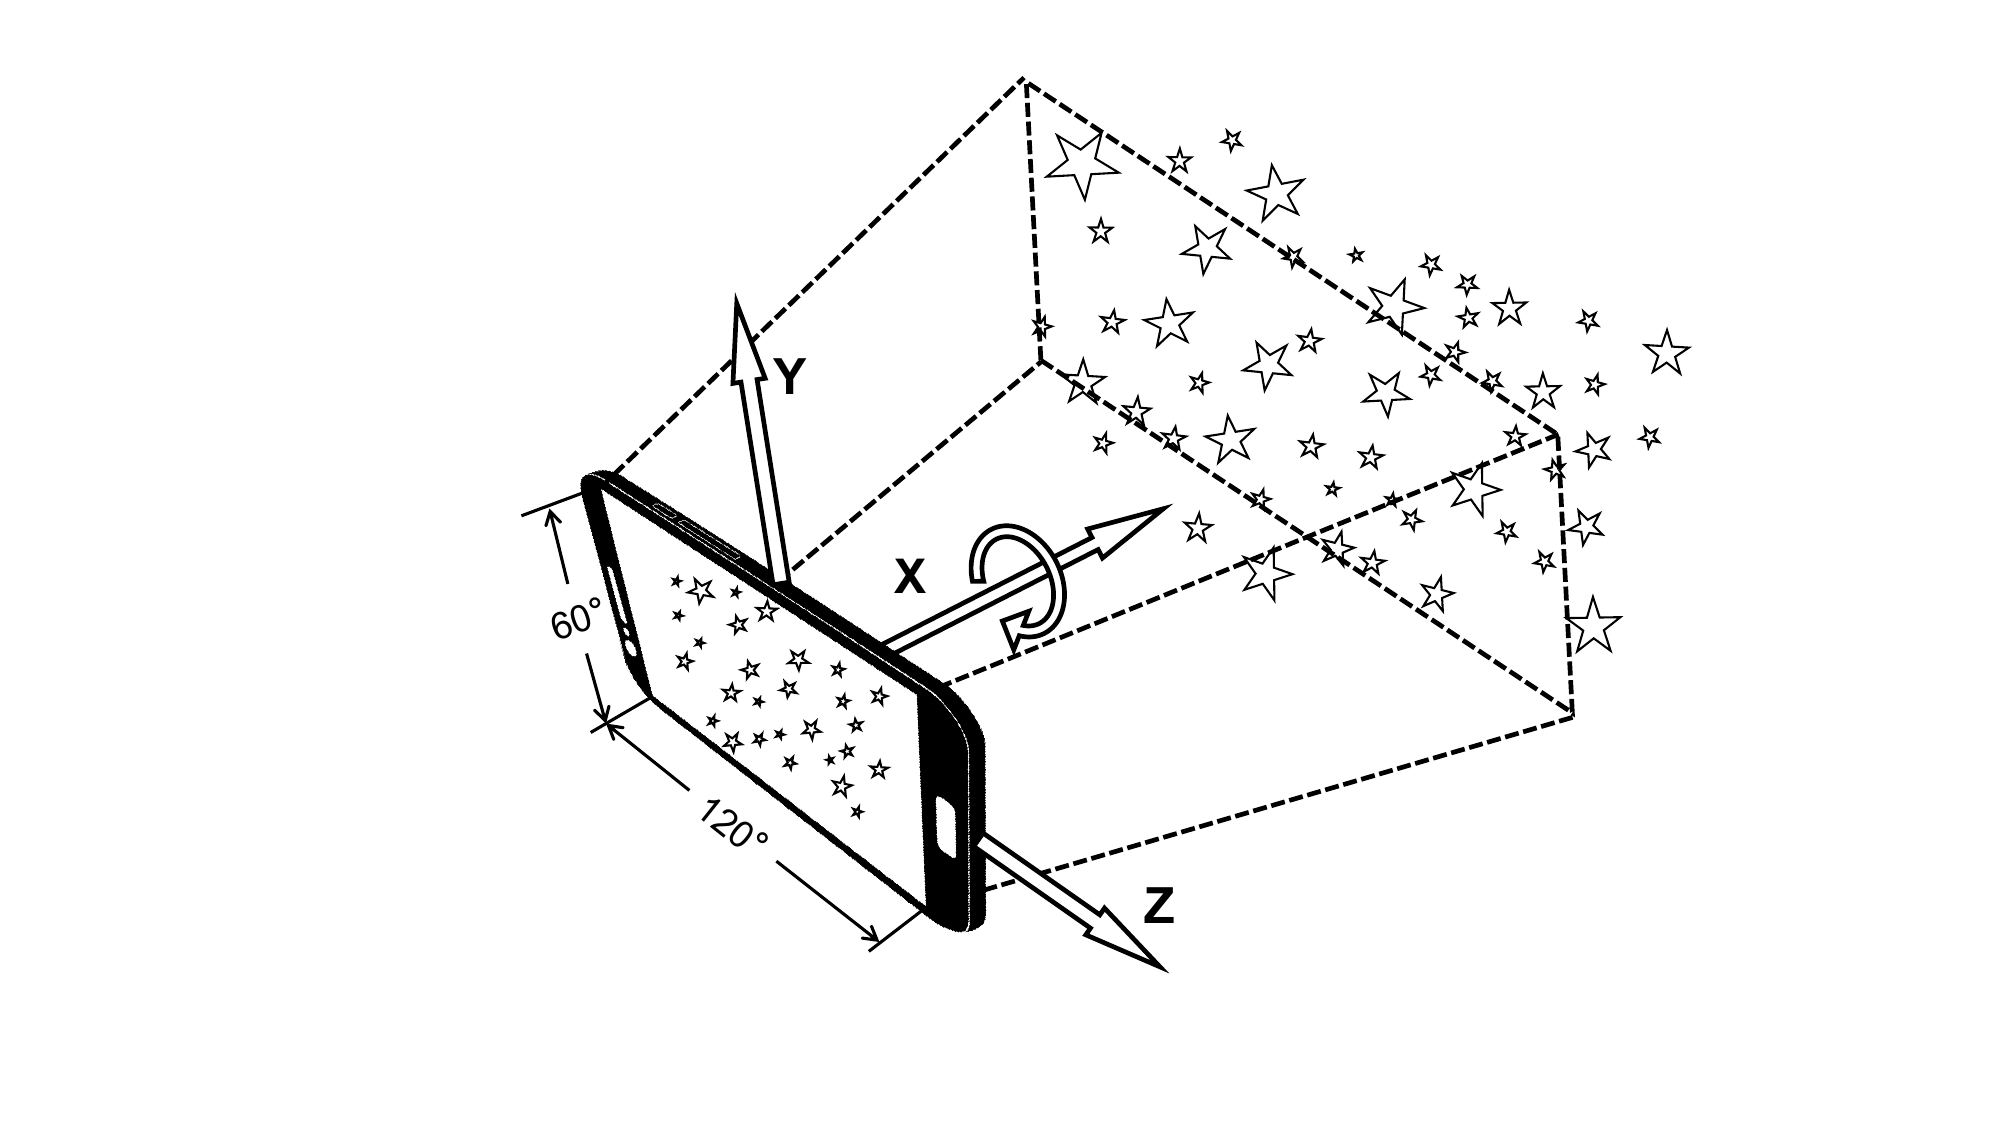}
        % \captionsetup{labelformat=empty}
        \vspace{-7mm}
        \captionsetup{labelformat=empty}
       \caption{Star sky application.}
        % \label{ubi_star_sky}
    \end{minipage}
\end{figure}

\begin{figure} [h]
    \vspace{-3mm}
    \subfigure['A']{\includegraphics[width=0.04\linewidth]{fig/gt/1_20°_220°.png}}
    \hfill
    \subfigure['B']{\includegraphics[width=0.04\linewidth]{fig/gt/2_20°_220°.png}}
    \hfill
    \subfigure['C']{\includegraphics[width=0.04\linewidth]{fig/gt/3_20°_220°.png}}
    \hfill
    \subfigure['D']{\includegraphics[width=0.04\linewidth]{fig/gt/4_20°_220°.png}}
    \hfill
    \subfigure['E']{\includegraphics[width=0.04\linewidth]{fig/gt/5_20°_220°.png}}
    \hfill
    \subfigure['F']{\includegraphics[width=0.04\linewidth]{fig/gt/6_20°_220°.png}}
    \hfill
    \subfigure['G']{\includegraphics[width=0.04\linewidth]{fig/gt/7_20°_220°.png}}
    \hfill
    \subfigure['H']{\includegraphics[width=0.04\linewidth]{fig/gt/8_20°_220°.png}}
    \hfill
    \subfigure['I']{\includegraphics[width=0.035\linewidth]{fig/gt/9_20°_220°.png}}
    \hfill
    \subfigure['J']{\includegraphics[width=0.04\linewidth]{fig/gt/10_20°_220°.png}}
    \hfill
    \subfigure['K']{\includegraphics[width=0.04\linewidth]{fig/gt/11_20°_220°.png}}
    \hfill
    \subfigure['L']{\includegraphics[width=0.04\linewidth]{fig/gt/12_20°_220°.png}}
    \hfill
    \subfigure['M']{\includegraphics[width=0.04\linewidth]{fig/gt/13_20°_220°.png}}
    \hfill
    \subfigure['N']{\includegraphics[width=0.04\linewidth]{fig/gt/14_20°_220°.png}}
    \hfill
    \subfigure['1']{\includegraphics[width=0.04\linewidth]{fig/gt/15_20°_220°.png}}
    \hfill
    \subfigure['2']{\includegraphics[width=0.04\linewidth]{fig/gt/16_20°_220°.png}}
    \hfill
    \subfigure['3']{\includegraphics[width=0.04\linewidth]{fig/gt/17_20°_220°.png}}
    \hfill
    \subfigure['4']{\includegraphics[width=0.04\linewidth]{fig/gt/18_20°_220°.png}}
    \hfill
    \subfigure[Tri.]{\includegraphics[width=0.04\linewidth]{fig/gt/19_20°_220°.png}}
    \hfill
    \subfigure[Rect.]{\includegraphics[width=0.04\linewidth]{fig/gt/20_20°_220°.png}}
    \vspace{-3mm}
        \captionsetup{labelformat=empty}
    \caption{In-Air Writing Trace Ground Truth Collected by VR System}
    % \label{demo_gt}
    
    % \vspace{-1mm}
    % \vspace{-1mm}
    \subfigure['A']{\includegraphics[width=0.04\linewidth]{fig/mdr/1_20°_220°.png}}
    \hfill
    \subfigure['B']{\includegraphics[width=0.04\linewidth]{fig/mdr/2_20°_220°.png}}
    \hfill
    \subfigure['C']{\includegraphics[width=0.04\linewidth]{fig/mdr/3_20°_220°.png}}
    \hfill
    \subfigure['D']{\includegraphics[width=0.04\linewidth]{fig/mdr/4_20°_220°.png}}
    \hfill
    \subfigure['E']{\includegraphics[width=0.04\linewidth]{fig/mdr/5_20°_220°.png}}
    \hfill
    \subfigure['F']{\includegraphics[width=0.04\linewidth]{fig/mdr/6_20°_220°.png}}
    \hfill
    \subfigure['G']{\includegraphics[width=0.04\linewidth]{fig/mdr/7_20°_220°.png}}
    \hfill
    \subfigure['H']{\includegraphics[width=0.04\linewidth]{fig/mdr/8_20°_220°.png}}
    \hfill
    \subfigure['I']{\includegraphics[width=0.035\linewidth]{fig/mdr/9_20°_220°.png}}
    \hfill
    \subfigure['J']{\includegraphics[width=0.04\linewidth]{fig/mdr/10_20°_220°.png}}
    \hfill
    \subfigure['K']{\includegraphics[width=0.04\linewidth]{fig/mdr/11_20°_220°.png}}
    \hfill
    \subfigure['L']{\includegraphics[width=0.04\linewidth]{fig/mdr/12_20°_220°.png}}
    \hfill
    \subfigure['M']{\includegraphics[width=0.04\linewidth]{fig/mdr/13_20°_220°.png}}
    \hfill
    \subfigure['N']{\includegraphics[width=0.04\linewidth]{fig/mdr/14_20°_220°.png}}
    \hfill
    \subfigure['1']{\includegraphics[width=0.04\linewidth]{fig/mdr/15_20°_220°.png}}
    \hfill
    \subfigure['2']{\includegraphics[width=0.04\linewidth]{fig/mdr/16_20°_220°.png}}
    \hfill
    \subfigure['3']{\includegraphics[width=0.04\linewidth]{fig/mdr/17_20°_220°.png}}
    \hfill
    \subfigure['4']{\includegraphics[width=0.04\linewidth]{fig/mdr/18_20°_220°.png}}
    \hfill
    \subfigure[Tri.]{\includegraphics[width=0.04\linewidth]{fig/mdr/19_20°_220°.png}}
    \hfill
    \subfigure[Rect.]{\includegraphics[width=0.04\linewidth]{fig/mdr/20_20°_220°.png}}
    \vspace{-3mm}
        \captionsetup{labelformat=empty}
    \caption{In-Air Writing Trace Inferred by \aliasSystem}
    % \label{demo_mdr}
    
    % \vspace{-1mm}
    \vspace{1mm}
    \subfigure['A']{\includegraphics[width=0.04\linewidth]{fig/muse/1_20°_220°.png}}
    \hfill
    \subfigure['B']{\includegraphics[width=0.04\linewidth]{fig/muse/2_20°_220°.png}}
    \hfill
    \subfigure['C']{\includegraphics[width=0.04\linewidth]{fig/muse/3_20°_220°.png}}
    \hfill
    \subfigure['D']{\includegraphics[width=0.04\linewidth]{fig/muse/4_20°_220°.png}}
    \hfill
    \subfigure['E']{\includegraphics[width=0.04\linewidth]{fig/muse/5_20°_220°.png}}
    \hfill
    \subfigure['F']{\includegraphics[width=0.04\linewidth]{fig/muse/6_20°_220°.png}}
    \hfill
    \subfigure['G']{\includegraphics[width=0.04\linewidth]{fig/muse/7_20°_220°.png}}
    \hfill
    \subfigure['H']{\includegraphics[width=0.04\linewidth]{fig/muse/8_20°_220°.png}}
    \hfill
    \subfigure['I']{\includegraphics[width=0.035\linewidth]{fig/muse/9_20°_220°.png}}
    \hfill
    \subfigure['J']{\includegraphics[width=0.04\linewidth]{fig/muse/10_20°_220°.png}}
    \hfill
    \subfigure['K']{\includegraphics[width=0.04\linewidth]{fig/muse/11_20°_220°.png}}
    \hfill
    \subfigure['L']{\includegraphics[width=0.04\linewidth]{fig/muse/12_20°_220°.png}}
    \hfill
    \subfigure['M']{\includegraphics[width=0.04\linewidth]{fig/muse/13_20°_220°.png}}
    \hfill
    \subfigure['N']{\includegraphics[width=0.04\linewidth]{fig/muse/14_20°_220°.png}}
    \hfill
    \subfigure['1']{\includegraphics[width=0.04\linewidth]{fig/muse/15_20°_220°.png}}
    \hfill
    \subfigure['2']{\includegraphics[width=0.04\linewidth]{fig/muse/16_20°_220°.png}}
    \hfill
    \subfigure['3']{\includegraphics[width=0.04\linewidth]{fig/muse/17_20°_220°.png}}
    \hfill
    \subfigure['4']{\includegraphics[width=0.04\linewidth]{fig/muse/18_20°_220°.png}}
    \hfill
    \subfigure[Tri.]{\includegraphics[width=0.04\linewidth]{fig/muse/19_20°_220°.png}}
    \hfill
    \subfigure[Rect.]{\includegraphics[width=0.04\linewidth]{fig/muse/20_20°_220°.png}}
    \vspace{-3mm}
     \captionsetup{labelformat=empty}
    \caption{In-Air Writing Trace Inferred by MUSE}
    % \label{demo_muse}
\end{figure}

\subsubsection{AR/VR headsets are already equipped with accurate and robust orientation systems such as using infrared sensing and CV methods.} \label{revision_r3_cv}
% For \textit{'Many devices/applications such as AR/VR headsets are already equipped with accurate and robust orientation systems such as using infrared sensing and CV methods.'},
CV-based methods requires designated hardware, e.g., depth cameras, infrared sensors and emitters, which can be expensive and need to specifically prepared and calibrated.
For example, the Meta Quest 2 we used to collect ground truth data costs 300 dollars, and require a wide-range scan of the nearby floor and walls for initialization.
While on the other hand, IMU sensor are relatively cheap and pervasive on smart device and provides convenient and independent tracking.
As smartwatches become pervasively accepted, they provide a convenient, ubiquitous way for arm tracking. Inertial Measurement Unit (IMU) sensors (i.e., gyroscope, accelerometer, and magnetometer) in smartwatches measure and track the orientation and location of the user’s wrist.
The only condition that an IMU-based system requires may be asking the user to stand still for a few seconds (e.g., 5 seconds), so that the accelerometer and magnetometer can acquire stable reading to establish the global reference frame using gravity and north directions.

To better address this question, we added in the Background section: 
\textit{'Compared to other computer vision or wireless sensing based works, IMU-based orientation estimation has an advantage of independence, as it only requires the IMU sensors on the mobile platform.
Additionally, as IMU sensors are vastly available on smart platforms, IMU based methods can also be conveniently and ubiquitously deployed.'}

We thank you for the review.

\subsection{}
\textbf{Review:} \label{revision_r3_data}
\textit{* Experiments
- While it is appreciated that the authors conducted experiments in 10 places, the data collection is not convincing (Section 7.1.3). In particular, it is unclear how the drawn lines and letters correlate to the targeted applications. This relates to the aforementioned motivation problem. For example, drawing letters can be done in seconds which may not be impacted by magnetic field distortion.}

\textbf{Revision:} 

First, \textit{'drawing letters can be done in seconds'} is true, but the application would still be at the mercy of magnetic distortion if it is not properly addressed.
That is because magnetic distortion mainly relates to location, rather than time, as introduced in Section \ref{stability} and Section \ref{spatial corr}.
Experiments shows that the magnetic field is temporally stable in Figure \ref{temporal}, but instead, changes its direction (if distorted) as location varies, shown in Figure \ref{spatial}.
Therefore, as a letter is drawn by a user wearing a smartwatch, the smartwatch would cover a relatively long distance (e.g., 0.5m to 1m), which according to Figure \ref{spatial}, could induce the affect of magnetic distortion, making the magnetometer \textit{'point to different directions at different locations'} (Paragraph 2, Introduction).
The arm motions in our collection data typically reach the distance span of 0.6m, and 1.1m for Z-axis (the up and down direction) specifically.
Therefore the collected motion data will take in the influence from magnetic distortion, which then requires our system design \aliasSystem to solve the problem.

\begin{figure}[h]
    \vspace{-1mm}
    \hfill
    \begin{minipage}[t]{0.25\linewidth}
        \centering
        \includegraphics[width=\linewidth]{fig/mobi_chrono.pdf}
         \vspace{-7mm}
     \captionsetup{labelformat=empty}
        \caption{Temporal stability of the magnetic field.}
        % \vspace{0cm}
        % \label{temporal}
    \end{minipage}
    \hfill
    \begin{minipage}[t]{0.23\linewidth}
        \centering
        \includegraphics[width=\linewidth]{fig/sensys_spatial.pdf}
         \vspace{-7mm}
     \captionsetup{labelformat=empty}
        \caption{Spatial correlation of the magnetic field.}
        % \vspace{0cm}
        % \label{spatial}
    \end{minipage}
    \hfill
    \vspace{-4mm}
\end{figure}

Second, drawing lines and letters are basic forms of interaction with smart devices.
The data collection also include many other forms like pointing directions and exercising.
Additionally, as we stated in Section \ref{data}, to better simulate daily arm movement, we allow the users to perform the above activities in any order they want.
Users may sometimes perform customized arm motion, which is also recorded in the data traces. The data collection should be complex enough to represent real use case with various linear and angular acceleration patterns.
Adding on the different places with different magnetic nature, in which we collect data, the data set thus also includes vast range of magnetic variation patterns.

We thank you for the review.

\subsection{}
\textbf{Review:}
\textit{- Technically, as previous reviewers mentioned, it is still how the authors address the varying magnetic anchor issue (Section 5.3). That is, it is unclear if the proposed method is robust when the context has been changed (such as location changes of appliances). I would suggest the authors consider conducting experiments for this point (e.g., updating Section 7.4).} \label{revision_robust}

\textbf{Revision:} 
To better address this issue, we have updated the introduction of experiment setting in   Section \ref{DBeval} with more explanation.

For the issue itself, first, to answer the question of \textit{'Whether the proposed method is robust when the context has been changed'},
in Section \ref{stability}, we conducted experiments to show that magnetic distortion pattern is stable.

\begin{figure}[h]
    \vspace{-1mm}
    \hfill
    \begin{minipage}[t]{0.25\linewidth}
        \centering
        \includegraphics[width=\linewidth]{fig/mobi_chrono.pdf}
         \vspace{-7mm}
     \captionsetup{labelformat=empty}
        \caption{Temporal stability of the magnetic field.}
        % \vspace{0cm}
        % \label{temporal}
    \end{minipage}
    \hfill
    \vspace{-4mm}
\end{figure}

On the other hand, in Section \ref{DBeval}, evaluation shows that the database takes 5 minutes to built itself to a decent size and accuracy.
Taking the two factors above and put in another way, given that the time for database build-up is short, we can assume there will be no change in the pattern of magnetic distortion during the build up of \aliasSystem.

Second, as for the issue of location changes of appliances, \aliasSystem can solve this issue as it auto-adapts to new scenarios. It constructs and updates its own database via utilizing estimated orientation and location.

% in the 4-th paragraph in Introduction Section, we first briefly introduced the auto-database-construction mechanism of \aliasSystem: 
% \textit{'Automatic Database Construction. Database preparation can be difficult, as MDR requires the magnetic field direction measurement at every location. To cancel that overhead and auto-adapt to new scenarios, MDR constructs and updates its own database via utilizing estimated orientation and location.'}

In Section \ref{selfDB}, we introduce the Automatic and Adaptive Database Updating.
MDR uses estimated orientation and location, along with the magnetometer reading 
to automatically build and update the database.
For any new scenario, MDR relies on automatic updating to explore and adapt to it, without any pre-modelling (Section \ref{workflow}). 
Section \ref{DBeval} also verifies the efficiency and accuracy of the database auto-construction with experimental results.

\begin{figure}[H]
    % \vspace{-0.2cm}
    \hfill
    \begin{minipage}[t]{0.26\linewidth}
        \centering
        % \vspace{-0.1cm}
        \includegraphics[width=1\linewidth]{fig/sensys_db_during_build_up_1.pdf}
        \vspace{-7mm}
        \captionsetup{labelformat=empty}
        \caption{Database accuracy and database size during self-construction.}
        % \vspace{-0.5cm}
        % \label{build up}
    \end{minipage}
    \hfill
    \begin{minipage}[t]{0.26\linewidth}
        \centering
        % \vspace{-0.1cm}
        \includegraphics[width=1\linewidth]{fig/sensys_db_during_build_up_2.pdf}
        \vspace{-7mm}
        \captionsetup{labelformat=empty}
        \caption{Database accuracy and visits per voxel during self-construction.}
        % \vspace{-0.5cm}
        % \label{build up 2}
    \end{minipage}
    \hfill
    \vspace{-2mm}
\end{figure}
% With this mechanism

In answering the question of previous reviewers on how our system generates to new scenarios and location changes, we added Section \ref{sec_app_flow}, where we stated that:
\textit{'An empty database will be initialized. After initialization, orientation estimation algorithm starts working, along with the database performing ’Query’ and ’Update’, so that it can construct itself based on sensor measurements. When the user ends the application, MDR does not need to save the database, but instead, builds a new one next time.'}

In conclusion, \aliasSystem does not require any beforehand-information, such as pre-scanning or historical database, and regards all deployments as new scenarios.
It starts from scratch to explore the new location, and is able to build a usable database for the new scenario in minutes.
After each deployment, \aliasSystem does not save the database, but discard it and builds a new one in the next new deployment.
Therefore \aliasSystem is robust when the magnetic distortion context has changed, as all experiments we conducted for \aliasSystem are regarded as new scenarios, where \aliasSystem has no access to pre-scanning or past-built databases.

In this revision, we have added more explanation on this matter in Section \ref{secExperimentSetting}:
\textit{
'Specifically, for all real experiments in this work, \aliasSystem has no access to any pre-scan or any information on past-built databases in the same places. 
Instead, \aliasSystem regards all scenarios as new, and has to build its own database from scratch to model the local magnetic field.'
}
Also in Section \ref{DBeval}:
\textit{'In conclusion, a database can adapt to new places with exploration of a few minutes, with adequate size and accuracy.
For new scenarios, \aliasSystem requires no pre-scanning or past database history, but instead builds a new database from scratch in a few minutes.'}

We thank you for the review.

\subsection{}
\textbf{Review:}

\textit{* Writings
- While there are some improvements compared to the last round, the writing should still be improved. In particular, the authors frequently refer to different Sections, which makes logical breaks. Hence, I would recommend the authors revise their writing with a clear logical flow, which can significantly improve the readability.}

\textbf{Revision:} 

In response to your suggestion, we reduced some cross-referring to improve the readability.
The cross-referring does not mean it is compulsory for readers to jump to the referred paragraph.
Instead, they provide a preview to certain experiment sections which will provide experimental support to the assertions or speculations.
For example, we introduced at the beginning of Section \ref{DB}: \textit{'To model magnetic distortion, \aliasSystem initializes a magnetic distortion database, which evenly divides the 3D space into voxel datapoints with a resolution of $l_{DB}$.
We set $l_{DB}=0.1m$, as to be justified in evaluation Section \ref{secDatabaseResolution}.'}
This is to make sure that readers know the important resolution setting $l_{DB}=0.1m$ is set based on experiments, and point the way to the exact experiment section if the reader is interested.
Also, to make sure that readers do not jump to the referred section every time, we stated \textit{'to be verified in Section X.Y.Z'} and \textit{'to be introduced in Section X.Y.Z'}.
We revised all cross-section references that were not in this form into this form.
We thank you for the suggestion.

The overall logical flow of this paper mainly is:
Section \ref{related} discusses existing methods on magnetic modelling, orientation estimation, and distortion handling.
It identifies the limitation of existing solutions, and highlight the potential contribution of this paper.
Section \ref{secBackground} introduces the complementary filter for orientation estimation, and the particle filter for location estimation, providing necessary notions.
Section \ref{secMotivation} presents important experimental insights on magnetic distortion, which inspires the design of \aliasSystem.
Section \ref{design} introduces the design framework of the database, which is the core design for solving the distortion issue in orientation estimation.
Section \ref{pro} discusses the error source and how it flows in the system, and correspondingly introduces three designs that reduces orientation and location errors, in order to improve database operation accuracy.
Section \ref{sec_evaluation} presents the experimental results that verifies the design of \aliasSystem and its components.
Section \ref{sec_case_study} further validates \aliasSystem on two real application cases.

\subsection{}
\textbf{Review:}
\textit{- Also, as reviewers from the previous round mentioned, the writing is still too verbose. For example, the motivation is described in Section 4, which should be clarified in the introduction and related work (i.e., pinpoint the motivation at the beginning of this paper).}

\textbf{Revision:} 
According to your suggestion, we reduced some unnecessary introductions.
We briefly introduced the motivation in the second paragraph of Introduction: \textit{'However, MUSE ignores the magnetic distortion that commonly exists in buildings, i.e., metal structures in buildings can cause the magnetic field to point to various directions.'}.
Following that we briefly introduced the magnetic distortion:
\textit{'Magnetic distortion makes the magnetometer’s reading deviate from true north and point to different directions at different locations, resulting in large errors in orientation estimation.'}.
However, Section \ref{secMotivation} Motivation is still greatly necessary, in which we present the experiments that show the temporal stability and spatial correlation of the magnetic field.
% which later support the design of \aliasSystem.
% That is the first introduction on motivation.

Additionally, the core feature of our motivation, i.e. magnetic distortion, has not been studied in depth in other existing works. 
Instead, we look deep into this issue via conducting real experiments on magnetic distortion in Section 4, which are crucial support for the design of \aliasSystem.

The related work section is meant to identify our work's difference from major existing techniques, e.g., magnetic fingerprint for localization and basic distortion handling for orientation estimation, as former reviewers questioned about why our work is needed since fingerprint already exists in localization.
Therefore we discuss the major differences between our magnetic anchor database and fingerprint in this section, which mainly are the resolution requirement and database error sourcing and handling.
Those factors are crucial to identify our work's contribution which are not achievable by existing works.

We thank you for the suggestion.

\subsection{}
\textbf{Review:}

* Minor points
\textit{- The authors should add line numbers for the manuscript so the reviewers can refer to particular contents.}

\textbf{Revision:} 
% Thank you for the review.
According to your suggestion, line numbers have been added for the manuscript.
We thank you for the suggestion.

\subsection{}
\textbf{Review:}
\textit{- The figures should be top-align by default, unless necessary.}

\textbf{Revision:} 
% We have carefully placed the figures for many times to ensure minimal distance between the figures and the paragraphs that refer to them, so that readers will not need to scroll too much to find the figures.
Thank you for the review.
According to your suggestion, we made most of the figures at the top in this revision.

\subsection{}
\textbf{Review:}
\textit{- The figures should be grouped with a more concise numbering method (refer to typical IMWUT papers, e.g., Fig. 3-5 should be a single number, while Fig. 21 shows a good example).}

\textbf{Revision:}  
Thank you for the review.
According to your suggestion, we mainly grouped the 9 pictures of the places for data collection into Figure \ref{fig_photo}, as the sub-figures share similar purpose and meaning.
% For the figures of the in-air writing traces in the new Section \ref{writing}, we also grouped the symbols.

\begin{figure} [h]
    % \vspace{-0.2cm}
    \hfill
    \subfigure[Conference Room.]{\includegraphics[width=.2\textwidth]{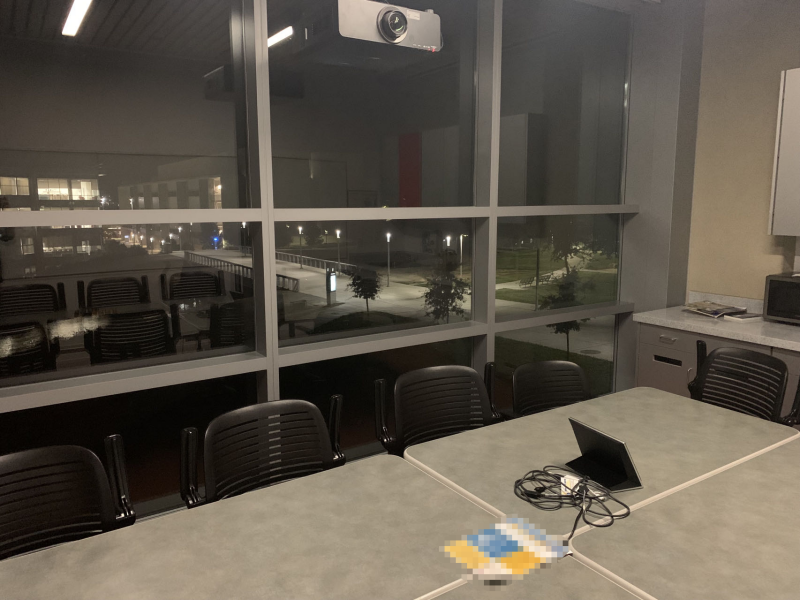}}
    \hfill
    \subfigure[Corridor.]{\includegraphics[width=.2\textwidth]{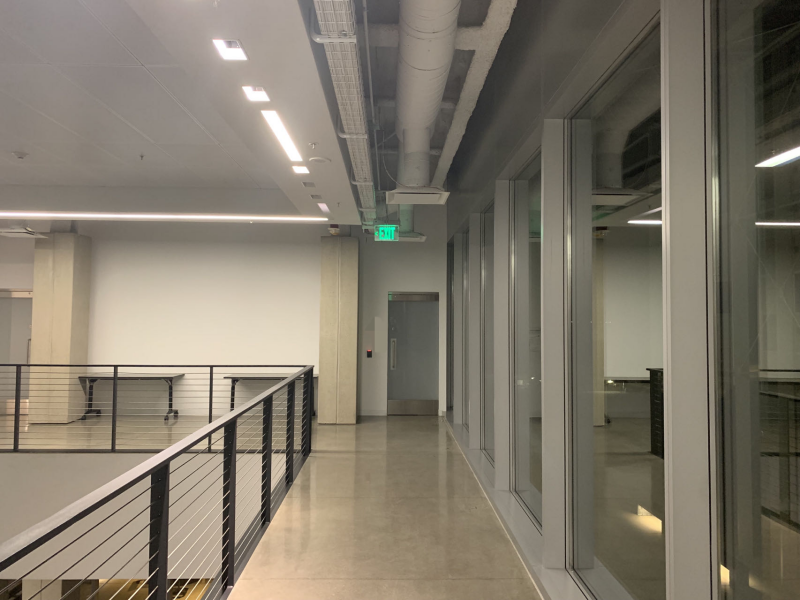}}
    \hfill
    \subfigure[House.]{\includegraphics[width=.2\textwidth]{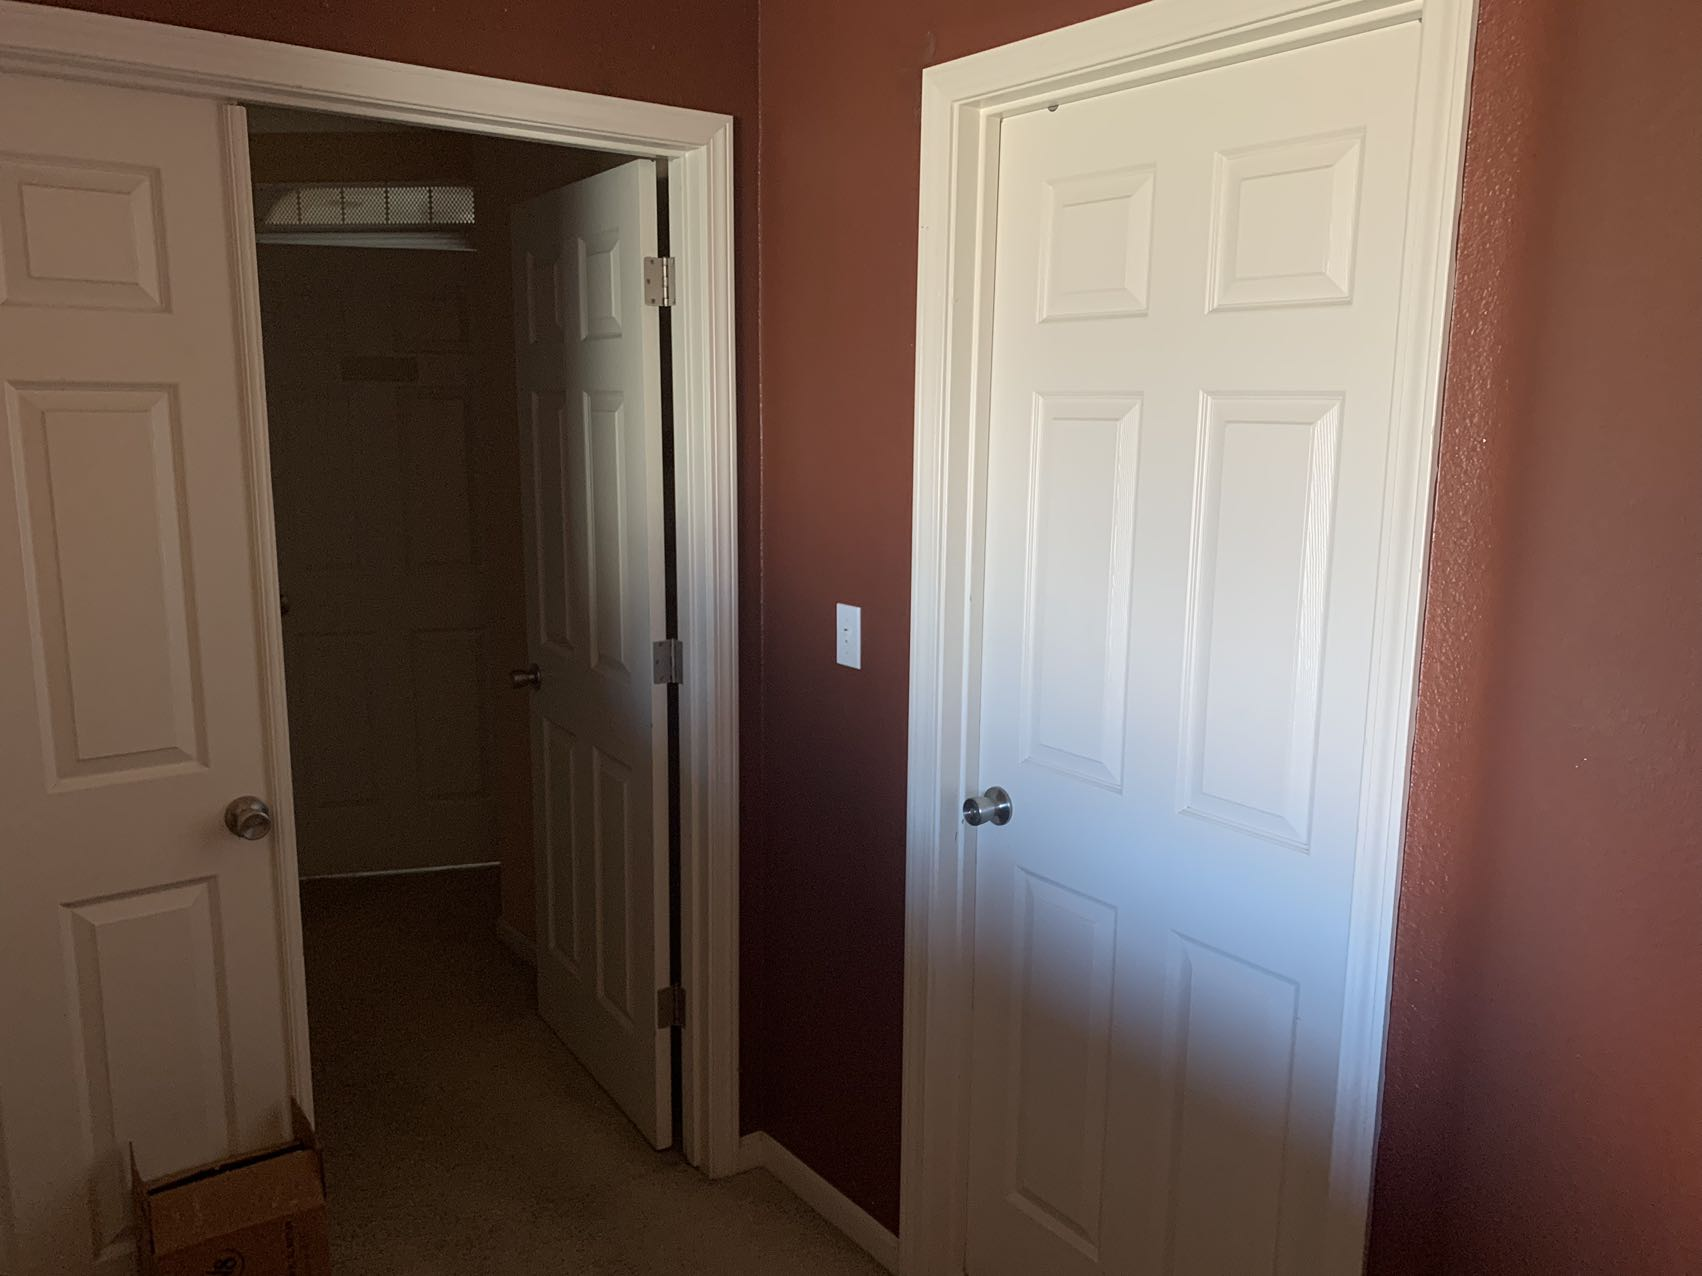}}
    \hfill
    \vspace{-2mm}
    
    \hfill
    \subfigure[Stairwell.]{\includegraphics[width=.2\textwidth]{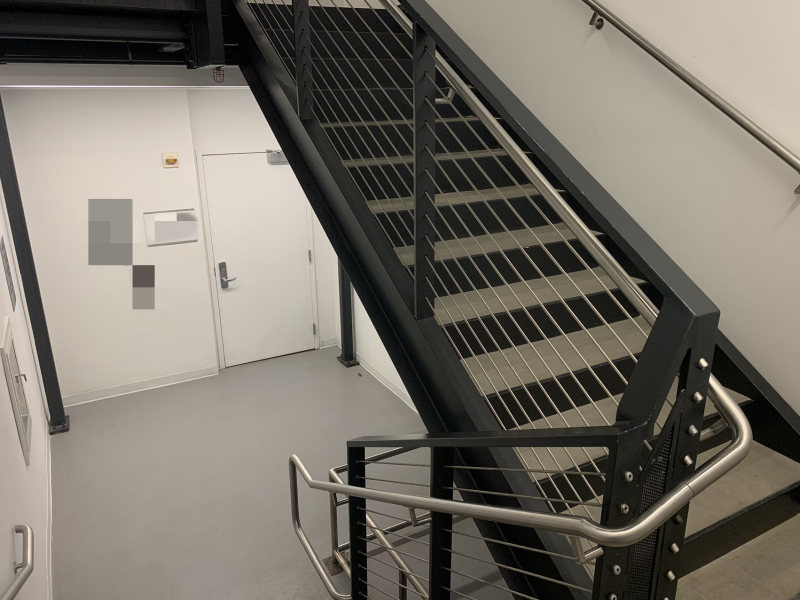}}
    \hfill
    \subfigure[Office.]{\includegraphics[width=.2\textwidth]{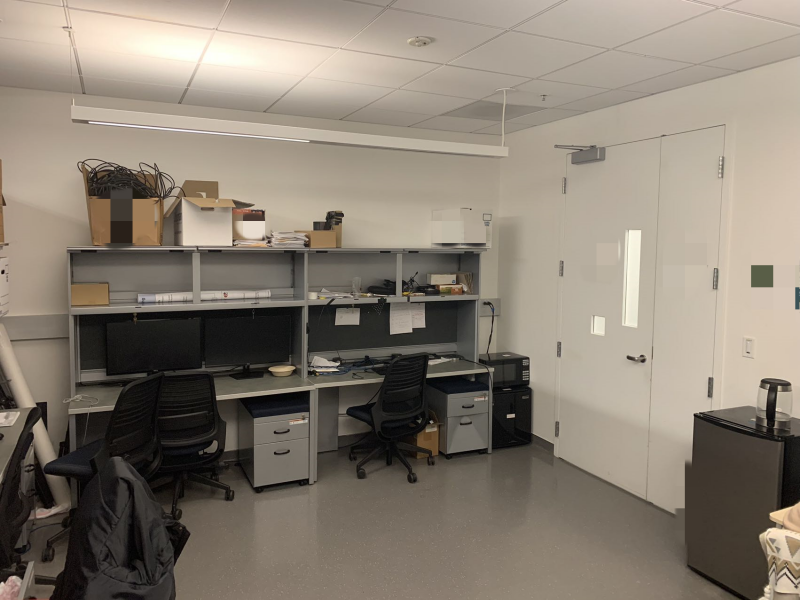}}
    \hfill
    \subfigure[Auditorium.]{\includegraphics[width=.2\textwidth]{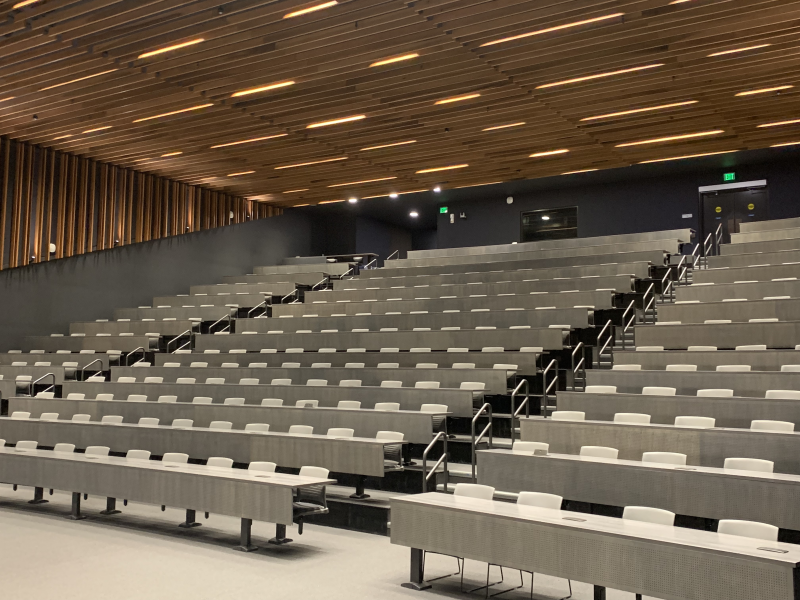}}
    \hfill
    \vspace{-2mm}
    
    \hfill
    \subfigure[Apartment 1.]{\includegraphics[width=.2\textwidth]{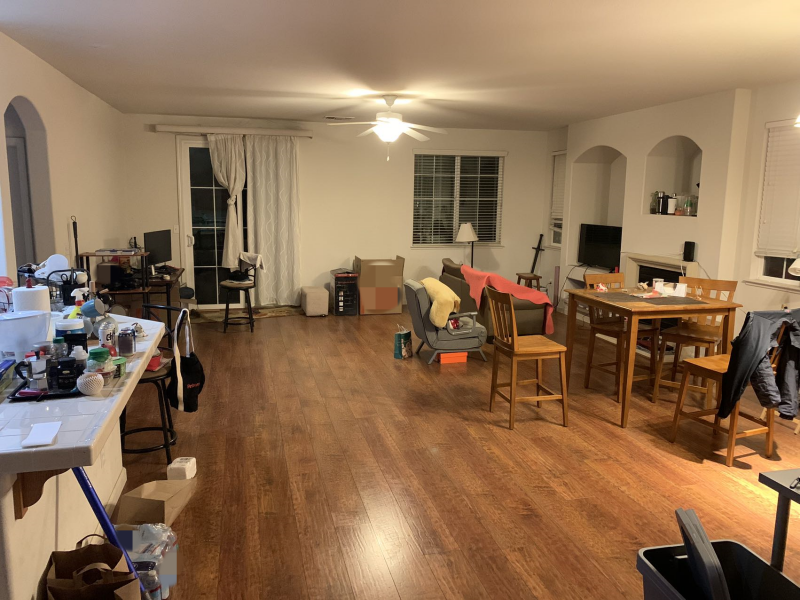}}
    \hfill
    \subfigure[Apartment 2.]{\includegraphics[width=.2\textwidth]{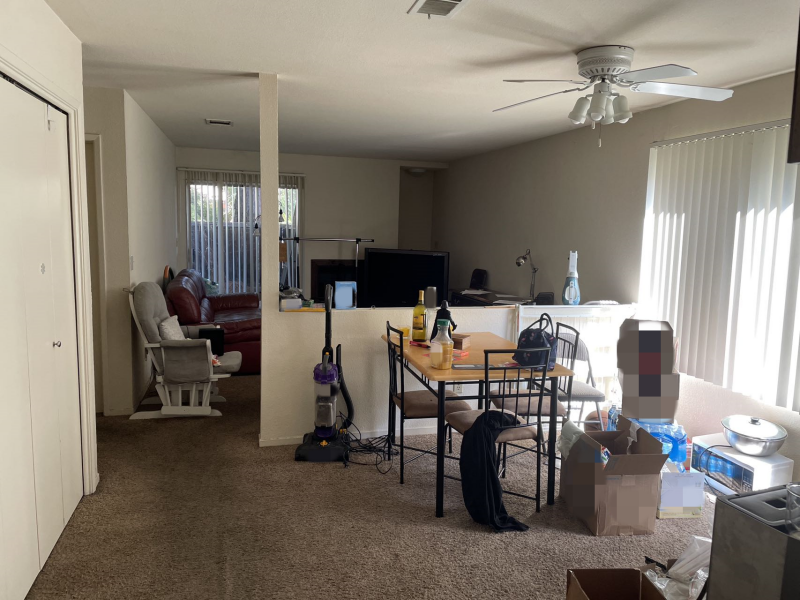}}
    \hfill
    \subfigure[Apartment 3.]{\includegraphics[width=.2\textwidth]{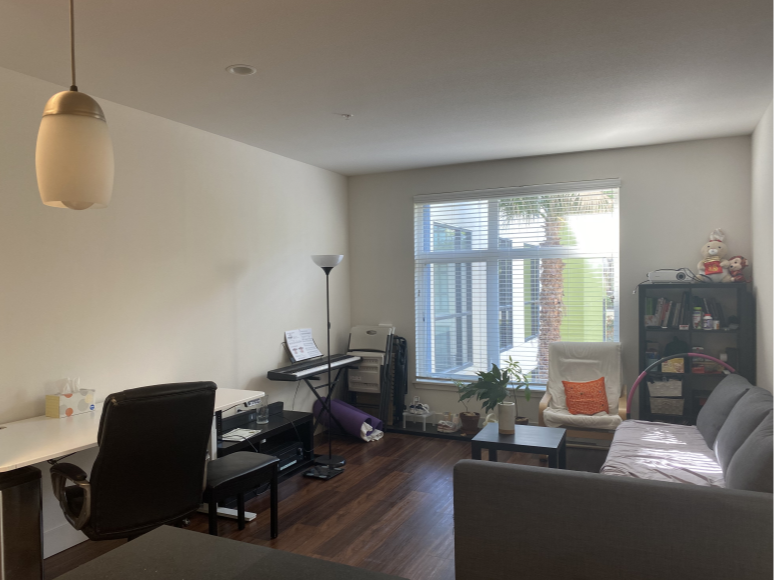}}
    \hfill
    \vspace{-3mm}
        \captionsetup{labelformat=empty}
    \caption{Pictures of Places for Data Collection and Experiments}
    % \label{fig_photo}
    \vspace{-5mm}
\end{figure}

However, other figures that are in one line usually belong to different sections, such as Figure \ref{muse_devM}, Figure \ref{temporal}, Figure \ref{spatial}.
They are positioned in on line only to save space for the paper.
As we tried very hard to group them, it would be hard to make a overall caption for the figure set that can conclude the figures' purpose and meaning.
Additionally, we try not to misguide the readers into thinking that these figures are from the same logical section.
Therefore, for those figures, we keep their current form.
We referred to other IMWUT papers \cite{figure_format, figure_format_2} on this point.

We thank you for the review.
% \begin{figure} [h]
%     % \vspace{-0.2cm}
%     \hfill
%     \subfigure[Conference Room.]{\includegraphics[width=.2\textwidth]{fig/photo_confer.png}}
%     \hfill
%     \subfigure[Corridor.]{\includegraphics[width=.2\textwidth]{fig/photo_corridor.png}}
%     \hfill
%     \subfigure[House.]{\includegraphics[width=.2\textwidth]{fig/photo_house.jpg}}
%     \hfill
%     \vspace{-2mm}
    
%     \hfill
%     \subfigure[Stairwell.]{\includegraphics[width=.2\textwidth]{fig/photo_stairwell.png}}
%     \hfill
%     \subfigure[Office.]{\includegraphics[width=.2\textwidth]{fig/photo_office.png}}
%     \hfill
%     \subfigure[Auditorium.]{\includegraphics[width=.2\textwidth]{fig/photo_audito.png}}
%     \hfill
%     \vspace{-2mm}
    
%     \hfill
%     \subfigure[Apartment 1.]{\includegraphics[width=.2\textwidth]{fig/photo_apt_1.png}}
%     \hfill
%     \subfigure[Apartment 2.]{\includegraphics[width=.2\textwidth]{fig/photo_apt2.png}}
%     \hfill
%     \subfigure[Apartment 3.]{\includegraphics[width=.2\textwidth]{fig/photo_apt_3.png}}
%     \hfill
%     \vspace{-3mm}
%     \captionsetup{labelformat=empty}
%     \caption{Pictures of Places for Data Collection and Experiments}
%     % \label{fig_photo}
%     \vspace{-5mm}
% \end{figure}

\subsection{}
\textbf{Review:}
\textit{- Irregular text should be avoided (e.g., round numbers such as \textcircled{1}
)}

\textbf{Revision:} 
In response to your suggestion, round numbers such as \textcircled{1} have been removed.
We thank you for the suggestion.

\subsection{}
\textbf{Review:}
\textit{- Missing commas after e.g. and i.e.}

\textbf{Revision:} 
According to your suggestion, all missing commas after e.g. and i.e. have been added.
We thank you for the suggestion.
